# Supplementary material for: Diaconis-Ylvisaker prior penalized likelihood for $p/n \to \kappa \in (0,1)$ logistic regression
Source: arXiv:2311.07419 source file (2026-01-06)
Supplement: Supplementary file 1 [file mDYPL-supplementary-arxiv-1.pdf]

Supplementary Material document for  
*Diaconis-Ylvisaker prior penalized likelihood for*  
 $p/n \rightarrow \kappa \in (0, 1)$  *logistic regression*

Philipp Sterzinger 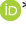\*<sup>1</sup> and Ioannis Kosmidis 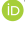†<sup>2</sup>

<sup>2</sup>Department of Statistics, London School of Economics  
London, WC2A 2AE, UK

<sup>2</sup>Department of Statistics, University of Warwick  
Coventry, CV4 7AL, UK

December 17, 2024

## Contents

|                                                                          |           |
|--------------------------------------------------------------------------|-----------|
| <b>S1 Overview</b>                                                       | <b>2</b>  |
| <b>S2 Further numerical results and simulation experiments</b>           | <b>2</b>  |
| S2.1 Signal recovery of the rescaled MDYPL estimator . . . . .           | 2         |
| S2.2 Stochastic boundedness of the MDYPL estimator . . . . .             | 3         |
| S2.3 Adjusted Z-statistics for MDYPL with intercept . . . . .            | 4         |
| S2.4 Estimates of $v$ for the simulation study of Section 5.1 . . . . .  | 7         |
| <b>A Maximum Diaconis-Ylvisaker prior penalized likelihood</b>           | <b>7</b>  |
| <b>B Proof of Theorem 3.1</b>                                            | <b>7</b>  |
| B.1 Asymptotic characterisation via stationary state evolution . . . . . | 8         |
| B.2 Proof outline for Theorem 3.1 . . . . .                              | 8         |
| B.3 Matrix-valued AMP . . . . .                                          | 9         |
| B.4 Proof of Theorem 3.1 . . . . .                                       | 11        |
| B.4.1 Target AMP recursion . . . . .                                     | 11        |
| B.4.2 Centred target AMP recursion . . . . .                             | 11        |
| B.4.3 Matrix-valued AMP-embedding . . . . .                              | 12        |
| B.4.4 A smooth approximation . . . . .                                   | 18        |
| B.4.5 Asymptotic equivalence of target and centred AMP . . . . .         | 23        |
| B.4.6 Asymptotic equivalence of AMP and MDYPL . . . . .                  | 26        |
| <b>C Proof of Theorem 3.2</b>                                            | <b>30</b> |
| <b>D Proof of Theorem 3.3</b>                                            | <b>35</b> |
| <b>E Proof of Theorem 3.4</b>                                            | <b>40</b> |

---

\*p.sterzinger@lse.ac.uk

†ioannis.kosmidis@warwick.ac.uk

## S1 Overview

This document contains further simulation results and the proofs of all results in the main text of *Diaconis-Ylvisaker prior penalized likelihood for  $p/n \rightarrow \kappa \in (0,1)$  logistic regression*. Section S2 provides another demonstration of the signal recovery, similar to Figure 1 of the main text, simulation evidence about the stochastic boundedness of  $\|\hat{\beta}^{\text{DY}}\|_2/\sqrt{n}$  for various values of  $\alpha$  following the discussion of Theorem 3.2, results on the suitability of adjusted  $Z$ -statistics for inference in support of Conjecture 6.1, and the empirical distribution of the estimator of  $v$  from the simulation study of Section 5.1. To provide context for the proofs of our results, Appendix A restates the MDYPL setting considered in the main paper. Appendices B-F contain proofs of the main results in the paper. Key lemmas are listed in the appendices of the respective proofs and minor auxiliary lemmas are listed in Appendix G.

## S2 Further numerical results and simulation experiments

### S2.1 Signal recovery of the rescaled MDYPL estimator

As an additional demonstration to Figure 1, we revisit the synthetic data example of Sur and Candès (2019, Figure 2). Specifically,  $\mathbf{x}_j \sim \mathcal{N}(\mathbf{0}_p, n^{-1}\mathbf{I}_p)$  and  $\beta_0$  consists of  $n\kappa/8$  replications of  $(-10, 10, 0, 0, 0, 0, 0)^\top$  adequately scaled to achieve  $\|\beta_0\|_2^2 = \gamma^2$  for various values of  $(\kappa, \gamma)$  and  $n = 2000$ . Figure S1 shows the MDYPL estimates and their rescaled versions  $\hat{\beta}^{\text{DY}}/\mu_*$  for various values of  $(\kappa, \gamma)$  and  $\alpha = 1/(1 + \kappa)$ . The rescaled estimates are found to recover the signal  $\beta_0$  at either side of the phase transition curve as is to be expected from (x).

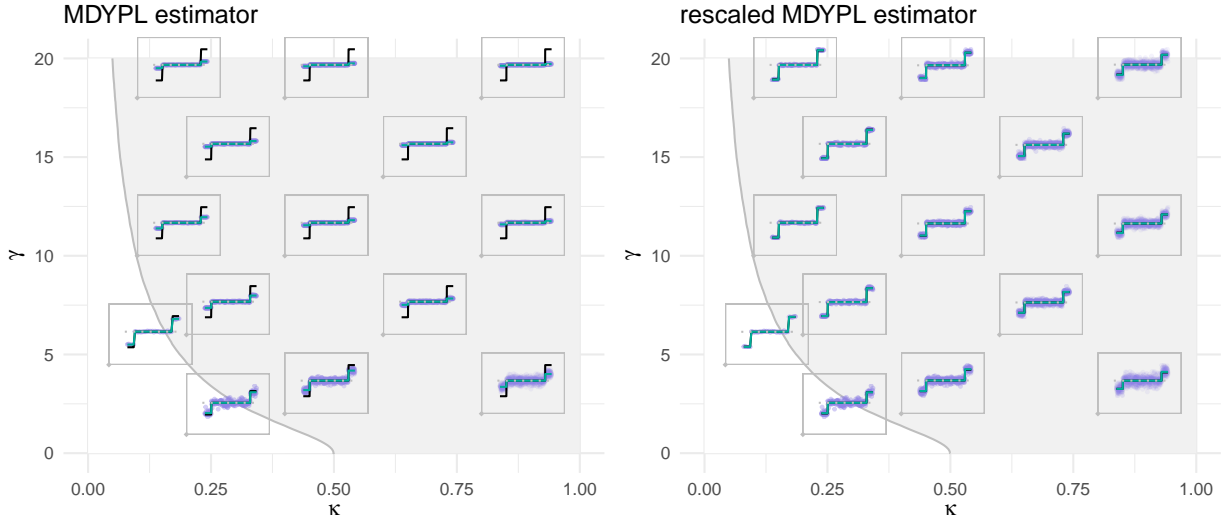

Figure S1: The MDYPL (left) and rescaled MDYPL (right) estimates for various configurations of  $(\kappa, \gamma)$  and  $\alpha = 1/(1 + \kappa)$ ,  $n = 2000$  in the setting of Figure 2 in Sur and Candès (2019). Blue markers show the average coefficient estimates over 10 independent runs while the green segments denote the signal. The white and grey areas in the background indicate where the ML estimate does or does not exist asymptotically, respectively.

## S2.2 Stochastic boundedness of the MDYPL estimator

To investigate the behaviour of the  $\ell_2$ -norm of the MDYPL-estimator, we simulate  $\|\hat{\beta}^{\text{DY}}(\alpha)\|_2/\sqrt{n}$ , for  $\alpha \in \{0.9, 0.95, 0.99, 0.99\}$  and  $\alpha = 1/(1 + \kappa)$  over a range of  $(\kappa, \gamma)$  values and  $n \in \{200, 400, \dots, 8000\}$ . The covariate matrix  $\mathbf{X}$  has i.i.d. rows  $\mathbf{x}_i \sim \mathcal{N}(\mathbf{0}_p, n^{-1}\mathbf{I}_p)$ , and the signal is the same as in Sur and Candès (2019, Figure 2) scaled to achieve the desired signal strength  $\gamma$ . For each specification of  $\alpha, \kappa, \gamma, n$ ,  $\|\hat{\beta}^{\text{DY}}(\alpha)\|_2/\sqrt{n}$  is estimated as the mean from 50 independent draws of  $\{\mathbf{y}, \mathbf{X}\}$ . The results are displayed in Figure S2 and provide no evidence that  $\|\hat{\beta}^{\text{DY}}(\alpha)\|_2/\sqrt{n}$  is not bounded in probability for all  $(\kappa, \gamma)$  ranges considered, even when there is almost no shrinkage induced by the DY prior. Hence, we believe that the threshold  $\alpha_0$  in Theorem 3.2 is an artefact of our proof strategy.

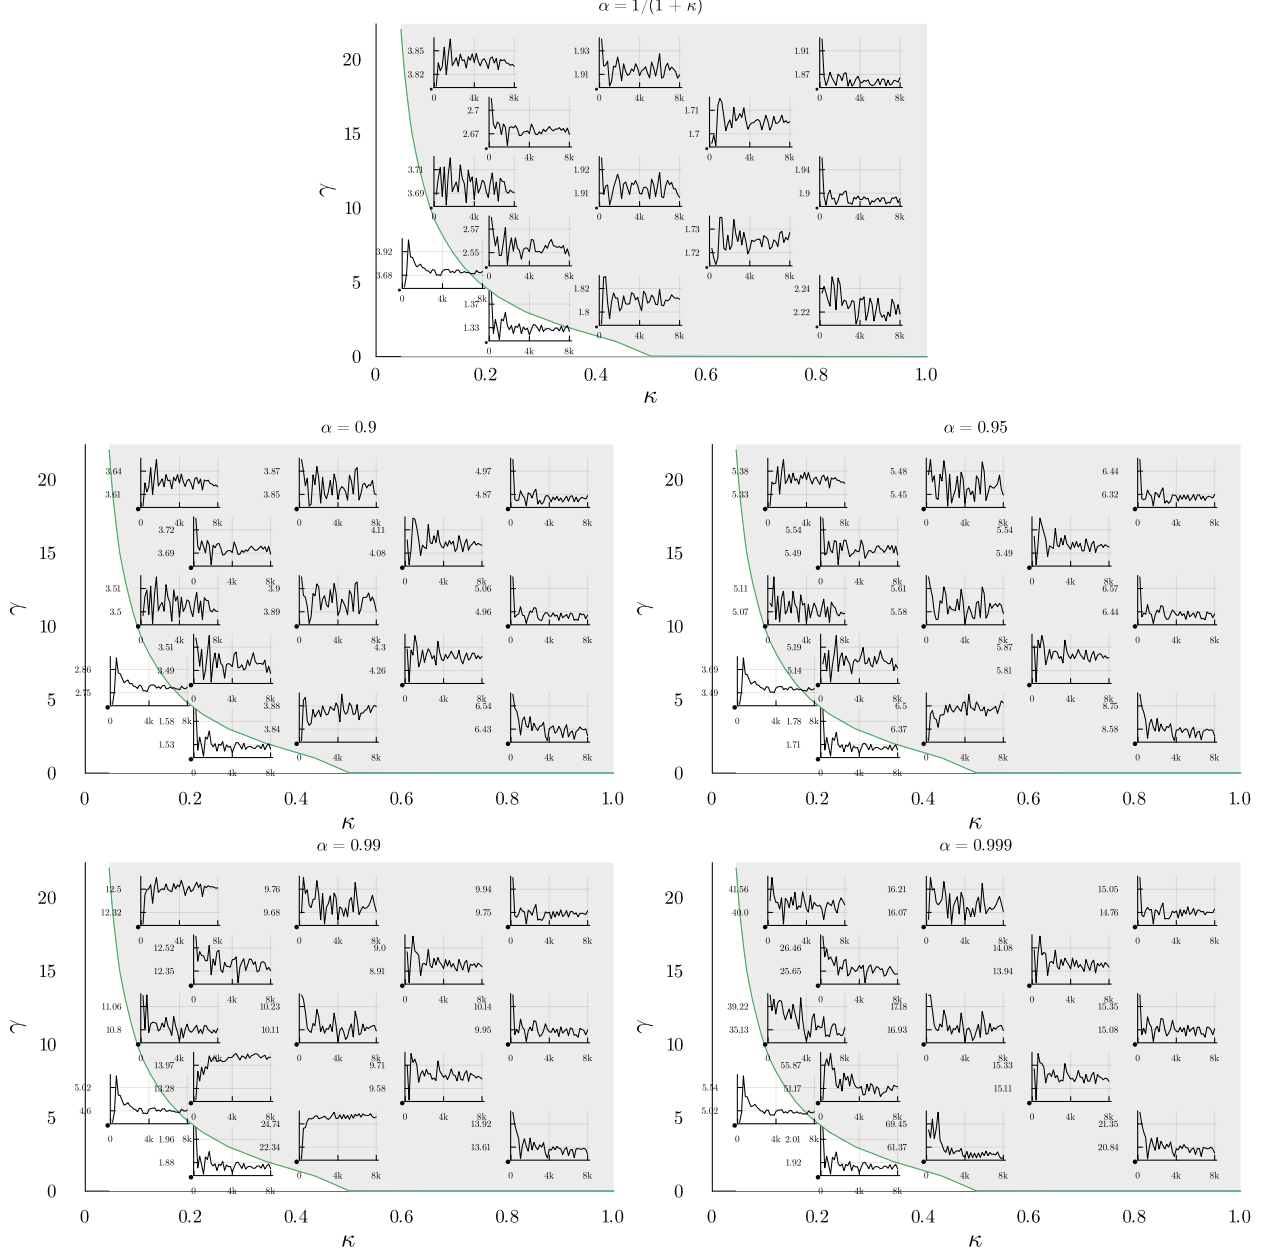

Figure S2: Stochastic boundedness of  $\|\hat{\beta}^{DY}\|_2/\sqrt{n}$  for various  $(\kappa, \gamma, \alpha)$  values. Each panel shows  $\|\hat{\beta}^{DY}\|_2/\sqrt{n}$  for  $\alpha \in \{0.9, 0.95, 0.99, (1+\kappa)^{-1}\}$  for various points in the  $(\kappa, \gamma)$  plane. In each panel, every inset plot shows the average values of  $\|\hat{\beta}^{DY}(\{1+\kappa\}^{-1})\|_2/\sqrt{n}$  for  $n \in \{200, 400, \dots, 8000\}$ , computed over 50 repetitions for each value of  $n$  and each  $(\kappa, \gamma)$  point, in the setting of Figure S1. The white and grey areas in the background indicate regions where the ML estimate does and does not exist asymptotically, respectively.

### S2.3 Adjusted Z-statistics for MDYPL with intercept

In this section we present further simulation evidence to support Conjecture 6.1 in the main text. We fix  $n = 2000$  and let  $p$  vary so that  $\kappa \in \{0.2, 0.4, 0.6, 0.8\}$ , setting  $\alpha = (1+\kappa)^{-1}$  and consider intercept values  $\theta_0 \in \{0.5, 1, \dots, 2.5\}$ . We let  $\mathbf{X}$  be the  $n$  times  $p$  matrix with i.i.d  $\mathcal{N}(0, 1/n)$  entries.  $\beta_0$  has all but  $p/4$  randomly chosen entries set to zero. The nonzero entries are all of the same value and scaled such that

$\gamma^2 = \|\beta_0\|_2^2/n = 5$ . For each combination of  $(\kappa, \theta_0)$ , we draw 5000 independent copies of  $\{\mathbf{X}, \mathbf{y}\}$  from a logistic regression model with intercept. We compute the adjusted  $Z$ -statistics of Theorem 3.4 with  $\mu_*, \sigma_*$  from (15) and compare the empirical 1, 5, 10, 25, 50, 75, 90, 95, 99%-quantiles to those of a  $\mathcal{N}(0, 1)$  distribution. Results are shown in Tables S1 and S2.

Table S1: Empirical distribution of adjusted  $Z$ -statistics from a logistic regression model with intercept using MDYPL; For  $n = 2000$ ,  $\kappa \in \{0.2, 0.4, 0.6, 0.8\}$ ,  $\alpha = 1/(1 + \kappa)$  and  $\theta_0 \in \{0.5, 1, 1.5, 2, 2.5\}$ ,  $\beta_0$  having  $p/4$  nonzero entries of equal magnitude such that  $\gamma^2 = \|\beta_0\|_2^2/n = 5$  and  $\mathbf{x}_j \sim \mathcal{N}(0, n^{-1}\mathbf{I}_p)$ , we draw 5000 independent samples of  $\{\mathbf{X}, \mathbf{y}\}$  according to (14) and compute the adjusted  $Z$ -statistics of Theorem 3.4 with  $\sigma_*$  from (15) for the first coordinate of  $\beta_0$  that is zero. For each combination of  $\kappa, \beta_0$ , we compute the average number of test statistics that lie below the 1, 5, 10, 25, 50, 75, 90, 95, 99%-quantiles of a  $\mathcal{N}(0, 1)$  distribution.

|                |            | Percent adjusted $Z$ -statistics $\leq \mathcal{N}(0, 1)$ -quantiles |     |      |      |      |      |      |      |      |
|----------------|------------|----------------------------------------------------------------------|-----|------|------|------|------|------|------|------|
|                | $\theta_0$ | 1                                                                    | 5   | 10   | 25   | 50   | 75   | 90   | 95   | 99   |
| $\kappa = 0.2$ | 0.5        | 0.7                                                                  | 4.9 | 9.5  | 24.7 | 48.7 | 74.2 | 89.4 | 94.8 | 98.8 |
|                | 1.0        | 1.1                                                                  | 5.4 | 10.1 | 24.3 | 49.8 | 74.8 | 89.1 | 94.9 | 99.0 |
|                | 1.5        | 1.0                                                                  | 5.1 | 10.4 | 25.4 | 50.6 | 75.9 | 90.0 | 94.9 | 99.2 |
|                | 2.0        | 0.9                                                                  | 4.9 | 9.9  | 24.3 | 49.4 | 74.2 | 89.6 | 94.7 | 98.9 |
|                | 2.5        | 1.3                                                                  | 4.8 | 9.8  | 24.9 | 50.2 | 74.8 | 90.2 | 95.2 | 99.2 |
| $\kappa = 0.4$ | 0.5        | 1.1                                                                  | 5.7 | 11.0 | 26.5 | 51.6 | 76.4 | 90.7 | 95.0 | 98.9 |
|                | 1.0        | 1.1                                                                  | 5.0 | 9.9  | 24.7 | 49.8 | 76.0 | 90.4 | 95.2 | 99.1 |
|                | 1.5        | 0.9                                                                  | 4.8 | 10.6 | 25.0 | 50.3 | 75.2 | 89.9 | 94.6 | 98.8 |
|                | 2.0        | 0.9                                                                  | 4.7 | 9.8  | 25.2 | 50.7 | 74.6 | 89.8 | 94.8 | 98.9 |
|                | 2.5        | 1.1                                                                  | 5.3 | 9.7  | 25.0 | 50.1 | 76.0 | 89.9 | 95.3 | 99.1 |
| $\kappa = 0.6$ | 0.5        | 1.0                                                                  | 4.9 | 10.4 | 24.6 | 49.1 | 74.5 | 89.7 | 95.0 | 99.0 |
|                | 1.0        | 1.0                                                                  | 5.2 | 10.5 | 25.3 | 49.5 | 75.1 | 90.4 | 94.8 | 99.2 |
|                | 1.5        | 1.1                                                                  | 5.1 | 10.5 | 25.3 | 49.9 | 75.7 | 90.6 | 95.6 | 99.0 |
|                | 2.0        | 0.8                                                                  | 4.9 | 10.4 | 25.1 | 49.9 | 75.2 | 90.5 | 95.3 | 98.7 |
|                | 2.5        | 0.9                                                                  | 5.0 | 10.1 | 25.3 | 50.3 | 74.9 | 90.2 | 95.1 | 98.9 |
| $\kappa = 0.8$ | 0.5        | 1.0                                                                  | 5.2 | 9.9  | 25.4 | 49.0 | 74.5 | 89.6 | 94.9 | 99.0 |
|                | 1.0        | 1.0                                                                  | 4.9 | 10.2 | 25.2 | 49.6 | 74.2 | 90.0 | 95.1 | 98.9 |
|                | 1.5        | 0.9                                                                  | 4.9 | 10.4 | 26.2 | 50.7 | 75.1 | 89.8 | 95.3 | 98.8 |
|                | 2.0        | 1.3                                                                  | 5.1 | 9.5  | 24.7 | 50.1 | 75.6 | 90.0 | 94.9 | 99.0 |
|                | 2.5        | 1.2                                                                  | 5.3 | 10.4 | 25.0 | 49.5 | 75.3 | 90.9 | 95.6 | 99.1 |

Table S2: Empirical distribution of adjusted Z-statistics from a logistic regression model with intercept using MDYPL; For  $n = 2000$ ,  $\kappa \in \{0.2, 0.4, 0.6, 0.8\}$ ,  $\alpha = 1/(1 + \kappa)$  and  $\theta_0 \in \{0.5, 1, 1.5, 2, 2.5\}$ ,  $\beta_0$  having  $p/4$  nonzero entries of equal magnitude such that  $\gamma^2 = \|\beta_0\|_2^2/n = 5$  and  $\mathbf{x}_j \sim \mathcal{N}(0, n^{-1}\mathbf{I}_p)$ , we draw 5000 independent samples of  $\{\mathbf{X}, \mathbf{y}\}$  according to (14) and compute the adjusted Z-statistics of Theorem 3.4 with  $\sigma_*$  from (15) for the first coordinate of  $\beta_0$  that is nonzero. For each combination of  $\kappa, \beta_0$ , we compute the average number of test statistics that lie below the 1, 5, 10, 25, 50, 75, 90, 95, 99%-quantiles of a  $\mathcal{N}(0, 1)$  distribution.

|                |            | Percent adjusted Z-statistics $\leq \mathcal{N}(0, 1)$ -quantiles |     |      |      |      |      |      |      |      |
|----------------|------------|-------------------------------------------------------------------|-----|------|------|------|------|------|------|------|
|                | $\theta_0$ | 1                                                                 | 5   | 10   | 25   | 50   | 75   | 90   | 95   | 99   |
| $\kappa = 0.2$ | 0.5        | 0.7                                                               | 4.7 | 9.2  | 24.5 | 48.8 | 74.4 | 90.0 | 95.2 | 99.1 |
|                | 1.0        | 1.2                                                               | 5.3 | 10.1 | 25.6 | 50.7 | 75.5 | 90.3 | 94.7 | 99.0 |
|                | 1.5        | 1.0                                                               | 5.0 | 10.3 | 24.9 | 49.4 | 73.7 | 89.9 | 94.9 | 98.7 |
|                | 2.0        | 1.0                                                               | 5.0 | 9.9  | 24.8 | 50.8 | 74.7 | 90.0 | 95.0 | 98.8 |
|                | 2.5        | 1.0                                                               | 4.7 | 9.5  | 23.8 | 49.1 | 74.7 | 89.7 | 95.4 | 99.1 |
|                |            |                                                                   |     |      |      |      |      |      |      |      |
| $\kappa = 0.4$ | 0.5        | 0.9                                                               | 5.3 | 10.2 | 25.6 | 50.5 | 76.3 | 91.0 | 95.5 | 99.2 |
|                | 1.0        | 1.0                                                               | 5.1 | 10.2 | 25.8 | 50.8 | 74.9 | 89.9 | 95.2 | 98.9 |
|                | 1.5        | 1.0                                                               | 5.1 | 10.8 | 25.6 | 49.8 | 75.2 | 89.9 | 95.0 | 99.1 |
|                | 2.0        | 1.0                                                               | 4.9 | 9.8  | 25.3 | 49.7 | 74.3 | 89.7 | 95.0 | 99.0 |
|                | 2.5        | 0.8                                                               | 4.5 | 9.6  | 25.1 | 50.9 | 75.9 | 89.7 | 94.8 | 98.9 |
|                |            |                                                                   |     |      |      |      |      |      |      |      |
| $\kappa = 0.6$ | 0.5        | 0.9                                                               | 5.3 | 10.2 | 25.7 | 50.9 | 75.8 | 90.3 | 95.0 | 98.9 |
|                | 1.0        | 1.0                                                               | 5.1 | 9.9  | 25.1 | 51.0 | 75.6 | 90.7 | 95.2 | 99.0 |
|                | 1.5        | 0.8                                                               | 5.2 | 10.2 | 25.0 | 50.0 | 75.0 | 89.9 | 95.3 | 98.8 |
|                | 2.0        | 1.0                                                               | 4.6 | 9.2  | 24.9 | 50.0 | 74.5 | 90.0 | 95.4 | 99.1 |
|                | 2.5        | 0.9                                                               | 5.1 | 9.8  | 25.0 | 50.7 | 74.8 | 90.2 | 95.2 | 99.2 |
|                |            |                                                                   |     |      |      |      |      |      |      |      |
| $\kappa = 0.8$ | 0.5        | 1.2                                                               | 4.8 | 9.2  | 23.9 | 48.4 | 74.0 | 89.7 | 95.1 | 99.1 |
|                | 1.0        | 1.1                                                               | 5.5 | 10.5 | 25.1 | 50.2 | 75.0 | 89.9 | 94.8 | 99.0 |
|                | 1.5        | 1.1                                                               | 5.2 | 9.7  | 24.8 | 50.0 | 75.8 | 90.6 | 95.2 | 99.1 |
|                | 2.0        | 1.0                                                               | 4.8 | 10.0 | 25.5 | 50.6 | 74.7 | 89.6 | 95.0 | 98.9 |
|                | 2.5        | 0.8                                                               | 4.3 | 9.6  | 25.2 | 49.9 | 74.9 | 89.8 | 94.7 | 99.2 |
|                |            |                                                                   |     |      |      |      |      |      |      |      |

## S2.4 Estimates of $v$ for the simulation study of Section 5.1

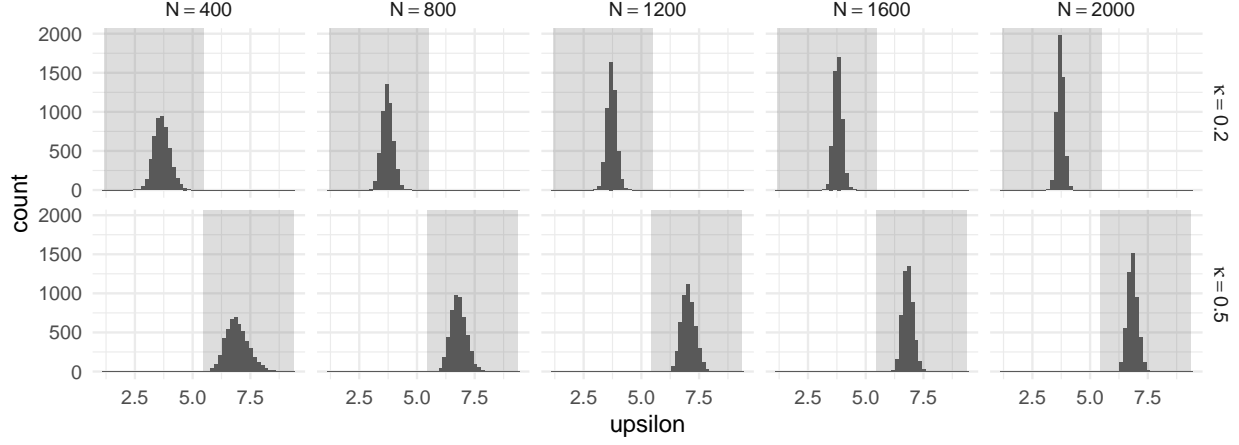

Figure S3: Empirical distribution of the SLOE estimator of  $v$  in the experiments of Section 5.1. The shaded area is the image of the function  $v = h(\gamma)$  for  $\kappa \in \{0.2, 0.5\}$  and  $\alpha = 0.95$ . See Figure 8 of the main text for  $v = h(\gamma)$ .

## A Maximum Diaconis-Ylvisaker prior penalized likelihood

Consider data  $\{\mathbf{y}, \mathbf{X}\}$  with responses  $\mathbf{y} = (y_1, \dots, y_n)^\top$ ,  $y_j \in \{0, 1\}$ , and covariate matrix  $\mathbf{X} \in \mathbb{R}^{n \times p}$  with rows  $\mathbf{x}_j \in \mathbb{R}^p$  ( $j = 1, \dots, n$ ). A logistic regression model assumes that conditional on  $\mathbf{x}_j$ , the responses  $y_j$  are independent realizations of Bernoulli random variables with mean  $\zeta'(\mathbf{x}_j^\top \boldsymbol{\beta}_0)$  where  $\zeta(x) = \log(1 + e^x)$  and  $\boldsymbol{\beta}_0 \in \mathbb{R}^p$  is the unknown  $p$ -dimensional vector of regression coefficients.

Given hyperparameters  $\alpha \in (0, 1]$  and  $\boldsymbol{\beta}_P \in \mathbb{R}^p$ , the logarithm of the Diaconis and Ylvisaker (1979) prior, bar the normalizing constant, for the logistic regression model is given by

$$\log p(\boldsymbol{\beta}; \mathbf{X}) = \frac{1 - \alpha}{\alpha} \sum_{j=1}^n \{ \zeta'(\mathbf{x}_j^\top \boldsymbol{\beta}_P) \mathbf{x}_j^\top \boldsymbol{\beta} - \zeta(\mathbf{x}_j^\top \boldsymbol{\beta}) \}, \quad (\text{S1})$$

where  $\boldsymbol{\beta}_P$  is the mode of the prior, while  $\alpha$  controls the variability of the prior distribution. The DY-prior penalized log-likelihood, without the normalizing constant is given by

$$\ell^*(\boldsymbol{\beta}; \mathbf{y}, \mathbf{X}) = \frac{1}{\alpha} \sum_{j=1}^n \{ (\alpha y_j + (1 - \alpha) \zeta'(\mathbf{x}_j^\top \boldsymbol{\beta}_P)) \mathbf{x}_j^\top \boldsymbol{\beta} - \zeta(\mathbf{x}_j^\top \boldsymbol{\beta}) \}. \quad (\text{S2})$$

The maximiser of (S2) is denoted by  $\hat{\boldsymbol{\beta}}^{\text{DY}}$ . Hence,  $\hat{\boldsymbol{\beta}}^{\text{DY}}$  is the maximiser of a logistic regression model log-likelihood with pseudo-responses  $\mathbf{y}^* = (y_1^*, \dots, y_n^*)^\top$ ,  $y_j^* = \alpha y_j + (1 - \alpha) \zeta'(\mathbf{x}_j^\top \boldsymbol{\beta}_P)$ ,  $\alpha \in (0, 1]$ . For the remainder of this work,  $\boldsymbol{\beta}_P = \mathbf{0}_p$  and  $\hat{\boldsymbol{\beta}}^{\text{DY}}$  is understood as the maximiser of  $\ell(\boldsymbol{\beta}; \mathbf{y}^*, \mathbf{X})$ .

## B Proof of Theorem 3.1

As in Sur and Candès (2019), we assume that the model matrix  $\mathbf{X}$  has independent rows  $\mathbf{x}_i \sim \mathcal{N}(\mathbf{0}_p, n^{-1} \mathbf{I}_p)$ , where  $\mathbf{I}_p$  is the  $p \times p$  identity matrix, and that the linear predictors  $\mathbf{x}_i^\top \boldsymbol{\beta}_0$  have asymptotic variance  $\lim_{n \rightarrow \infty} \text{var}(\mathbf{x}_i^\top \boldsymbol{\beta}_0) = \lim_{n \rightarrow \infty} \|\boldsymbol{\beta}_0\|_2^2 / n = \gamma^2$ . It is further assumed that there exists a random variable  $\bar{\beta} \sim \pi_{\bar{\beta}}$  with finite second moment, such that the empirical distribution of the entries of  $\boldsymbol{\beta}_0$  converges weakly in distribution to  $\pi_{\bar{\beta}}$  and  $\lim_{n \rightarrow \infty} \frac{1}{p} \sum_{j=1}^n \beta_{0,j}^2 = \mathbb{E}(\bar{\beta}^2)$ . Finally, let  $\lim_{n \rightarrow \infty} p/n = \kappa$  for  $\kappa \in (0, 1)$ .

## B.1 Asymptotic characterisation via stationary state evolution

Recall the state evolution equations (S3), (S4), (S5) below.

$$\mathbb{E} \left[ 2\zeta'(Z)Z \left\{ \frac{1+\alpha}{2} - \zeta' \left( \text{prox}_{b\zeta} \left( Z_* + \frac{1+\alpha}{2}b \right) \right) \right\} \right] = 0 \quad (\text{S3})$$

$$1 - \kappa - \mathbb{E} \left[ \frac{2\zeta'(Z)}{1 + b\zeta''(\text{prox}_{b\zeta}(Z_* + \frac{1+\alpha}{2}b))} \right] = 0 \quad (\text{S4})$$

$$\sigma^2 - \frac{b^2}{\kappa^2} \mathbb{E} \left[ 2\zeta'(Z) \left\{ \frac{1+\alpha}{2} - \zeta' \left( \text{prox}_{b\zeta} \left( Z_* + \frac{1+\alpha}{2}b \right) \right) \right\}^2 \right] = 0. \quad (\text{S5})$$

Here,  $Z \sim N(0, \gamma^2)$ ,  $Z_* = \mu Z + \kappa^{1/2}\sigma G$  for  $G \sim N(0, 1)$  which is independent of  $Z$ ,  $\zeta'(\cdot), \zeta''(\cdot)$  are the first and second derivatives of  $\zeta(\cdot)$  and  $\text{prox}_{b\zeta}(x) = \arg \min_u \{b_*\zeta(u) + \frac{1}{2}(x-u)^2\}$  denotes the proximal operator. Equations (S3)-(S5) define the stationary points to the state evolution iterates (S16)-(S18) of the AMP recursion (S12)-(S13). A discussion about how these equations are derived is thus postponed to B.4.2.

Denote by  $\mathbf{J}(\mu, b, \sigma)$  the Jacobian matrix of the LHS of (S3)-(S5) with respect to  $(\mu, b, \sigma)$ .

**Theorem 3.1.** *Assume that  $(\alpha, \kappa, \gamma)$  are such that  $\|\hat{\beta}^{\text{DY}}\|_2 = \mathcal{O}(n^{1/2})$  almost surely and that (S3)-(S5) admit a solution  $(\mu_*, b_*, \sigma_*)$  such that  $\mathbf{J}(\mu_*, b_*, \sigma_*)$  is nonsingular. Then for any function  $\psi : \mathbb{R}^2 \rightarrow \mathbb{R}$  that is pseudo-Lipschitz of order 2,*

$$\frac{1}{p} \sum_{j=1}^n \psi(\hat{\beta}_j^{\text{DY}} - \mu_* \beta_{0,j}, \beta_{0,j}) \xrightarrow{a.s.} \mathbb{E}[\psi(\sigma_* G, \bar{\beta})], \quad \text{as } n \rightarrow \infty, \quad (\text{S6})$$

where  $G \sim N(0, 1)$  is independent of  $\bar{\beta} \sim \pi_{\bar{\beta}}$ .

The proof of Theorem 3.1 closely follows the proof of Theorem 1 in Sur and Candès (2019). We replace the logistic indicator function  $h(u, v) = \{1 - \text{sign}(v \leq \zeta'(u))\}/2$  is simply replaced by  $h(u, v) = \alpha \{1 - \text{sign}(v \leq \zeta'(u))\}/2 + (1 - \alpha)/2$  and the derivations are adjusted accordingly. Further, we provide a smoothing argument that formally justifies the asymptotic results of the relevant AMP recursion, and which has been missing hitherto.

## B.2 Proof outline for Theorem 3.1

The following steps constitute the proof of Theorem 3.1:

- A.2.1) *Target AMP recursion:* As a starting point, we formulate an AMP recursion, whose stationary point coincides with  $\hat{\beta}^{\text{DY}}$ .
- A.2.2) *Centred target AMP recursion:* Based on the target AMP recursion, we devise a centred AMP recursion, for which the aggregate asymptotic behaviour can be established via existing AMP results.
- A.2.3) *Matrix-valued AMP embedding:* The centred AMP recursion is embedded into a symmetric, matrix valued AMP recursion of Javanmard and Montanari (2013) for which the topical AMP asymptotics hold. A reduction argument, which is also due to Javanmard and Montanari (2013) and which was subsequently used in Donoho and Montanari (2016) and Sur and Candès (2019), identifies the correct asymptotic behaviour for the centred AMP recursion.
- A.2.4) *Smoothing argument:* As the logistic indicator function is not Lipschitz, which is a prerequisite for the application of the asymptotic result of Javanmard and Montanari 2013, Theorem 1, we instead establish a Lipschitz approximation to the indicator function that is parametrised by  $\epsilon > 0$ , such that  $\epsilon = 0$  recovers the original recursions of A.2.1 and A.2.2.

A.2.5) *Asymptotic equivalence of target and centred AMP*: Next, we show that the target recursion and the centred AMP recursion, whose asymptotic behaviour is characterised through A.2.3, are asymptotically equivalent for sufficiently large iterations.

A.2.6) *Asymptotic equivalence of AMP and MDYPL*: Finally, we shown that for  $\epsilon \rightarrow 0$ , the approximate AMP iterates are arbitrarily close to  $\hat{\beta}^{\text{DY}}$ , asymptotically, if iterated for sufficiently long.

### B.3 Matrix-valued AMP

For the readers' convenience, this subsection introduces the matrix valued AMP recursion of Javanmard and Montanari (2013), which is the theoretical workhorse to derive the asymptotic behaviour of the AMP recursion of interest. It is more or less a verbatim replication of Javanmard and Montanari 2013, Section 2, tailored to the specific requirements of the problem at hand.

Given integers  $q, N$ , let  $\mathcal{V}_{q,N} \equiv (\mathbb{R}^q)^N$ , so that a vector  $x \in \mathcal{V}_{q,N}$  is regarded as a  $N$ -vector with entries in  $\mathbb{R}^q$ , i.e.  $x = (\mathbf{x}_1, \dots, \mathbf{x}_N)$  where  $\mathbf{x}_i \in \mathbb{R}^q$  with components denoted by  $\mathbf{x}_i = (\mathbf{x}_i(1), \dots, \mathbf{x}_i(q))$  ( $i = 1, \dots, N$ ). Given  $x \in \mathcal{V}_{q,N}$ , define its  $\ell_2$ -norm as  $\|x\|_2 = \left( \sum_{i=1}^N \|\mathbf{x}_i\|_2^2 \right)^{1/2}$ . Given a matrix  $\mathbf{A} \in \mathbb{R}^{N \times N}$ , let it act on  $\mathcal{V}_{q,N}$  so that for  $v, v' \in \mathcal{V}_{q,N}$ ,  $v' = \mathbf{A}v$  for  $\mathbf{v}'_i = \sum_{j=1}^N A_{ij} \mathbf{v}_j$  for  $i \in [N]$ , where  $[N]$  denotes the integers  $1, \dots, N$ . That is,  $\mathbf{A}$  is identified with the Kronecker product  $\mathbf{A} \otimes \mathbf{I}_q$  when acting on elements of  $\mathcal{V}_{N,q}$ .

**Definition 1** (Symmetric AMP). A symmetric AMP instance is a triple  $(\mathbf{A}, \mathcal{F}, x^0)$ , where

- 1)  $\mathbf{A} = \mathbf{G} + \mathbf{G}^\top$ , where  $\mathbf{G} \in \mathbb{R}^{N \times N}$  has i.i.d.  $N(0, (2N)^{-1})$  entries
- 2)  $\mathcal{F} = \{f^k : k \in [N]\}$  is a collection of mappings  $f^k : \mathbb{R}^q \times \mathbb{N} \rightarrow \mathbb{R}^q$ ,  $(\mathbf{x}, t) \mapsto f^k(\mathbf{x}, t)$  is locally Lipschitz in its first argument
- 3)  $x^0 \in \mathcal{V}_{q,N}$  is an initial condition.

Given  $\mathcal{F} = \{f^k : k \in [N]\}$ , denote by  $f(\cdot, t)$  the mapping from  $\mathcal{V}_{q,N} \rightarrow \mathcal{V}_{q,N}$  such that  $v' = f(v, t)$  for  $\mathbf{v}'_i = f^i(\mathbf{v}_i, t)$  and all  $i \in [N]$ .

**Definition 2** (AMP orbit). The AMP orbit corresponding to an AMP instance  $(\mathbf{A}, \mathcal{F}, x^0)$  is the sequence of vectors  $\{x^t\}_{t \in \mathbb{N}_0}$ ,  $x^t \in \mathcal{V}_{q,N}$  such that for  $t \geq 0$ ,

$$x^{t+1} = \mathbf{A}f(x^t, t) - \mathbf{B}_t f(x^{t-1}, t-1), \quad (\text{S7})$$

where  $\mathbf{B}_t : \mathcal{V}_{q,N} \rightarrow \mathcal{V}_{q,N}$  is the linear operator such that for  $v' = \mathbf{B}_t v$ ,

$$\mathbf{v}'_i = \left( \frac{1}{N} \sum_{j=1}^N \frac{\partial f^j}{\partial \mathbf{x}}(\mathbf{x}_j^t, t) \right) \mathbf{v}_i,$$

and where  $\frac{\partial f^j}{\partial \mathbf{x}}$  denotes the Jacobian matrix of  $f^j(\cdot, t) : \mathbb{R}^q \rightarrow \mathbb{R}^q$  given  $t$ .

Any expression with negative  $t$ -index is considered zero in the above definition.

**Definition 3** (Converging AMP). A sequence of AMP instances  $\{(\mathbf{A}(N), \mathcal{F}_N, x^{0,N})\}_{N \in \mathbb{N}_0}$  is said to be converging if

- i) There exist integers  $q, q'$ , and
- ii) a function  $g : \mathbb{R}^q \times \mathbb{R}^q \times [q'] \times \mathbb{N} \rightarrow \mathbb{R}^q$  with  $g(\mathbf{x}, \mathbf{y}, a, t) = (g_1(\mathbf{x}, \mathbf{y}, a, t), \dots, g_q(\mathbf{x}, \mathbf{y}, a, t))$ , such that for each  $r \in [q], a \in [q'], t \in \mathbb{N}$ ,  $g_r(\cdot, \cdot, a, t)$  is Lipschitz,
- iii)  $q'$  probability measures  $P_1, \dots, P_{q'}$  on  $\mathbb{R}^q$ ,

iv) for each  $N$ , a finite partition  $C_1^N \cup \dots \cup C_{q'}^N = [N]$ ,

v)  $q'$  positive definite matrices  $\widehat{\Sigma}_1^0, \dots, \widehat{\Sigma}_{q'}^0 \in \mathbb{R}^{q \times q}$ ,

such that the following happens:

- 1) For each  $a \in [q']$ , one has  $\lim_{N \rightarrow \infty} \frac{|C_a^N|}{N} = c_a \in (0, 1)$ ,
- 2) There exists  $y \in \mathcal{V}_{q,N}$  with  $y = (\mathbf{y}_1, \dots, \mathbf{y}_N)$ ,  $\mathbf{y}_i \in \mathbb{R}^q$  ( $i = 1, \dots, N$ ), such that for each  $N \in \mathbb{N}_0$ ,  $a \in [q']$ ,  $i \in C_a^N$ ,  $f^i(\mathbf{x}, t) = g(\mathbf{x}, \mathbf{y}_i, a, t)$ . Further, the empirical distribution of  $\{\mathbf{y}_i\}_{i \in C_a^N}$ , denote it by  $\widehat{P}_a$ , converges weakly to  $P_a$ , i.e.

$$\frac{1}{|C_a^N|} \sum_{i \in C_a^N} \delta_{\mathbf{y}_i} \xrightarrow{d} P_a,$$

- 3) For each  $a \in [q']$ , in probability,

$$\lim_{N \rightarrow \infty} \frac{1}{|C_a^N|} \sum_{i \in C_a^N} g(\mathbf{x}_i^0, \mathbf{y}_i, a, 0) g(\mathbf{x}_i^0, \mathbf{y}_i, a, 0)^\top = \widehat{\Sigma}_a^0.$$

This definition follows Remark 1 of Javanmard and Montanari (2013) and allows for a partition size  $q'$  that is distinct from  $q$ . Further note that the functions  $f^i(\cdot, \cdot)$  of Definition 3, 2), depends on  $\mathbf{y}_i$ , but as these do not change between iterations, this dependence is suppressed for notational convenience.

**Definition 4** (State evolution). Given  $q, q' \in \mathbb{N}_0$  and starting points  $\{\widehat{\Sigma}_a^0\}_{a \in [q']}$ ,  $\widehat{\Sigma}_a^0 \in \mathbb{R}^{q \times q}$  positive definite, and weights  $\{c_a\}_{a \in [q']}$ ,  $c_a \in \mathbb{R}$ , the state evolution defines a sequence of positive definite matrices  $\{\Sigma^t\}_{t \in \mathbb{N}}$ , such that for each  $t \in \mathbb{N}$ ,

$$\Sigma^t = \sum_{b=1}^{q'} c_b \widehat{\Sigma}_b^{t-1} \tag{S8}$$

$$\widehat{\Sigma}_a^t = \mathbb{E} [g(Z_a^t, Y_a, a, t) g(Z_a^t, Y_a, a, t)^\top] \quad (a = 1, \dots, q'), \tag{S9}$$

where  $Y_a \sim P_a$ ,  $Z_a^t \sim N(\mathbf{0}_q, \Sigma^t)$  and where  $Y_a \perp Z_a^t$  for  $a \in [q']$ .

It is now possible to state Theorem 1 of Javanmard and Montanari (2013) which will serve as the blackbox result to establish the asymptotic behaviour of the MDYPL estimator. This result makes use of pseudo-Lipschitz functions, a definition of which is given for completeness.

**Definition 5** (Pseudo-Lipschitzianity). For  $k \geq 1$ , a function  $\psi : \mathbb{R}^m \rightarrow \mathbb{R}$  is said to be pseudo-Lipschitz of order  $k$ , denote the corresponding class of functions by  $\text{PL}(k)$ , if there exists a constant  $L > 0$  such that for all  $\mathbf{u}, \mathbf{v} \in \mathbb{R}^m$ ,

$$|\psi(\mathbf{u}) - \psi(\mathbf{v})| \leq L \left( 1 + \|\mathbf{u}\|_2^{k-1} + \|\mathbf{v}\|_2^{k-1} \right) \|\mathbf{u} - \mathbf{v}\|_2.$$

Hence, if  $\psi \in \text{PL}(k)$ , there exists a constant  $L'$  such that for all  $\mathbf{u} \in \mathbb{R}^m$ ,  $|\psi(\mathbf{u})| \leq L'(1 + \|\mathbf{u}\|_2^k)$ . Further, note that every Lipschitz function is also pseudo Lipschitz for any  $k \geq 1$ .

**Theorem B.1** (Javanmard and Montanari (2013) Theorem 1). *Let  $\{(\mathbf{A}(N), \mathcal{F}_N, x^{0,N})\}_{N \in \mathbb{N}_0}$  be a converging sequence of AMP instances and denote by  $\{x^t\}_{t \in \mathbb{N}_0}$  the corresponding AMP orbit. Suppose further that for some  $k \geq 2$  and all  $a \in [q']$ ,  $E_{P_a}[\|Y_a\|^{2k-2}]$  is bounded and that  $E_{\widehat{P}_a}[\|Y_a\|^{2k-2}] \rightarrow E_{P_a}[\|Y_a\|^{2k-2}]$*

as  $N \rightarrow \infty$ . Then for all  $t \in \mathbb{N}$ ,  $a \in [q']$  and any pseudo-Lipschitz function  $\psi : \mathbb{R}^q \times \mathbb{R}^q \rightarrow \mathbb{R}$  of order  $k$ ,

$$\lim_{N \rightarrow \infty} \frac{1}{|C_a^N|} \sum_{i \in C_a^N} \psi(\mathbf{x}_i^t, \mathbf{y}_i) = E[\psi(Z_a^t, Y_a)],$$

where  $Y_a \sim P_a$ ,  $Z_a^t \sim N(\mathbf{0}_q, \Sigma^t)$  and  $Y_a \perp Z_a^t$ .

## B.4 Proof of Theorem 3.1

### B.4.1 Target AMP recursion

Consider the following recursion. Given initial conditions  $\hat{\beta}^0$ ,  $\mathbf{S}^0 = \mathbf{X}\hat{\beta}^0$ , and a sequence of constants  $\{\mu_t, b_t, \sigma_t\}_{t \in \mathbb{N}_0}$ , for  $t \in \mathbb{N}$ , set

$$\hat{\beta}^t = \hat{\beta}^{t-1} + \kappa^{-1} \mathbf{X}^\top \Psi^{t-1}(\mathbf{y}^*, \mathbf{S}^{t-1}) \quad (\text{S10})$$

$$\mathbf{S}^t = \mathbf{X}\hat{\beta}^t - \Psi^{t-1}(\mathbf{y}^*, \mathbf{S}^{t-1}), \quad (\text{S11})$$

where  $\Psi^t(\mathbf{y}^*, \mathbf{S}^t)$  acts elementwise on  $\mathbf{y}^*, \mathbf{S}^t$  as

$$\Psi^t(y_i^*, \mathbf{S}_i^t) = b_t \{y_i^* - \zeta'(\text{prox}_{b_t \zeta}(b_t y_i^* + \mathbf{S}_i^t))\},$$

for  $i = 1, \dots, n$  and where  $y_i^* = \alpha y_i + (1 - \alpha)/2$ . For  $\alpha = 1$ , this recursion corresponds to equations (49) and (50) of the supplementary material of Sur and Candès (2019).

The relation of this recursion to the maximiser of  $\ell(\beta; \mathbf{y}^*, \mathbf{X})$  is shown in Sur and Candès 2019, Appendix B: If there exists a fixed points  $\hat{\beta}_*, \mathbf{S}_*$  along with  $(\mu_*, b_*, \sigma_*)$ , then by construction

$$\begin{aligned} \mathbf{X}^\top b_* (\mathbf{y}^* - \zeta'(\text{prox}_{b_* \zeta}(b_* \mathbf{y}^* + \mathbf{S}_*))) &= \mathbf{0}_p \\ (b_* \mathbf{y}^* + \mathbf{S}_*) - b_* \zeta'(\text{prox}_{b_* \zeta}(b_* \mathbf{y}^* + \mathbf{S}_*)) &= \mathbf{X}\hat{\beta}_*. \end{aligned}$$

Now using that  $x - b\zeta'(\text{prox}_{b\zeta}(x)) = \text{prox}_{b\zeta}(x)$ , it follows immediately that

$$\mathbf{X}^\top (\mathbf{y}^* - \zeta'(\mathbf{X}\hat{\beta}_*)) = \mathbf{0}_p,$$

the left hand side of which is proportional to the gradient of (S2), and by strict concavity thereof,  $\hat{\beta}_*$  is equal to  $\hat{\beta}^{\text{DY}}$ .

### B.4.2 Centred target AMP recursion

Instead of analysing the target AMP recursion directly, a centred variant thereof is analysed. This centring ensures that the iterates of the resulting recursion have well-defined limits that are understood by AMP theory (See remarks in Donoho and Montanari 2016, Appendix B). In particular, as in Sur and Candès (2019) and Donoho and Montanari (2016), consider the following centred recursion with adjusted initial conditions  $\boldsymbol{\nu}^0 = \hat{\beta}^0 - \mu_0 \beta_0$ ,  $\mathbf{R}^0 = \mathbf{S}^0$  for  $\hat{\beta}^0, \beta_0 \in \mathbb{R}^p$ ,  $\mu_0 \in \mathbb{R}$  and  $\mathbf{S}^0 \in \mathbb{R}^n$ , for  $t \in \mathbb{N}$ , let

$$\boldsymbol{\nu}^t = q_{t-1}(\boldsymbol{\nu}^{t-1} + \mu_{t-1} \beta_0) - a_t \beta_0 + \kappa^{-1} \mathbf{X}^\top \Psi^{t-1}(\mathbf{y}^*, \mathbf{R}^{t-1}) \quad (\text{S12})$$

$$\mathbf{R}^t = \mathbf{X}(\boldsymbol{\nu}^t + \mu_t \beta_0) - \Psi^{t-1}(\mathbf{y}^*, \mathbf{R}^{t-1}), \quad (\text{S13})$$

where  $a_0 = \mu_0$  and for  $t \in \mathbb{N}$ ,

$$q_t = -\frac{1}{\kappa n} \sum_{i=1}^n \frac{\partial \Psi^t}{\partial R}(y_i^*, R) \Big|_{R=\mathbf{R}_i^t} \quad (\text{S14})$$

$$a_t = \frac{1}{\kappa n} \sum_{i=1}^n \frac{\partial \Psi^{t-1}}{\partial Z}(h(Z, \bar{\varepsilon}_i), \mathbf{R}_i^{t-1}) \Big|_{Z=\mathbf{x}_i^\top \beta_0}, \quad (\text{S15})$$

where  $\bar{\varepsilon}_i \sim U(0, 1)$  ( $i = 1, \dots, n$ ) are i.i.d. draws independent of all other random variables.

Given initial conditions  $(\mu_0, b_0, \sigma_0)$ , let the state evolution of  $(\mu_t, b_t, \sigma_t)$  be characterised by the solution to the following system of nonlinear equations

$$1 - \kappa = \mathbb{E} \left[ \frac{1}{1 + b_t \zeta''(\text{prox}_{b_t \zeta}(b_t Y^* + Z_t))} \right] \quad (\text{S16})$$

$$\mu_{t+1} = \frac{b_t}{\kappa \gamma^2} \mathbb{E} [Z \{Y^* - \zeta'(\text{prox}_{b_t \zeta}(b_t Y^* + Z_t))\}] + \mu_t \quad (\text{S17})$$

$$\sigma_{t+1}^2 = \frac{b_t^2}{\kappa^2} \mathbb{E} [\{Y^* - \zeta'(\text{prox}_{b_t \zeta}(b_t Y^* + Z_t))\}^2], \quad (\text{S18})$$

for independent  $Z \sim N(0, \gamma^2)$ ,  $G \sim N(0, 1)$ , and  $\bar{\varepsilon} \sim U(0, 1)$ , and letting

$$Y^* = \frac{\alpha}{2} \{1 - \text{sign}(\bar{\varepsilon} - \zeta'(Z))\} + \frac{1 - \alpha}{2}, \quad Z_t = \mu_t Z + \kappa^{1/2} \sigma_t G.$$

The iterate of  $\sigma_{t+1}$  in (S18) arises from the state evolution  $\Sigma^t$  (cf. Definition 4) that characterises the variance of the AMP iterates (S10) and (S11) as is shown in (S50). On the other hand,  $b_t, \mu_t$  come from the nonlinear corrections  $a_t, q_t$  in (S14) and (S14) to the recursion (S10) and (S11). (S53) and (S55)-(S59), establish the relation between  $b_t, \mu_t$  and the corrections  $a_t, q_t$ . These corrections ensure that the AMP iterates have a tractable asymptotic distribution. It is customary in the AMP literature to refer to the iterates  $\mu_t, b_t, \sigma_t$  as state evolutions and equations (S36)-(S38) as state evolution equations – a convention which is henceforth adhered to in this text. Feng *et al.* (2022), Section 2.1, and Section 4 provide a thorough discussion of the state evolutions and their role in AMP.

The relation to equations (22)-(24) of the supplementary material of Sur and Candès (2019) and equation (118) in Feng *et al.* (2022) is evident.

### B.4.3 Matrix-valued AMP-embedding

This section embeds the centred AMP recursion of (B.4.2) in a symmetric AMP-instance, which is shown to satisfy all properties of Definitions 1-4, apart from a Lipschitzianity constraint on  $g(\cdot, \cdot, a, t)$  in Definition 3, which is dealt with in Section B.4.4. Theorem B.1 then characterises the asymptotic behaviour of said recursion. In particular, the centred recursion of (S12)-(S15), which is not symmetric, is embedded in a symmetric AMP recursion as defined in B.4.1. A subset of the resulting orbit then corresponds to the orbit of interest, namely (S12)-(S15). This approach was proposed in Javanmard and Montanari (2013, Lemma 1) and also followed in Sur and Candès (2019, Lemma 3) and Donoho and Montanari (2016, Lemma C.1). The symmetric AMP instance is built up for even and odd iterates and the partition  $[n] \cup [N] \setminus [n]$  of  $[N]$  separately, which is then extended to a complete AMP recursion.

In what follows, iterates are indicated by the letters  $t, t-1, t-2$  and 0, which for scalar values are used as subscripts, e.g.  $\mu_0, \sigma_{t-1}$  and are used as superscripts for functions and nonscalar elements, e.g.  $\Psi^{t-1}(\mathbf{y}, \mathbf{R}^{t-1})$ .

Relating a recursion that is parametrised in terms of model parameters  $\mathbf{y}, y_i, \mathbf{X}, \mathbf{x}_i$  etc. and a general AMP recursion, which is parametrised by elements such as  $x, y, \mathbf{x}_i, \mathbf{y}_i, Y_a$  may lead to confusion. For this reason, an effort is made to point out the disparity. It is specifically pointed out that boldface elements pertaining to the original model use mathematical boldface (e.g.  $\mathbf{x}_i$ ), while boldface elements of a AMP recursion use standard boldface (e.g.  $\mathbf{x}_i$ ). Moreover, note that Javanmard and Montanari (2013) chose symbols  $x, y$  to denote elements in  $\mathcal{V}_{q,N}$ , and in particular,  $y = (\mathbf{y}_1, \dots, \mathbf{y}_N)$ , a convention which is kept for comparability. This is not the same as  $\mathbf{y} = (y_1, \dots, y_n)$ , which is used to denote the response variables in the logistic regression model. Moreover, the response variables  $y_i$  are assumed to be realizations of random variables  $Y_i$  for  $i = 1, \dots, n$ . This may stand in conflict with  $Y_a$ , the random variables in  $\mathbb{R}^q$  as defined in the AMP setup, which are indexed by partition cell labels  $a \in [q']$ . To avoid ill-definedness, the index  $i$  is exclusively used when referring to the Bernoulli random variables  $Y_i$  that give rise to observations  $y_i$ , while the subscript  $a$  is used in the context of the random variables for the AMP recursion. Finally, recall that  $\beta_0 \in \mathbb{R}^p$  is the parameter vector that is to be estimated, not an initial condition.

Let  $q$  be an arbitrarily large integer,  $q' = 2$ ,  $N = n + p$ , where  $n, p$  denote the rows and columns of  $\mathbf{X}$ , respectively, and  $\kappa = \kappa(N) = p/n$ . Following Definition 1, 1), let  $\mathbf{A}$  be the symmetric  $N \times N$  matrix whose

upper triangular entries are given by  $\mathbf{A}_{ij} = \sqrt{n/N} \mathbf{X}_{i,j-n}$  for  $i \in [n]$  and  $j \in [N] \setminus [n]$ , and all other entries  $\mathbf{A}_{ij}$   $i < j$  are i.i.d.  $N(0, N^{-1})$  independent of all other entries in  $\mathbf{A}$ . That is, letting  $\mathbf{B}_1, \mathbf{B}_2$  be  $n \times n$  matrices with i.i.d.  $N(0, (2N)^{-1})$  entries and defining  $\mathbf{C}_k = \mathbf{B}_k + \mathbf{B}_k^\top$  for  $k = 1, 2$ , then

$$\mathbf{A} = \begin{bmatrix} \mathbf{C}_1 & \sqrt{\frac{n}{N}} \mathbf{X} \\ \sqrt{\frac{n}{N}} \mathbf{X}^\top & \mathbf{C}_2 \end{bmatrix}. \quad (\text{S19})$$

Next, the collection of functions  $\mathcal{F}$  is constructed. For this, recall from Definition 3, 2), that the collections  $\mathcal{F}_N$  of a converging sequence of AMP-instances with functions  $f^i(\cdot, \cdot)$  may depend on  $\mathbf{y}_i$  for some  $y \in \mathcal{V}_{q,N}$ . Hence, given  $\mathbf{x}, \mathbf{y}_i \in \mathbb{R}^q$ , which should be thought of as entries of some  $x, y \in \mathcal{V}_{q,N}$  that are concretely specified in (S22) and (S23), for  $i \in [n]$ , and odd  $t$ , define  $f^i(\mathbf{x}, t)$  as

$$f^i(\mathbf{x}, t) = \kappa^{-1} \sqrt{\frac{N}{n}} \left[ 0, \Psi^0(h(\mathbf{x}(1), \mathbf{y}_i(1)), \mathbf{x}(3)), 0, \Psi^1(h(\mathbf{x}(1), \mathbf{y}_i(1)), \mathbf{x}(5)), \dots, \Psi^{\frac{t-1}{2}}(h(\mathbf{x}(1), \mathbf{y}_i(1)), \mathbf{x}(t+2)), 0, 0, \dots \right]^\top. \quad (\text{S20})$$

whereas for  $i \in [N] \setminus [n]$  and odd  $t$ , let  $f^i(\mathbf{x}, t) = \mathbf{0}_q$ . Further, for  $i \in [n]$  and even  $t$ ,  $f^i(\mathbf{x}, t) = \mathbf{0}_q$  and for  $i \in [N] \setminus [n]$ , even  $t$ , let

$$f^i(\mathbf{x}, t) = \sqrt{\frac{N}{n}} \left[ \mathbf{y}_i(1), 0, \mathbf{y}_i(2) + \mu_0 \mathbf{y}_i(1), 0, \mathbf{x}(2) + \mu_1 \mathbf{y}_i(1), 0, \mathbf{x}(4) + \mu_2 \mathbf{y}_i(1), 0, \dots, \mathbf{x}(t) + \mu_{\frac{t}{2}} \mathbf{y}_i(1), 0, 0, \dots \right]^\top. \quad (\text{S21})$$

For well-definedness of (S20), (S21), which map to  $\mathbb{R}^q$ , it must be the case that  $t \leq q - 3$ , which is of no consequence as  $q$  can always be chosen large enough to accommodate any  $t \in \mathbb{R}$ . Hence, without loss of generality, all results are stated for  $t \in [q]$ , rather than  $t \in [\tilde{q}]$  for  $\tilde{q} = q + 3$  to simplify presentation.

It is straightforward to establish that  $f^i(\cdot, t)$  is locally Lipschitz in its first argument, which is shown formally for the smoothed version of B.4.4, to which Theorem B.1 applies ultimately. To conclude the symmetric AMP-instance, let  $x^0 = \mathbf{0}_{N,q}$  be the  $N$ -vector with elements  $\mathbf{0}_q$ .

With these definitions in place, it is possible to define the iterates  $x^t$  and  $y$  that give rise to the target AMP recursion. In particular, let  $\boldsymbol{\eta}_0 = \mathbf{X} \boldsymbol{\beta}_0$  and for some integer  $k, t \in [q]$ , define  $\mathbf{x}_i^t$  as

$$\mathbf{x}_i^t = \begin{cases} \left[ \boldsymbol{\eta}_{0,i}, 0, \mathbf{R}_i^0, 0, \mathbf{R}_i^1, 0, \dots, \mathbf{R}_i^{\frac{t-1}{2}}, 0, 0, \dots \right]^\top & \text{if } t = 2k + 1, i \in [n] \\ \mathbf{0}_q & \text{if } t = 2k + 1, i \in [N] \setminus [n] \\ \mathbf{0}_q & \text{if } t = 2k, i \in [n] \\ \left[ 0, \boldsymbol{\nu}_{i-n}^1, 0, \boldsymbol{\nu}_{i-n}^2, \dots, \boldsymbol{\nu}_{i-n}^{\frac{t}{2}}, 0, 0, \dots \right]^\top & \text{if } t = 2k, i \in [N] \setminus [n] \end{cases} \quad (\text{S22})$$

Finally, let  $y \in \mathcal{V}_{N,q}$  have vectors  $\mathbf{y}_i \in \mathbb{R}^q$ ,  $i = 1, \dots, N$ , such that

$$\mathbf{y}_i(k) = \begin{cases} \bar{\varepsilon}_i & \text{if } i \in [n], k = 1 \\ \boldsymbol{\beta}_{0,i-n} & \text{if } i \in [N] \setminus [n], k = 1 \\ \boldsymbol{\nu}_{i-n}^0 & \text{if } i \in [N] \setminus [n], k = 2 \\ 0 & \text{else} \end{cases} \quad (\text{S23})$$

That is,  $y$  can be seen as the  $q \times N$  matrix

$$y = \begin{bmatrix} \bar{\varepsilon}_1 & \bar{\varepsilon}_2 & \dots & \bar{\varepsilon}_n & \boldsymbol{\beta}_{0,1} & \boldsymbol{\beta}_{0,2} & \dots & \boldsymbol{\beta}_{0,p} \\ 0 & 0 & \dots & 0 & \boldsymbol{\nu}_1^0 & \boldsymbol{\nu}_2^0 & \dots & \boldsymbol{\nu}_p^0 \\ 0 & & & & \dots & & & 0 \\ \vdots & & & & \ddots & & & \vdots \\ 0 & & & & \dots & & & 0 \end{bmatrix}$$

It is now possible to define an AMP-orbit corresponding to the above AMP instance, which is subject of the next two Lemmas. For this, note from Definition 2, equation (S7), that the  $i$ th component of an AMP

orbit  $\{x^t\}_{t \in \mathbb{N}}$  for an AMP instance  $(\mathbf{A}, \mathcal{F}, x^0)$  is given by

$$\mathbf{x}_i^t = \sum_{j=1}^N \mathbf{A}_{ij} f^j(\mathbf{x}_j^{t-1}, t-1) - \frac{1}{N} \left\{ \sum_{j=1}^N \frac{\partial}{\partial \mathbf{x}} f^j(\mathbf{x}, t-1) \Big|_{\mathbf{x}=\mathbf{x}_j^{t-1}} \right\} f^i(\mathbf{x}_i^{t-2}, t-2). \quad (\text{S24})$$

**Lemma B.1.** Consider the symmetric AMP instance  $(\mathbf{A}, \mathcal{F}, x^0)$  defined by (S19), (S20), (S21) and  $x^0 = 0_{N,q}$  and the iterates  $\{x^t\}_{t \in [q]}$ , the entries of which are defined in (S22) and (S12)-(S15). Then, for  $t \in [q]$  being even, and  $i \in [N] \setminus [n]$  and  $t \in [q]$  odd with  $i \in [n]$ , these iterates satisfy the recursion of (S24).

*Proof.* The proof follows from strong induction on  $t$  for even and odd iterates and straightforward algebra.

*Base case (i):*  $t = 1, i \in [n]$ . Note that by construction

$$\begin{aligned} \sum_{j=1}^N \mathbf{A}_{ij} f^j(\mathbf{x}_j^0, 0) &= \sum_{j=n+1}^{n+p} \mathbf{A}_{ij} f^j(\mathbf{x}_j^0, 0) \\ &= \sqrt{\frac{n}{N}} \sum_{j=1}^p \mathbf{X}_{ij} f^{j+n}(\mathbf{x}_{j+n}^0, 0) \\ &= \sum_{j=1}^p \mathbf{X}_{ij} [\mathbf{y}_{j+n}(1), 0, \mathbf{y}_{j+n}(2) + \mu_0 \mathbf{y}_{j+n}(1), 0, 0, \dots]^\top \\ &= \sum_{j=1}^p \mathbf{X}_{ij} [\beta_{0,j}, 0, \boldsymbol{\nu}_j^0 + \mu_0 \beta_{0,j}, 0, 0, \dots]^\top \\ &= \sum_{j=1}^p \mathbf{X}_{ij} [\beta_{0,j}, 0, \hat{\beta}_j^0 - \mu_0 \beta_{0,j} + \mu_0 \beta_{0,j}, 0, 0, \dots]^\top \\ &= \left[ \sum_{j=1}^p \mathbf{X}_{ij} \beta_{0,j}, 0, \sum_{j=1}^p \mathbf{X}_{ij} \hat{\beta}_j^0, 0, 0, \dots \right]^\top \\ &= [\boldsymbol{\eta}_{0,i}, 0, \mathbf{R}_i^0, 0, 0, \dots]^\top \\ &= \mathbf{x}_i^1, \end{aligned} \quad (\text{S25})$$

The first equality follows from the definition of (S21), the second from the definition of (S19), the third again from (S21), the fourth from (S23), the fifth and seventh from the definition of  $\boldsymbol{\nu}^0, \mathbf{R}^0$  above (S12) and since  $\boldsymbol{\eta}_0 = \mathbf{X} \beta_0$  and the last from (S22). Concordance with the full recursion of (S24) follows since  $f^i(\mathbf{x}_i^{-1}, -1) = \mathbf{0}_q$  by definition.

*Base case (ii):*  $t = 2, i \in [N] \setminus [n]$ . Again it is easily checked that

$$\begin{aligned} \sum_{j=1}^N \mathbf{A}_{ij} f^j(\mathbf{x}_j^1, 1) &= \sum_{j=1}^n \mathbf{A}_{ij} f^j(\mathbf{x}_j^1, 1) \\ &= \sqrt{\frac{N}{n}} \sum_{j=1}^n \mathbf{X}_{ji} f^j(\mathbf{x}_j^1, 1) \\ &= \kappa^{-1} \sum_{j=1}^n \mathbf{X}_{ji} [0, \Psi^0(h(\mathbf{x}_j^1(1), y_j(1)), \mathbf{x}_j^1(3)), 0, 0, \dots]^\top \\ &= \kappa^{-1} \sum_{j=1}^n \mathbf{X}_{ji} [0, \Psi^0(h(\boldsymbol{\eta}_{0,j}, \bar{\varepsilon}_j), \mathbf{R}_j^0), 0, 0, \dots]^\top, \end{aligned} \quad (\text{S26})$$

where the first equality comes from (S20), the second and third from (S19), the fourth again from (S20) and the last from (S25). Now recalling that  $y_i^* = h(\boldsymbol{\eta}_{0,i}, \bar{\varepsilon}_i)$  for  $h(Z, \bar{\varepsilon}) = \alpha \{1 - \text{sign}(\bar{\varepsilon} - \zeta'(Z))\} / 2 + (1 - \alpha)/2$ , it immediately follows that the nonzero element in the last line of (S26) corresponds to the  $i$ th entry of  $\kappa^{-1} \mathbf{X}^\top \Psi^0(\mathbf{y}^*, \mathbf{R}^0)$ .

Next consider

$$\begin{aligned} \sum_{j=1}^N \frac{\partial}{\partial \mathbf{x}} f^j(\mathbf{x}, 1) \Big|_{\mathbf{x}=\mathbf{x}_j^1} &= \sum_{j=1}^n \frac{\partial}{\partial \mathbf{x}} f^j(\mathbf{x}, 1) \Big|_{\mathbf{x}=\mathbf{x}_j^1} \\ &= \kappa^{-1} \sqrt{\frac{N}{n}} \sum_{j=1}^n [0, \frac{\partial}{\partial \mathbf{x}} \Psi^0(h(\mathbf{x}(1), \mathbf{y}(1)), \mathbf{x}(3)), 0, 0, \dots]^\top \Big|_{\mathbf{x}=\mathbf{x}_j^1} \\ &= \kappa^{-1} \sqrt{\frac{N}{n}} \sum_{j=1}^n \begin{bmatrix} 0 & 0 & \dots & 0 & 0 & \dots \\ \frac{\partial}{\partial Z} \Psi^0(h(Z, \bar{\varepsilon}_j), \mathbf{R}_j^0) \Big|_{Z=\boldsymbol{\eta}_{0,j}} & 0 & \frac{\partial}{\partial R} \Psi^0(y_j^*, R) \Big|_{R=\mathbf{R}_j^0} & 0 & 0 & \dots \\ 0 & 0 & \dots & & & \\ \vdots & \ddots & & & & \end{bmatrix}, \end{aligned} \quad (\text{S27})$$

where the first two equalities follow from (S20) and the last from straightforward differentiation and  $\mathbf{x}^1$  from (S25).

Finally, it immediately follows from (S21) that

$$\begin{aligned} f^i(\mathbf{x}_i^0, 0) &= \sqrt{\frac{N}{n}} [\mathbf{y}_i(1), 0, \mathbf{y}_i(2) + \mu_0 \mathbf{y}_i(1), 0, 0, \dots]^\top \\ &= \sqrt{\frac{N}{n}} [\boldsymbol{\beta}_{0,i-n}, 0, \boldsymbol{\nu}_{i-n}^0 + \mu_0 \boldsymbol{\beta}_{0,i-n}, 0, 0, \dots]^\top \end{aligned} \quad (\text{S28})$$

so that (S27) and (S28) yield

$$\begin{aligned} & -\frac{1}{N} \left\{ \sum_{j=1}^N \frac{\partial}{\partial \mathbf{x}} f^j(\mathbf{x}, 1) \Big|_{\mathbf{x}=\mathbf{x}_j^1} \right\} f^i(\mathbf{x}_i^0, 0) \\ &= -\frac{1}{n\kappa} \begin{bmatrix} 0 & 0 & \dots & 0 & 0 & \dots \\ \sum_{j=1}^n \frac{\partial}{\partial Z} \Psi^0(h(Z, \bar{\varepsilon}_j), \mathbf{R}_j^0) \Big|_{Z=\boldsymbol{\eta}_{0,j}} & 0 & \sum_{j=1}^n \frac{\partial}{\partial R} \Psi^0(y_j^*, R) \Big|_{R=\mathbf{R}_j^0} & 0 & 0 & \dots \\ 0 & 0 & \dots & & & \\ \vdots & \ddots & & & & \end{bmatrix} \begin{bmatrix} \boldsymbol{\beta}_{0,i-n} \\ 0 \\ \boldsymbol{\nu}_{i-n}^0 + \mu_0 \boldsymbol{\beta}_{0,i-n} \\ 0 \\ 0 \\ \vdots \end{bmatrix} \\ &= \left[ 0, \left\{ -\frac{1}{n\kappa} \sum_{j=1}^n \frac{\partial}{\partial Z} \Psi^0(h(Z, \bar{\varepsilon}_j), \mathbf{R}_j^0) \Big|_{Z=\boldsymbol{\eta}_{0,j}} \right\} \boldsymbol{\beta}_{0,i-n} + \left\{ -\frac{1}{n\kappa} \sum_{j=1}^n \frac{\partial}{\partial R} \Psi^0(y_j^*, R) \Big|_{R=\mathbf{R}_j^0} \right\} (\boldsymbol{\nu}_{i-n}^0 + \mu_0 \boldsymbol{\beta}_{0,i-n}), 0, 0, \dots \right] \\ &= [0, -a_1 \boldsymbol{\beta}_{0,i-n} + q_0 (\boldsymbol{\nu}_{i-n}^0 + \mu_0 \boldsymbol{\beta}_{0,i-n}), 0, 0, \dots]^\top, \quad (\text{S29}) \end{aligned}$$

Hence, from (S26), (S29) and (S12), (S14), (S15), it follows that the second entry of (S24) equals

$$\kappa^{-1} \sum_{j=1}^n \mathbf{X}_{ji} \Psi^0(h(\boldsymbol{\eta}_{0,j}, \bar{\varepsilon}_j), \mathbf{R}_j^0) - a_1 \boldsymbol{\beta}_{0,i-n} + q_0 (\boldsymbol{\nu}_{i-n}^0 + \mu_0 \boldsymbol{\beta}_{0,i-n}) = \boldsymbol{\nu}_{i-n}^1,$$

while all other entries are zero. Hence, by construction of (S22) the second base case holds.

*Induction hypothesis:* Assume that there exists some  $t < q$ ,  $t \geq 2$  such that for all  $t' \leq t$  if  $t'$  is even, and  $i \in [N] \setminus [n]$  or if  $t'$  is odd with  $i \in [n]$ , the iterates of (S22) satisfy the recursion of (S24).

*Induction step (i):*  $t + 1$  odd,  $i \in [n]$ . Most derivations are analogous to Base case (i), so that details are skipped on repetitive steps. First note that due to the nested nature of the iterates  $\mathbf{x}_i^t$  in (S22) and the induction hypothesis, the induction step must only be established for the last nonzero entry in  $\mathbf{x}_j^{t+1}$ .

For this, note that

$$\sum_{j=1}^N \mathbf{A}_{ij} f^j(\mathbf{x}_j^t, t) = \sum_{j=1}^p \mathbf{X}_{ij} \left[ \beta_{0,j}, 0, \nu_j^0 + \mu_0 \beta_{0,j}, 0, \nu_j^1 + \mu_1 \beta_{0,j}, 0, \dots, \nu_j^{\frac{t}{2}} + \mu_{\frac{t}{2}} \beta_{0,j}, 0, 0, \dots \right]^\top. \quad (\text{S30})$$

Next, it is easily seen that

$$\begin{aligned} \sqrt{\frac{n}{N}} \sum_{j=1}^N \frac{\partial}{\partial \mathbf{x}} f^j(\mathbf{x}, t) \Big|_{\mathbf{x}=\mathbf{x}_j^t} &= \sqrt{\frac{n}{N}} \sum_{j=1}^p \frac{\partial}{\partial \mathbf{x}} f^{n+j}(\mathbf{x}, t) \Big|_{\mathbf{x}=\mathbf{x}_{n+j}^t} \\ &= \sum_{j=1}^p \frac{\partial}{\partial \mathbf{x}} \left[ \mathbf{y}_i(1), 0, \mathbf{y}_i(2) + \mu_0 \mathbf{y}_i(1), 0, \mathbf{x}(2) + \mu_1 \mathbf{y}_i(1), 0, \mathbf{x}(4) + \mu_2 \mathbf{y}_i(1), 0, \dots, \mathbf{x}(t) + \mu_{\frac{t}{2}} \mathbf{y}_i(1), 0, \dots \right]^\top \Big|_{\mathbf{x}=\mathbf{x}_{n+j}^t} \\ &= \sum_{j=1}^p \tilde{I}_{q \times q} = p \tilde{I}_{q \times q}, \quad (\text{S31}) \end{aligned}$$

where  $\tilde{I}_{q \times q}$  whose odd rows with row index  $5 \leq i \leq t + 3$  have the  $(i - 3)$ rd element equal to one, while all other elements of this matrix are equal to zero.

Further, note that for  $t + 1$  odd,  $i \in [n]$ ,

$$\kappa \sqrt{\frac{n}{N}} f^i(\mathbf{x}_i^{t-1}, t - 1) = \begin{bmatrix} 0 \\ \Psi^0(h(\mathbf{x}_i^{t-1}(1), \mathbf{y}_i(1)), \mathbf{x}_i^{t-1}(3)) \\ 0 \\ \Psi^1(h(\mathbf{x}_i^{t-1}(1), \mathbf{y}_i(1)), \mathbf{x}_i^{t-1}(5)) \\ 0 \\ \vdots \\ \Psi^{\frac{t-2}{2}}(h(\mathbf{x}_i^{t-1}(1), \mathbf{y}_i(1)), \mathbf{x}_i^{t-1}(t+1)) \\ 0 \\ \vdots \end{bmatrix} = \begin{bmatrix} 0 \\ \Psi^0(h(\boldsymbol{\eta}_{0,i}, \bar{\varepsilon}_i), \mathbf{R}_i^0) \\ 0 \\ \Psi^1(h(\boldsymbol{\eta}_{0,i}, \bar{\varepsilon}_i), \mathbf{R}_i^1) \\ 0 \\ \vdots \\ \Psi^{\frac{t}{2}-1}(h(\boldsymbol{\eta}_{0,i}, \bar{\varepsilon}_i), \mathbf{R}_i^{\frac{t}{2}-1}) \\ 0 \\ \vdots \end{bmatrix}, \quad (\text{S32})$$

by definition of (S21), (S22) and (S23). Hence, from (S31) and (S32), it follows that

$$-\frac{1}{N} \left\{ \sum_{j=1}^N \frac{\partial}{\partial \mathbf{x}} f^j(\mathbf{x}, t) \Big|_{\mathbf{x}=\mathbf{x}_j^t} \right\} f^i(\mathbf{x}_i^{t-1}, t - 1) = -\kappa^{-1} \frac{p}{n} \begin{bmatrix} 0 \\ 0 \\ 0 \\ 0 \\ \Psi^0(h(\boldsymbol{\eta}_{0,i}, \bar{\varepsilon}_i), \mathbf{R}_i^0) \\ 0 \\ \Psi^1(h(\boldsymbol{\eta}_{0,i}, \bar{\varepsilon}_i), \mathbf{R}_i^1) \\ 0 \\ \vdots \\ \Psi^{\frac{t}{2}-1}(h(\boldsymbol{\eta}_{0,i}, \bar{\varepsilon}_i), \mathbf{R}_i^{\frac{t}{2}-1}) \\ 0 \\ \vdots \end{bmatrix},$$

Hence, it follows from equations (S30) and (S30), that the last nonzero entry of

$$\sum_{j=1}^N \mathbf{A}_{ij} f^j(\mathbf{x}_j^t, t) - \frac{1}{N} \left\{ \sum_{j=1}^N \frac{\partial}{\partial \mathbf{x}} f^j(\mathbf{x}, t) \Big|_{\mathbf{x}=\mathbf{x}_j^t} \right\} f^i(\mathbf{x}_i^{t-1}, t-1)$$

is given by

$$\sum_{j=1}^p \mathbf{X}_{ij} \left( \nu_j^{\frac{t}{2}} + \mu_{\frac{t}{2}} \beta_{0,j} \right) - \Psi^{\frac{t}{2}-1} \left( h(\boldsymbol{\eta}_{0,i}, \bar{\varepsilon}_i), \mathbf{R}^{\frac{t}{2}-1} \right),$$

which by (S13) corresponds to the  $i$ th entry of  $\mathbf{R}^{\frac{t}{2}}$  and that corresponds precisely to the last nonzero entry of  $\mathbf{x}_i^{t+1}$  as defined in (S22). This establishes the first part of the induction step.

*Induction step (ii):*  $t+1$  even,  $i \in [N] \setminus [n]$ . This step is completely analogous to base case (ii) and therefore omitted.

By strong induction, the claim of the Lemma holds for any  $t \in [q]$ .  $\square$

With this result it is possible to fill up the missing parts the incomplete recursion of Lemma B.1. Hence, define iterate  $\tilde{\mathbf{x}}^t$  as follows. Let  $\tilde{\mathbf{x}}^0 = 0_{N,q}$  and for  $t \in [q]$  odd and  $i \in [n]$  or if  $t$  is even and  $i \in [N] \setminus [n]$ , set  $\tilde{\mathbf{x}}_i^t = \mathbf{x}_i^t$ . Otherwise, let

$$\tilde{\mathbf{x}}_i^t = \sum_{j=1}^N \mathbf{A}_{ij} f^j(\tilde{\mathbf{x}}_j^{t-1}, t-1) - \frac{1}{N} \left\{ \sum_{j=1}^N \frac{\partial}{\partial \mathbf{x}} f^j(\tilde{\mathbf{x}}, t-1) \Big|_{\tilde{\mathbf{x}}=\tilde{\mathbf{x}}_j^{t-1}} \right\} f^i(\tilde{\mathbf{x}}_i^{t-2}, t-2), \quad (\text{S33})$$

again with the convention that terms involving negative  $t$ -indices are zero. The Lemma below establishes that this recursion is indeed a AMP orbit corresponding to instance  $(\mathbf{A}, \mathcal{F}, \tilde{\mathbf{x}}^0)$  and that the orbit of interest, i.e. the iterates of Lemma B.1, are preserved.

**Lemma B.2.** *Given the AMP instance  $(\mathbf{A}, \mathcal{F}, \tilde{\mathbf{x}}^0)$  of Lemma B.1, the recursion of (S33) is an orbit according to Definition 2. Further, for  $t \in [q]$  odd and  $i \in [n]$  or if  $t$  is even and  $i \in [N] \setminus [n]$ , the iterates  $\tilde{\mathbf{x}}_i^t$  correspond to those in Lemma B.1.*

*Proof.* The statement of the Lemma is shown by strong induction on  $t$ .

*Base case (i):*  $t = 1$ . Since  $\tilde{\mathbf{x}}^0 = \mathbf{x}^0 = 0_{n,q}$ , by base case (i) of Lemma B.1, the second part of the Lemma holds for  $t = 1$ . For  $i \in [n]$ , the first part of the claim follows from base case (i) of Lemma B.1 too, while for  $i \in [N] \setminus [n]$  it follows trivially from (S33).

*Base case (ii):*  $t = 2$ . Again, note that by the base case (ii) in Lemma B.1, the claim of the Lemma immediately follows for  $i \in [N] \setminus [n]$ . For  $i \in [n]$ , the second part of the Lemma follows from (S33).

*Induction hypothesis:* The claim of the Lemma holds for all  $t'$  up to some  $t < q$ ,  $t \geq 2$ .

*Induction step (i):*  $t+1$  odd. Consider  $i \in [n]$ . From the induction hypothesis, one has that  $\tilde{\mathbf{x}}_j^t = \mathbf{x}_j^t$  for  $i \in [N] \setminus [n]$  and similarly  $\tilde{\mathbf{x}}_j^{t-1} = \mathbf{x}_j^{t-1}$  for  $i \in [n]$ . Hence again, the corresponding induction step of Lemma B.1 shows that the recursion is an orbit according to Definition 2 and that the iterates  $\tilde{\mathbf{x}}_i^t$  correspond to those in Lemma B.1. Now consider  $i \in [N] \setminus [n]$ . The induction step holds trivially by construction of (S33).

*Induction step (ii):*  $t+1$  even. This case is handled similarly to induction step (i) and is therefore omitted.

By strong induction, the Lemma is proven for all  $t \in [q]$ .  $\square$

Hence, if  $(\mathbf{A}, \mathcal{F}, \tilde{\mathbf{x}}^0)$  were shown to be a converging AMP instance according to Definition 3, then Theorem B.1 along with the state evolution of Definition 4, would give the large sample behaviour of the corresponding orbit of interest. However, as remarked in Feng *et al.* (2022), Section 4.7, the function  $g$  in Definition 3 cannot be Lipschitz, which is owed to the indicator function  $h(Z, \bar{\varepsilon})$ , so that Theorem B.1 does not apply. The next section deals with this technicality.

#### B.4.4 A smooth approximation

This section introduces a smooth approximation to the original recursions (S10)-(S11) and to (S12)-(S15), the latter of which can be used in a matrix-valued AMP embedding for which Theorem B.1 applies. A limiting argument then shows that the theorem still applies in the limit where the smooth approximation approaches the nonsmooth original recursion.

In particular, the step function  $\{1 - \text{sign}(x)\}/2$  can, amongst others, be approximated by  $\left\{1 - \frac{x}{|x|+\epsilon}\right\}/2$  for some positive constant  $\epsilon$ . Note that defining the Bernoulli response  $Y = \{1 - \text{sign}(\bar{\epsilon} - \zeta'(Z))\}/2$  rather than the more conventional  $Y = \mathbb{1}\{\bar{\epsilon} < \zeta'(Z)\}$  comes without loss of generality, as per the modelling assumption,  $\boldsymbol{\eta}_{0,i}$  are independent  $N(0, \gamma^2)$  normal random variables and  $\bar{\epsilon}_i$  are independent of  $\boldsymbol{\eta}_0$  and uniformly distributed on the unit interval so that the event  $\{\exists i \in [n] : \bar{\epsilon}_i = \zeta'(\boldsymbol{\eta}_{0,i})\}$  has measure zero.

Hence, in what follows, denote by  $h_\epsilon(Z, \bar{\epsilon})$  the function

$$h_\epsilon(Z, \bar{\epsilon}) = \frac{\alpha}{2} \left\{ 1 - \frac{\bar{\epsilon} - \zeta'(Z)}{|\bar{\epsilon} - \zeta'(Z)| + \epsilon} \right\} + \frac{1 - \alpha}{2}.$$

Consequently, define new sets of recursions analogous to (S10)-(S11) and (S12)-(S15) where all appearances of  $h(\cdot, \cdot)$  are replaced by  $h_\epsilon(\cdot, \cdot)$ . In particular, define the approximate target AMP recursion with initial conditions  $\hat{\boldsymbol{\beta}}^0, \mathbf{S}^0 = \mathbf{X}\hat{\boldsymbol{\beta}}^0$ , and a sequence of constants  $\{\epsilon\mu_t, \epsilon b_t, \epsilon\sigma_t\}_{t \in \mathbb{N}_0}$ , for  $t \in \mathbb{N}$ , as

$$\epsilon\hat{\boldsymbol{\beta}}^t = \epsilon\hat{\boldsymbol{\beta}}^{t-1} + \kappa^{-1} \mathbf{X}^\top \Psi^{t-1}(\epsilon\mathbf{y}^*, \epsilon\mathbf{S}^{t-1}) \quad (\text{S34})$$

$$\epsilon\mathbf{S}^t = \mathbf{X}_\epsilon \hat{\boldsymbol{\beta}}^t - \Psi^{t-1}(\epsilon\mathbf{y}^*, \epsilon\mathbf{S}^{t-1}), \quad (\text{S35})$$

where  $\Psi^t(\epsilon\mathbf{y}^*, \epsilon\mathbf{S}^t)$  acts elementwise on  $\epsilon\mathbf{y}^*, \epsilon\mathbf{S}^t$  as

$$\Psi^t(\epsilon y_i^*, \epsilon \mathbf{S}_i^t) = \epsilon b_t \left\{ \epsilon y_i^* - \zeta'(\text{prox}_{\epsilon b_t \zeta}(\epsilon b_t y_i^* + \epsilon \mathbf{S}_i^t)) \right\},$$

for  $i = 1, \dots, n$  and where  $\epsilon y_i^* = \alpha h_\epsilon(\boldsymbol{\eta}_{0,i}, \bar{\epsilon}_i) + (1 - \alpha)/2$ . Further, the state evolution is determined by the system of nonlinear equations

$$1 - \kappa = \mathbb{E} \left[ \frac{1}{1 + \epsilon b_t \zeta''(\text{prox}_{\epsilon b_t \zeta}(\epsilon b_t Y^* + \epsilon Z_t))} \right] \quad (\text{S36})$$

$$\epsilon\mu_{t+1} = \frac{\epsilon b_t}{\kappa \gamma^2} \mathbb{E} [Z \{ \epsilon Y^* - \zeta'(\text{prox}_{\epsilon b_t \zeta}(\epsilon b_t Y^* + \epsilon Z_t)) \}] + \epsilon\mu_t \quad (\text{S37})$$

$$\epsilon\sigma_{t+1}^2 = \frac{\epsilon b_t^2}{\kappa^2} \mathbb{E} \left[ \{ \epsilon Y^* - \zeta'(\text{prox}_{\epsilon b_t \zeta}(\epsilon b_t Y^* + \epsilon Z_t)) \}^2 \right], \quad (\text{S38})$$

for independent  $Z, \tilde{Z} \sim N(0, \gamma^2)$ ,  $G \sim N(0, 1)$ , and  $\bar{\epsilon} \sim U(0, 1)$ , and letting

$$\epsilon Y^* = h_\epsilon(Z, \bar{\epsilon}), \quad \epsilon Z_t = \epsilon\mu_t Z + \kappa^{1/2} \epsilon\sigma_t G.$$

Given initial conditions  $\boldsymbol{\nu}^0 = \hat{\boldsymbol{\beta}}^0 - \mu_0 \boldsymbol{\beta}_0$ ,  $\mathbf{R}^0 = \mathbf{S}^0$  for  $\hat{\boldsymbol{\beta}}^0, \boldsymbol{\beta}_0 \in \mathbb{R}^p$ ,  $\mu_0 \in \mathbb{R}$  and  $\mathbf{S}^0 \in \mathbb{R}^n$ , for  $t \in \mathbb{N}$ , the approximate centred recursion of (S12)-(S15) is defined as

$$\epsilon\boldsymbol{\nu}^t = \epsilon q_{t-1}(\epsilon\boldsymbol{\nu}^{t-1} + \epsilon\mu_{t-1}\boldsymbol{\beta}_0) - \epsilon a_t \boldsymbol{\beta}_0 + \kappa^{-1} \mathbf{X}^\top \Psi^{t-1}(\epsilon\mathbf{y}^*, \epsilon\mathbf{R}^{t-1}) \quad (\text{S39})$$

$$\epsilon\mathbf{R}^t = \mathbf{X}(\epsilon\boldsymbol{\nu}^t + \epsilon\mu_t \boldsymbol{\beta}_0) - \Psi^{t-1}(\epsilon\mathbf{y}^*, \epsilon\mathbf{R}^{t-1}), \quad (\text{S40})$$

where  $a_0 = \mu_0$  and for  $t \in \mathbb{N}$ ,

$$\begin{aligned} \epsilon q_t &= -\frac{1}{\kappa n} \sum_{i=1}^n \frac{\partial \Psi^t}{\partial R}(\epsilon y_i^*, R) \Big|_{R=\epsilon \mathbf{R}_i^t} \\ \epsilon a_t &= \frac{1}{\kappa n} \sum_{i=1}^n \frac{\partial \Psi^{t-1}}{\partial Z}(h_\epsilon(Z, \bar{\epsilon}_i), \epsilon \mathbf{R}_i^{t-1}) \Big|_{Z=\mathbf{x}_i^\top \boldsymbol{\beta}_0}, \end{aligned} \quad (\text{S41})$$

where  $\bar{\varepsilon}_i \sim U(0, 1)$  ( $i = 1, \dots, n$ ) are i.i.d. draws independent of all other random variables.

Similarly, define  $f_\epsilon^i(\mathbf{x}, t)$  as functions (S20) and (S21) with  $h(Z, \bar{\varepsilon})$  replaced by  $h_\epsilon(Z, \bar{\varepsilon})$  and denote by  ${}_\epsilon \mathbf{x}_i^t$  the orbit of (S22) whose definition is unchanged but whose entries now depend on  $\epsilon$  through the replacement of  $h(\cdot, \cdot)$  by  $h_\epsilon(\cdot, \cdot)$  in (S12)-(S15). Finally, denote by  ${}_\epsilon \tilde{\mathbf{x}}_i^t$  the corresponding full AMP recursion as defined in (S33) with  $\mathbf{x}_i^t$  replaced by  ${}_\epsilon \mathbf{x}_i^t$ . Completely analogous to Lemmas B.1 and B.2, it can be shown that  ${}_\epsilon \mathbf{x}_i^t$  is a AMP orbit to the AMP instance  $(\mathbf{A}, \mathcal{F}_\epsilon, \tilde{\mathbf{x}}^0)$ , where the definition of  $\mathbf{A}$  remains unchanged,  $\mathcal{F}_\epsilon$  is the collection of functions  $f_\epsilon^i$  and  $\tilde{\mathbf{x}}^0 = \mathbf{0}_{q,N}$  as before. This is easily verified by noting that the proofs of these Lemmas do not depend on the form of the indicator function but are concerned with the general structure of the recursion.

It remains to construct a converging AMP instance following Definition 3 to motivate Theorem B.1. Following the structure of Definition 3,

- i) Let  $q$  be some arbitrarily large integer, and  $q' = 2$
- ii) Define  $g_\epsilon : \mathbb{R}^q \times \mathbb{R}^q \times [q'] \times \mathbb{N} \rightarrow \mathbb{R}^q$  as follows. Given  $k \in \mathbb{N}_0$ ,

$$\begin{aligned} & g_\epsilon(\mathbf{x}, \mathbf{y}, 1, 2k+1) \\ &= \kappa^{-1} \sqrt{\frac{N}{n}} \left[ 0, \Psi^0(h_\epsilon(\mathbf{x}(1), \mathbf{y}(1)), \mathbf{x}(3)), 0, \Psi^1(h_\epsilon(\mathbf{x}(1), \mathbf{y}(1)), \mathbf{x}(5)), \dots, \Psi^{\frac{t-1}{2}}(h_\epsilon(\mathbf{x}(1), \mathbf{y}(1)), \mathbf{x}(t+2)), 0, 0, \dots \right]^\top, \end{aligned} \quad (\text{S42})$$

and

$$\begin{aligned} & g_\epsilon(\mathbf{x}, \mathbf{y}, 2, 2k) \\ &= \sqrt{\frac{N}{n}} \left[ \mathbf{y}(1), 0, \mathbf{y}(2) + \mu_0 \mathbf{y}(1), 0, \mathbf{x}(2) + \mu_1 \mathbf{y}(1), 0, \mathbf{x}(4) + \mu_2 \mathbf{y}(1), 0, \dots, \mathbf{x}(t) + \mu_{\frac{t}{2}} \mathbf{y}(1), 0, 0, \dots \right]^\top, \end{aligned} \quad (\text{S43})$$

while for all other configurations of  $t, a$ ,  $g_\epsilon(\mathbf{x}, \mathbf{y}, a, t) = \mathbf{0}_q$ .

- iii) Let  $\pi_{\bar{\beta}}$  be the probability distribution such that the empirical distribution of  $\beta_0$  converges weakly to  $\pi_{\bar{\beta}}$ , which is assumed to exist. Further, given initial conditions  $\hat{\beta}^0, \mu_0$ , let  $\pi_{\bar{\nu}}$  be the probability distribution such that the empirical distribution of  $\nu^0 = \hat{\beta}^0 - \mu_0 \beta_0$  converges weakly to, which is also assumed to exist, such as the joint distribution  $\pi_{\bar{\beta}, \bar{\nu}}$  which is the limit of the joint distribution of  $\beta_0, \nu^0$ . Finally, let  $\pi_{\bar{\varepsilon}}$  be the distribution of a  $U(0, 1)$  random variable. Then let  $P_1$  be the distribution of  $q$  independent random variables whose marginals are  $\pi_{\bar{\varepsilon}}$  for the first coordinate and point masses at zero for all others. Further, let  $P_2$  be the distribution of  $q$  random variables whose first two coordinates are distributed according to  $\pi_{\bar{\beta}, \bar{\nu}}$  and are independent of all other coordinates, whose distributions are independent of another and point masses at zero.
- iv) For  $N = n + p$ , partition  $[N]$  into  $C_1^N = [n]$  and  $C_2^N = [N] \setminus [n]$
- v) For  $a = 1, 2$ , let

$$\hat{\Sigma}_a^0 = \text{plim}_{N \rightarrow \infty} \frac{1}{|C_a^N|} \sum_{i \in C_a^N} g_\epsilon(\mathbf{0}_q, \mathbf{y}_i, a, 0) g_\epsilon(\mathbf{0}_q, \mathbf{y}_i, a, 0)^\top,$$

which is assumed to exist. Here,  $c_1 = \lim_{N \rightarrow \infty} n/(n+p) = 1/(1+\kappa)$  and  $c_2 = \lim_{N \rightarrow \infty} p/(n+p) = \kappa/(1+\kappa)$  in concordance with Definition 3 1).

Condition iii) appears a bit abstract in its stated generality. For initial condition of relevance in this paper, namely the oracle initialiser  $\mu_* \beta_0 + \sigma_* \xi$ , where  $\xi \sim \mathcal{N}(\mathbf{I}_p)$  independent of everything else, it is readily seen that the condition holds whenever the empirical distribution of  $\beta_0$  converges to some distribution  $\pi_{\bar{\beta}}$ .

To conclude the definition, it must now be shown that for all  $r \in [q]$ , the  $r$ th component of  $g_\epsilon(\cdot, \cdot, a, t)$  is Lipschitz in its first two arguments and that points 1)-3) of Definition 3 hold. This is subject of the Lemma below.

**Lemma B.3.** *The AMP instance defined above is a converging AMP instance according to Definition 3.*

*Proof.* It must be shown that 0) each component of  $g_\epsilon(\cdot, \cdot, a, t)$  is Lipschitz in its first two arguments and that points 1)-3) of Definition 3 hold. Each point is shown separately.

0) *Lipschitzianity of  $g_\epsilon(\cdot, \cdot, a, t)$ :* It is shown in Lemma G.2 ii) that  $\Psi^{\frac{t-1}{2}}(h_\epsilon(\mathbf{x}(1), \mathbf{y}(1)), \mathbf{x}(t+2))$  is Lipschitz in  $[\mathbf{x}(1), \mathbf{x}(t+2), \mathbf{y}(1)]^\top$ . Hence by (S42), for any  $k \in \mathbb{N}_0$ ,  $a = 1$ ,  $r \in [q]$ , the  $r$ th component of  $g_\epsilon(\cdot, \cdot, 1, 2k+1)$  is Lipschitz. On the other hand, by (S43), Lipschitzianity of  $g_\epsilon(\cdot, \cdot, 2, 2k)$  is immediate since it is an affine transformation of its arguments. For all other combinations of  $t, a$ ,  $g_\epsilon(\cdot, \cdot, a, t) = \mathbf{0}_q$  and thus trivially Lipschitz.

1) *Convergence of  $|C_a^N|/N$ :* By definition of  $N = n + p$ , and  $C_N^1 = [n]$ ,  $C_N^2 = [N] \setminus [n]$ . Hence, since by assumption,  $\kappa(N) = p/n$  converges to some  $\kappa \in (0, 1)$ , 1) holds.

2): Agreement of  $f_\epsilon^i$  with the  $i$ th component of  $g_\epsilon$  holds by construction of  $y$  in (S23),  $f_\epsilon^i$  in (S20), (S21),  $g_\epsilon$  in (S42) and (S43) along with the partition  $C_N^1, C_N^2$ . Convergence of the empirical distribution of  $\{\mathbf{y}_i\}_{i \in C_N^a}$  to  $P_a$  follows by definition of  $P_a$ .

3) *Initial condition of state evolution:* Follows by assumption v).  $\square$

It thus follows from Lemma B.2 applied to the smooth approximation  ${}_\epsilon \tilde{\mathbf{x}}_i^t$  and Lemma B.3 that  $(\mathbf{A}, \mathcal{F}_\epsilon, \tilde{x}^0)$  along with iterates  ${}_\epsilon \tilde{\mathbf{x}}_i^t$  is a converging AMP instance and Theorem B.1 applies.

**Theorem B.2.** *Under assumptions (i)-(v), for any pseudo Lipschitz-function of order 2, and for all  $t \in [q]$ ,  $a = 1, 2$ , almost surely*

$$\lim_{N \rightarrow \infty} \frac{1}{|C_a^N|} \sum_{i \in C_a^N} \psi({}_\epsilon \tilde{\mathbf{x}}_i^t, \mathbf{y}) = E[\psi({}_\epsilon Z_a^t, Y_a)] ,$$

where  ${}_\epsilon Z_a^t \sim N(0, {}_\epsilon \Sigma^t)$ , and  ${}_\epsilon \Sigma^t$  denotes the covariance matrices from state evolution (S8) and (S9) with function  $g_\epsilon(\mathbf{x}, \mathbf{y}, a, t)$

*Proof.* By Lemma B.3 and Theorem B.1, for any pseudo Lipschitz function  $\psi$  of order 2,

$$\lim_{N \rightarrow \infty} \frac{1}{|C_a^N|} \sum_{i \in C_a^N} \psi({}_\epsilon \tilde{\mathbf{x}}_i^t, \mathbf{y}) = E[\psi({}_\epsilon Z_a^t, Y_a)] ,$$

where  ${}_\epsilon Z_a^t \sim N(0, {}_\epsilon \Sigma^t)$  as defined in the statement of the Theorem.  $\square$

**Corollary B.2.1.** *Under assumptions (i)-(v), and initial conditions  $\hat{\beta}^0$ ,*

$$\begin{aligned} {}_\epsilon \mu_0 &= \frac{1}{\gamma^2} \lim_{n \rightarrow \infty} \frac{\langle \hat{\beta}^0, \beta_0 \rangle}{n} \\ {}_\epsilon \sigma_0^2 &= \lim_{n \rightarrow \infty} \frac{\left\| \hat{\beta}^0 - \mu_0 \beta_0 \right\|_2^2}{p} , \end{aligned}$$

for any pseudo Lipschitz-function of order 2, and for all  $t \in [q]$ , almost surely

$$\lim_{N \rightarrow \infty} \frac{1}{p} \sum_{j=1}^p \psi({}_\epsilon \nu_j^t, \beta_{0,j}) = E[\psi({}_\epsilon \sigma_t^2 G, \bar{\beta})] , \quad \lim_{N \rightarrow \infty} \frac{1}{n} \sum_{j=1}^n \psi \left( \begin{bmatrix} \eta_{0,j} \\ {}_\epsilon \mathbf{R}_i^t \end{bmatrix}, \begin{bmatrix} \bar{\varepsilon}_j \\ 0 \end{bmatrix} \right) = E \left[ \psi \left( \begin{bmatrix} Z_1^t \\ {}_\epsilon Z_2^t \end{bmatrix}, \begin{bmatrix} \bar{\varepsilon} \\ 0 \end{bmatrix} \right) \right] ,$$

where  $G \sim N(0, 1)$ ,  $Z_1^t \sim N(0, \gamma^2)$ ,  ${}_\epsilon Z_2^t = {}_\epsilon \mu_t Z_1^t + \kappa^{1/2} {}_\epsilon \sigma_t G$ ,  $G \sim N(0, 1)$ ,  $\bar{\epsilon} \sim U(0, 1)$  and where  $G \perp \bar{\beta}$ ,  $G \perp Z_1^t$  and  $(Z_1^t, {}_\epsilon Z_2^t) \perp \bar{\epsilon}$ .

*Proof.* The proof consists of two parts, which shall be shown in turn: i) For fixed  $\epsilon > 0$ , extract the iterates  ${}_\epsilon \boldsymbol{\nu}^t, {}_\epsilon \mathbf{R}^t$  of (S39) and (S40) from  ${}_\epsilon \tilde{\mathbf{x}}_i^t$  and obtain their asymptotic variances according to Theorem B.2, and ii) relate these variances to the state evolution of (S36)-(S38).

The first step is similar to the derivations in the proof of Lemma 6 in the supplementary material of Sur and Candès (2019). For  $t = 1$ , it is easily seen from the AMP instance defined in B.4.4 and the state evolutions (S8) and (S9) that

$$\begin{bmatrix} {}_\epsilon \boldsymbol{\Sigma}_{1,1}^1 & {}_\epsilon \boldsymbol{\Sigma}_{1,3}^1 \\ {}_\epsilon \boldsymbol{\Sigma}_{3,1}^1 & {}_\epsilon \boldsymbol{\Sigma}_{3,3}^1 \end{bmatrix} = \begin{bmatrix} \lim_{N \rightarrow \infty} \frac{\|\boldsymbol{\beta}_0\|_2^2}{n} & \lim_{N \rightarrow \infty} \frac{\langle \hat{\boldsymbol{\beta}}^0, \boldsymbol{\beta}_0 \rangle}{n} \\ \lim_{N \rightarrow \infty} \frac{\langle \hat{\boldsymbol{\beta}}^0, \boldsymbol{\beta}_0 \rangle}{n} & \lim_{N \rightarrow \infty} \frac{\|\hat{\boldsymbol{\beta}}^0\|_2^2}{n} \end{bmatrix}, \quad (\text{S44})$$

where  ${}_\epsilon \boldsymbol{\Sigma}_{i,j}^1$  denotes the  $j$ th entry in the  $i$ th row of  ${}_\epsilon \boldsymbol{\Sigma}^1$ . All other entries of  ${}_\epsilon \boldsymbol{\Sigma}^1$  are zero. Now from (S22) it follows that for  $i \in [n]$ , the first and third entries of  ${}_\epsilon \tilde{\mathbf{x}}_i^1$  are  $\boldsymbol{\eta}_{0,i}$ ,  ${}_\epsilon \mathbf{R}_i^0 = \mathbf{x}_i^\top \hat{\boldsymbol{\beta}}^0$ . Hence, by Theorem B.2,

$$\lim_{N \rightarrow \infty} \frac{1}{n} \sum_{j=1}^n \psi \left( \begin{bmatrix} \boldsymbol{\eta}_{0,j} \\ {}_\epsilon \mathbf{R}_i^0 \end{bmatrix}, \begin{bmatrix} \bar{\epsilon}_j \\ 0 \end{bmatrix} \right) = \mathbb{E} \left[ \psi \left( \mathbf{Z}^1, \begin{bmatrix} \bar{\epsilon} \\ 0 \end{bmatrix} \right) \right],$$

where  $\mathbf{Z}^1 = [\mathbf{Z}_1^1, \mathbf{Z}_2^1]^\top \perp \bar{\epsilon}$  is bivariate normal with mean zero and covariance (S44).

Next, the only nonzero entry of  ${}_\epsilon \boldsymbol{\Sigma}^2$  is readily computed as  $\kappa^{-2} \mathbb{E} \left[ \left\{ \Psi^0(h_\epsilon(\mathbf{Z}_1^1, \bar{\epsilon}), \mathbf{Z}_2^1) \right\}^2 \right]$ . By construction of  ${}_\epsilon \tilde{\mathbf{x}}_i^t$  it follows from (S22) and Lemma B.3 and Theorem B.1 that almost surely

$$\lim_{N \rightarrow \infty} \frac{1}{p} \sum_{j=1}^p \psi({}_\epsilon \boldsymbol{\nu}_j^1, \boldsymbol{\beta}_{0,j}) = \mathbb{E} \left[ \psi({}_\epsilon \tau_1^2 G, \bar{\beta}) \right],$$

where  ${}_\epsilon \tau_1^2 = \kappa^{-2} \mathbb{E} \left[ \left\{ \Psi^0(h_\epsilon(\mathbf{Z}_1^1, \bar{\epsilon}), \mathbf{Z}_2^1) \right\}^2 \right]$  and  $G \sim N(0, 1) \perp \bar{\beta}$ . Next consider  ${}_\epsilon \boldsymbol{\Sigma}^3$ . By the nested nature of the iterates  ${}_\epsilon \mathbf{x}_i^t$ , it follows that the first  $3 \times 3$  principal submatrix is exactly the one given in (S44). Further, it is readily verified that the remaining nonzero entries are given by

$${}_\epsilon \boldsymbol{\Sigma}_{1,5}^3 = {}_\epsilon \mu_1 \gamma^2, \quad {}_\epsilon \boldsymbol{\Sigma}_{3,5}^3 = {}_\epsilon \mu_1 \lim_{N \rightarrow \infty} \frac{\langle \hat{\boldsymbol{\beta}}^0, \boldsymbol{\beta}_0 \rangle}{n}, \quad {}_\epsilon \boldsymbol{\Sigma}_{5,5}^3 = {}_\epsilon \tau_1^2 \kappa + {}_\epsilon \mu_1^2 \gamma^2,$$

where  ${}_\epsilon \mu_1$  comes from recursion (S37) with initial condition  $\mu_0$ . Again, Lemma B.2 and Theorem B.1 yield almost surely

$$\lim_{N \rightarrow \infty} \frac{1}{n} \sum_{j=1}^n \psi \left( \begin{bmatrix} \boldsymbol{\eta}_{0,j} \\ {}_\epsilon \mathbf{R}_j^0 \\ {}_\epsilon \mathbf{R}_j^1 \end{bmatrix}, \begin{bmatrix} \bar{\epsilon}_j \\ 0 \\ 0 \end{bmatrix} \right) = \mathbb{E} \left[ \psi \left( \mathbf{Z}^3, \begin{bmatrix} \bar{\epsilon} \\ 0 \\ 0 \end{bmatrix} \right) \right],$$

where  $\mathbf{Z}^3 = [\mathbf{Z}_1^3, \mathbf{Z}_2^3, \mathbf{Z}_3^3]^\top \perp \bar{\epsilon}$  is trivariate normal with mean zero and covariance matrix

$$\begin{bmatrix} {}_\epsilon \boldsymbol{\Sigma}_{1,1}^3 & {}_\epsilon \boldsymbol{\Sigma}_{1,3}^3 & {}_\epsilon \boldsymbol{\Sigma}_{1,5}^3 \\ {}_\epsilon \boldsymbol{\Sigma}_{3,1}^3 & {}_\epsilon \boldsymbol{\Sigma}_{3,3}^3 & {}_\epsilon \boldsymbol{\Sigma}_{3,5}^3 \\ {}_\epsilon \boldsymbol{\Sigma}_{5,1}^3 & {}_\epsilon \boldsymbol{\Sigma}_{5,3}^3 & {}_\epsilon \boldsymbol{\Sigma}_{5,5}^3 \end{bmatrix} = \begin{bmatrix} \lim_{N \rightarrow \infty} \frac{\|\boldsymbol{\beta}_0\|_2^2}{n} & \lim_{N \rightarrow \infty} \frac{\langle \hat{\boldsymbol{\beta}}^0, \boldsymbol{\beta}_0 \rangle}{n} & {}_\epsilon \mu_1 \gamma^2 \\ \lim_{N \rightarrow \infty} \frac{\langle \hat{\boldsymbol{\beta}}^0, \boldsymbol{\beta}_0 \rangle}{n} & \lim_{N \rightarrow \infty} \frac{\|\hat{\boldsymbol{\beta}}^0\|_2^2}{n} & {}_\epsilon \mu_1 \lim_{N \rightarrow \infty} \frac{\langle \hat{\boldsymbol{\beta}}^0, \boldsymbol{\beta}_0 \rangle}{n} \\ {}_\epsilon \mu_1 \gamma^2 & {}_\epsilon \mu_1 \lim_{N \rightarrow \infty} \frac{\langle \hat{\boldsymbol{\beta}}^0, \boldsymbol{\beta}_0 \rangle}{n} & {}_\epsilon \tau_1^2 \kappa + {}_\epsilon \mu_1^2 \gamma^2 \end{bmatrix}.$$

Calculating the nonzero entries of  ${}_{\epsilon}\Sigma^4$  yields that

$$\begin{bmatrix} {}_{\epsilon}\Sigma_{2,2}^4 & {}_{\epsilon}\Sigma_{2,4}^4 \\ {}_{\epsilon}\Sigma_{4,2}^4 & {}_{\epsilon}\Sigma_{4,4}^4 \end{bmatrix} = \begin{bmatrix} {}_{\epsilon}\tau_1^2 & {}_{\epsilon}\rho_{1,2} \\ {}_{\epsilon}\rho_{1,2} & {}_{\epsilon}\tau_2^2 \end{bmatrix}, \quad (\text{S45})$$

where

$$\begin{aligned} {}_{\epsilon}\tau_2^2 &= \kappa^{-2} \mathbb{E} [\{\Psi^1(h_{\epsilon}(\mathbf{Z}_1^3, \bar{\epsilon}), \mathbf{Z}_2^3)\}^2] \\ {}_{\epsilon}\rho_{1,2} &= \kappa^{-2} \mathbb{E} [\Psi^0(h_{\epsilon}(\mathbf{Z}_1^3, \bar{\epsilon}), \mathbf{Z}_2^3) \Psi^1(h_{\epsilon}(\mathbf{Z}_1^3, \bar{\epsilon}), \mathbf{Z}_3^3)]. \end{aligned}$$

Consequently, almost surely

$$\lim_{N \rightarrow \infty} \frac{1}{p} \sum_{j=1}^p \psi \left( \begin{bmatrix} {}_{\epsilon}\nu_j^1 \\ {}_{\epsilon}\nu_j^2 \end{bmatrix}, \begin{bmatrix} \beta_{0,j} \\ 0 \end{bmatrix} \right) = \mathbb{E} \left[ \psi \left( \mathbf{Z}^4, \begin{bmatrix} \bar{\beta} \\ 0 \end{bmatrix} \right) \right],$$

where  $\mathbf{Z}^4 = [\mathbf{Z}_1^4, \mathbf{Z}_2^4]^{\top}$  is bivariate normal with mean zero and covariance matrix (S45). Iterating further,

$$\begin{bmatrix} {}_{\epsilon}\Sigma_{1,1}^5 & {}_{\epsilon}\Sigma_{1,3}^5 & {}_{\epsilon}\Sigma_{1,5}^5 & {}_{\epsilon}\Sigma_{1,7}^5 \\ {}_{\epsilon}\Sigma_{3,1}^5 & {}_{\epsilon}\Sigma_{3,3}^5 & {}_{\epsilon}\Sigma_{3,5}^5 & {}_{\epsilon}\Sigma_{3,7}^5 \\ {}_{\epsilon}\Sigma_{5,1}^5 & {}_{\epsilon}\Sigma_{5,3}^5 & {}_{\epsilon}\Sigma_{5,5}^5 & {}_{\epsilon}\Sigma_{5,7}^5 \\ {}_{\epsilon}\Sigma_{7,1}^5 & {}_{\epsilon}\Sigma_{7,3}^5 & {}_{\epsilon}\Sigma_{7,5}^5 & {}_{\epsilon}\Sigma_{7,7}^5 \end{bmatrix} = \begin{bmatrix} \lim_{N \rightarrow \infty} \frac{\|\beta_0\|_2^2}{n} & \lim_{N \rightarrow \infty} \frac{\langle \hat{\beta}^0, \beta_0 \rangle}{n} & {}_{\epsilon}\mu_1 \gamma^2 & {}_{\epsilon}\mu_2 \gamma^2 \\ \lim_{N \rightarrow \infty} \frac{\langle \hat{\beta}^0, \beta_0 \rangle}{n} & \lim_{N \rightarrow \infty} \frac{\|\hat{\beta}^0\|_2^2}{n} & {}_{\epsilon}\mu_1 \lim_{N \rightarrow \infty} \frac{\langle \hat{\beta}^0, \beta_0 \rangle}{n} & {}_{\epsilon}\mu_2 \lim_{N \rightarrow \infty} \frac{\langle \hat{\beta}^0, \beta_0 \rangle}{n} \\ {}_{\epsilon}\mu_1 \gamma^2 & {}_{\epsilon}\mu_1 \lim_{N \rightarrow \infty} \frac{\langle \hat{\beta}^0, \beta_0 \rangle}{n} & {}_{\epsilon}\tau_1^2 \kappa + {}_{\epsilon}\mu_1^2 \gamma^2 & {}_{\epsilon}\rho_{1,2} \kappa + {}_{\epsilon}\mu_1 {}_{\epsilon}\mu_2 \gamma^2 \\ {}_{\epsilon}\mu_2 \gamma^2 & {}_{\epsilon}\mu_2 \lim_{N \rightarrow \infty} \frac{\langle \hat{\beta}^0, \beta_0 \rangle}{n} & {}_{\epsilon}\rho_{1,2} \kappa + {}_{\epsilon}\mu_1 {}_{\epsilon}\mu_2 \gamma^2 & {}_{\epsilon}\tau_2^2 \kappa + {}_{\epsilon}\mu_2^2 \gamma^2 \end{bmatrix}, \quad (\text{S46})$$

so that almost surely

$$\lim_{N \rightarrow \infty} \frac{1}{n} \sum_{j=1}^n \psi \left( \begin{bmatrix} \eta_{0,j} \\ {}_{\epsilon}\mathbf{R}_j^0 \\ {}_{\epsilon}\mathbf{R}_j^1 \\ {}_{\epsilon}\mathbf{R}_j^2 \end{bmatrix}, \begin{bmatrix} \bar{\epsilon}_i \\ 0 \\ 0 \\ 0 \end{bmatrix} \right) = \mathbb{E} \left[ \psi \left( \mathbf{Z}^5, \begin{bmatrix} \bar{\epsilon} \\ 0 \\ 0 \\ 0 \end{bmatrix} \right) \right],$$

where once again  $\mathbf{Z}^5 = [\mathbf{Z}_1^5, \dots, \mathbf{Z}_4^5]^{\top} \perp \bar{\epsilon}$  is multivariate normal with mean zero and covariance matrix (S46). Hence continuing,

$$\begin{bmatrix} {}_{\epsilon}\Sigma_{2,2}^6 & {}_{\epsilon}\Sigma_{2,4}^6 & {}_{\epsilon}\Sigma_{2,6}^6 \\ {}_{\epsilon}\Sigma_{4,2}^6 & {}_{\epsilon}\Sigma_{4,4}^6 & {}_{\epsilon}\Sigma_{4,6}^6 \\ {}_{\epsilon}\Sigma_{6,2}^6 & {}_{\epsilon}\Sigma_{6,4}^6 & {}_{\epsilon}\Sigma_{6,6}^6 \end{bmatrix} = \begin{bmatrix} {}_{\epsilon}\tau_1^2 & {}_{\epsilon}\rho_{1,2} & {}_{\epsilon}\rho_{1,3} \\ {}_{\epsilon}\rho_{1,2} & {}_{\epsilon}\tau_2^2 & {}_{\epsilon}\rho_{2,3} \\ {}_{\epsilon}\rho_{1,3} & {}_{\epsilon}\rho_{2,3} & {}_{\epsilon}\tau_3^2 \end{bmatrix}, \quad (\text{S47})$$

where

$$\begin{aligned} {}_{\epsilon}\tau_3^2 &= \kappa^{-2} \mathbb{E} [\{\Psi^2(h_{\epsilon}(\mathbf{Z}_1^5, \bar{\epsilon}), \mathbf{Z}_2^5)\}^2] \\ {}_{\epsilon}\rho_{l,m} &= \kappa^{-2} \mathbb{E} [\Psi^{l-1}(h_{\epsilon}(\mathbf{Z}_1^5, \bar{\epsilon}), \mathbf{Z}_{l+1}^5) \Psi^{m-1}(h_{\epsilon}(\mathbf{Z}_1^5, \bar{\epsilon}), \mathbf{Z}_{m+1}^5)]. \end{aligned}$$

Therefore almost surely,

$$\lim_{N \rightarrow \infty} \frac{1}{p} \sum_{j=1}^p \psi \left( \begin{bmatrix} {}_{\epsilon}\nu_j^1 \\ {}_{\epsilon}\nu_j^2 \\ {}_{\epsilon}\nu_j^3 \end{bmatrix}, \begin{bmatrix} \beta_{0,j} \\ 0 \\ 0 \end{bmatrix} \right) = \mathbb{E} \left[ \psi \left( \mathbf{Z}^6, \begin{bmatrix} \bar{\beta} \\ 0 \\ 0 \end{bmatrix} \right) \right],$$

with  $\mathbf{Z}^6 = [\mathbf{Z}_1^6, \mathbf{Z}_2^6, \mathbf{Z}_3^6]^{\top}$  trivariate normal with mean zero and covariance (S47). Continuing in this

vein, one gets that for all  $t \in [q]$ , by Lemmas B.2 and Theorem B.1, almost surely

$$\begin{aligned} \lim_{N \rightarrow \infty} \frac{1}{p} \sum_{j=1}^p \psi(\epsilon \nu_j^t, \beta_{0,j}) &= \mathbb{E}[\psi(\tau_t G, \bar{\beta})] \\ \lim_{N \rightarrow \infty} \frac{1}{n} \sum_{j=1}^n \psi\left(\begin{bmatrix} \eta_{0,j} \\ \epsilon \mathbf{R}_j^t \end{bmatrix}, \begin{bmatrix} \bar{\epsilon}_i \\ 0 \end{bmatrix}\right) &= \mathbb{E}\left[\psi\left(\begin{bmatrix} \mathbf{Z}_t^{2t+1} \\ \mathbf{Z}_{t+2}^{2t+1} \end{bmatrix}, \begin{bmatrix} \bar{\epsilon} \\ 0 \end{bmatrix}\right)\right], \end{aligned} \quad (\text{S48})$$

where  $G \sim \mathcal{N}(0, 1) \perp \bar{\beta}$ , and  $(\mathbf{Z}_t^{2t+1}, \mathbf{Z}_{t+2}^{2t+1}) \perp \bar{\epsilon}$  are bivariate normal with mean zero and covariance

$$\begin{bmatrix} \epsilon \Sigma_{1,1}^{t+2} & \epsilon \Sigma_{1,t+2}^{t+2} \\ \epsilon \Sigma_{t+2,1}^{t+2} & \epsilon \Sigma_{t+2,t+2}^{t+2} \end{bmatrix} = \begin{bmatrix} \lim_{N \rightarrow \infty} \frac{\|\beta_0\|_2^2}{n} & \epsilon \mu_t \gamma^2 \\ \epsilon \mu_t \gamma^2 & \epsilon \tau_t^2 \kappa + \epsilon \mu_t^2 \gamma^2 \end{bmatrix}, \quad (\text{S49})$$

and

$$\epsilon \tau_t = \kappa^{-2} \mathbb{E} \left[ \left\{ \Psi^{t-1}(h_\epsilon(\mathbf{Z}_1^{2t-1}, \bar{\epsilon}), \mathbf{Z}_{t+1}^{2t-1}) \right\}^2 \right], \quad (\text{S50})$$

and where  $\mathbf{Z}_1^{2t-1}, \mathbf{Z}_{t+1}^{2t-1} \perp \bar{\epsilon}$  are bivariate normal with the covariance structure of (S49) with  $\epsilon \mu_{t-1}, \epsilon \tau_{t-1}$  in place of  $\epsilon \mu_t, \epsilon \tau_t$  respectively.

Next, note that with initialisations  $\epsilon \mu_0 = \gamma^{-2} \lim_{n \rightarrow \infty} \langle \hat{\beta}^0, \beta_0 \rangle / n$  and  $\epsilon \sigma_0^2 = \lim_{n \rightarrow \infty} \|\hat{\beta}^0 - \mu_0 \beta_0\|_2^2 / p$ , the variances of (S44) correspond to

$$\begin{bmatrix} \gamma^2 & \epsilon \mu_0 \gamma^2 \\ \epsilon \mu_0 \gamma^2 & \epsilon \sigma_0^2 \kappa + \epsilon \mu_0^2 \gamma^2 \end{bmatrix},$$

Hence by the definition of  $\epsilon \sigma_t$  in (S38),  $\epsilon \tau_1 = \epsilon \sigma_1$ . By induction it follows that  $\epsilon \tau_t = \epsilon \sigma_t$  for all  $t$  under consideration. This concludes the proof.  $\square$

#### B.4.5 Asymptotic equivalence of target and centred AMP

Next it is possible to establish the asymptotic equivalence of the centred recursion (S12)-(S15) with the initial target recursion (S10)-(S11) for appropriately centred iterates. The proof closely follows along the proof of Lemma 4 of the supplementary material of Sur and Candès (2019) which in turn is an adaptation of the proof of Lemma 6.7 of Donoho and Montanari (2016).

**Lemma B.4.** *In the setting of Corollary B.2.1, it holds that for initial conditions  $\epsilon \nu^0 = \hat{\beta}^0 - \mu_0 \beta_0$ ,  $\epsilon \mathbf{R}^0 = \epsilon \mathbf{S}^0$ ,  $t \in [q]$ ,*

$$\lim_{N \rightarrow \infty} \frac{1}{p} \left\| \epsilon \nu^t - \epsilon \hat{\beta}^t - \epsilon \mu_t \beta_0 \right\|_2^2 = 0, \quad \lim_{N \rightarrow \infty} \frac{1}{n} \left\| \epsilon \mathbf{R}^t - \epsilon \mathbf{S}^t \right\|_2^2 = 0,$$

*almost surely.*

*Proof.* To facilitate notation, let  $\epsilon \theta^t = \epsilon \hat{\beta}^t - \epsilon \mu_t \beta_0$ . Then by construction of recursions (S10)-(S11) and (S12)-(S13), and the triangle inequality it holds that

$$\begin{aligned} \left\| \epsilon \mathbf{R}^t - \epsilon \mathbf{S}^t \right\|_2 &\leq \left\| \mathbf{X} \right\|_2 \left\| \epsilon \nu^t - \epsilon \theta^t \right\|_2 + \left\| \Psi^{t-1}(\epsilon \mathbf{y}^*, \epsilon \mathbf{R}^{t-1}) - \Psi^{t-1}(\epsilon \mathbf{y}^*, \epsilon \mathbf{S}^{t-1}) \right\| \\ &\leq \left\| \mathbf{X} \right\|_2 \left\| \epsilon \nu^t - \epsilon \theta^t \right\|_2 + \left\| \epsilon \mathbf{R}^{t-1} - \epsilon \mathbf{S}^{t-1} \right\|_2, \end{aligned} \quad (\text{S51})$$

where the second inequality follows by Lemma G.2 iii) and where  $\epsilon \mathbf{y}^* = \alpha h_\epsilon(\eta_0, \bar{\epsilon}) + (1 - \alpha)/2$ .

Similarly,

$$\|\epsilon \boldsymbol{\nu}^t - \epsilon \boldsymbol{\theta}^t\|_2 \leq \|\epsilon \boldsymbol{\nu}^{t-1} - \epsilon \boldsymbol{\theta}^{t-1}\|_2 + |\epsilon q_{t-1} - 1| \|\epsilon \boldsymbol{\nu}^{t-1} + \epsilon \mu_{t-1} \boldsymbol{\beta}_0\|_2 + \|\epsilon \mu_t - \epsilon a_t\| \|\boldsymbol{\beta}_0\| + \frac{1}{\kappa} \|\mathbf{X}\|_2 \|\epsilon \mathbf{R}^{t-1} - \epsilon \mathbf{S}^{t-1}\|_2.$$

Now since  $\epsilon \boldsymbol{\nu}^0 = \epsilon \boldsymbol{\theta}^0$ , an induction argument on the number of iterations  $t$  gives that there exists a constant  $C$ , which may depend on  $\kappa$ , such that for each  $t \in [q]$ ,

$$\|\epsilon \boldsymbol{\nu}^t - \epsilon \boldsymbol{\theta}^t\|_2 \leq (C \|\mathbf{X}\|_2)^{2t} \left( \sum_{l=1}^{t-1} |\epsilon q_l - 1| \|\epsilon \boldsymbol{\nu}^l + \epsilon \mu_l \boldsymbol{\beta}_0\|_2 + \sum_{l=0}^{t-1} |\epsilon \mu_l - a_l| \|\boldsymbol{\beta}_0\|_2 \right). \quad (\text{S52})$$

Recalling that  $\epsilon q_t = -\frac{1}{\kappa n} \sum_{j=1}^n \frac{-b_t \zeta''(\text{prox}_{b_t \zeta}(b_t h_\epsilon(\boldsymbol{\eta}_{0,j}, \bar{\epsilon}_j), \mathbf{R}_j^t))}{1 + b_t \zeta''(\text{prox}_{b_t \zeta}(b_t h_\epsilon(\boldsymbol{\eta}_{0,j}, \bar{\epsilon}_j), \mathbf{R}_j^t))}$  (cf. (S14) and (S90)), it follows from Lemma G.2 iv) and Corollary B.2.1 i), that almost surely

$$\lim_{N \rightarrow \infty} \epsilon q_t = \frac{1}{\kappa} \mathbb{E} \left[ \frac{b_t \zeta''(\text{prox}_{b_t \zeta}(b_t h_\epsilon(Z_1^t, \bar{\epsilon}), \epsilon Z_2^t))}{1 + b_t \zeta''(\text{prox}_{b_t \zeta}(b_t h_\epsilon(Z_1^t, \bar{\epsilon}), \epsilon Z_2^t))} \right] \quad (\text{S53})$$

for  $Z_1^t \sim N(0, \gamma^2)$ ,  $\epsilon Z_2^t = \epsilon \mu_t Z_1^t + \kappa^{1/2} \epsilon \sigma_t G$ ,  $G \sim N(0, 1)$ ,  $\bar{\epsilon} \sim U(0, 1)$  and where  $G \perp \bar{\beta}$ ,  $G \perp Z_1^t$  and  $(Z_1^t, \epsilon Z_2^t) \perp \bar{\epsilon}$ . Now the right hand side of (S53) can be rearranged as

$$\frac{1}{\kappa} \mathbb{E} \left[ \frac{b_t \zeta''(\text{prox}_{b_t \zeta}(b_t h_\epsilon(Z_1^t, \bar{\epsilon}), \epsilon Z_2^t))}{1 + b_t \zeta''(\text{prox}_{b_t \zeta}(b_t h_\epsilon(Z_1^t, \bar{\epsilon}), \epsilon Z_2^t))} \right] = \frac{1}{\kappa} \mathbb{E} \left[ 1 - \frac{1}{b_t \zeta''(\text{prox}_{b_t \zeta}(b_t h_\epsilon(Z_1^t, \bar{\epsilon}), \epsilon Z_2^t))} \right] = 1,$$

according to state evolution equation (S36).

Again, by Corollary B.2.1 i) and  $\psi(u, v) = u^2$ , it follows that almost surely,

$$\lim_{N \rightarrow \infty} \sum_{j=1}^n (\epsilon \boldsymbol{\nu}_j^t)^2 = \mathbb{E} [(\epsilon \sigma_t Z)^2] < \infty,$$

for  $Z \sim N(0, 1)$ . Further recall that by assumption  $\lim_{n \rightarrow \infty} \|\boldsymbol{\beta}_0\|_2^2/n = \gamma^2$  and that by Lemma G.3,  $\lim_{N \rightarrow \infty} \|\mathbf{X}\|_2 < \infty$  almost surely. Hence it holds almost surely that

$$\lim_{N \rightarrow \infty} \frac{1}{\sqrt{p}} (C \|\mathbf{X}\|_2)^{2t} \sum_{l=0}^{t-1} |\epsilon q_l - 1| \|\epsilon \boldsymbol{\nu}_j^l + \epsilon \mu_l \boldsymbol{\beta}_0\|_2 = 0. \quad (\text{S54})$$

Similarly, recalling the definition of  $\epsilon a_t$  in (S41) and invoking Lemma G.2 iv) and Corollary B.2.1 equation (S48), almost surely

$$\lim_{N \rightarrow \infty} \epsilon a_t = \frac{1}{\kappa} \mathbb{E} \left[ \frac{\partial}{\partial Z} \Psi^{t-1}(h_\epsilon(Z, \bar{\epsilon}), \epsilon Z_2^t) \Big|_{Z=Z_1^t} \right], \quad (\text{S55})$$

for  $Z_1^t \sim N(0, \gamma^2)$ ,  $\epsilon Z_2^t = \epsilon \mu_t Z_1^t + \kappa^{1/2} \epsilon \sigma_t G$ ,  $G \sim N(0, 1)$ ,  $\bar{\epsilon} \sim U(0, 1)$  and where  $G \perp \bar{\beta}$ ,  $G \perp Z_1^t$  and  $(Z_1^t, \epsilon Z_2^t) \perp \bar{\epsilon}$ .

To compute the expectation in (S55), Stein's Lemma (Stein, 1981, Lemma 1) shall prove useful. It states that for a normal random variable  $z \sim N(\mu, \sigma^2)$ , and a differentiable function  $h(z)$ ,  $\mathbb{E}[h(z)(z - \mu)] = \sigma^2 \mathbb{E}(h'(z))$ , where  $h$  is derivative of  $h$  with respect to  $z$ .

To use the Lemma, first note that  ${}_{\epsilon}Z_2^t$  is a function of  $Z_1^t$ . Hence write  ${}_{\epsilon}Z_2^t = t_{\epsilon}(Z_1^t, G_t) = {}_{\epsilon}\mu_t Z_1^t + \kappa^{1/2} {}_{\epsilon}\sigma_t G_t$ . Then conditioning on both  $\bar{\epsilon}, G_t$ , one gets that

$$\mathbb{E} \left[ \frac{\partial}{\partial Z} \Psi^{t-1}(h_{\epsilon}(Z, \bar{\epsilon}), {}_{\epsilon}Z_2^t) \Big|_{Z=Z_1^t} \right] = \mathbb{E}_{G_t, \bar{\epsilon}} \left\{ \mathbb{E}_{Z_1^t} \left[ \frac{\partial}{\partial Z} \Psi(h_{\epsilon}(Z, \bar{\epsilon}), s) \Big|_{\substack{Z=Z_1^t, \\ s=t_{\epsilon}(Z_1^t, G_t)}} \Big| G_t, \bar{\epsilon} \right] \right\}. \quad (\text{S56})$$

Now since  $Z_1^t$  is independent of  $G_t, \bar{\epsilon}$ , the conditional distribution of  $Z_1^t$  given  $G_t, \bar{\epsilon}$  is its unconditional distribution, i.e.  $Z_1^t|_{G_t, \bar{\epsilon}} \sim N(0, \gamma^2)$  and thus by Stein's Lemma,

$$\gamma^2 \mathbb{E}_{Z_1^t} \left[ \frac{\partial}{\partial Z_1^t} \Psi(h_{\epsilon}(Z_1^t, \bar{\epsilon}), t_{\epsilon}(Z_1^t, G_t)) \Big| G_t, \bar{\epsilon} \right] = \mathbb{E}_{Z_1^t} \left[ Z_1^t \Psi(h_{\epsilon}(Z_1^t, \bar{\epsilon}), t_{\epsilon}(Z_1^t, G_t)) \Big| G_t, \bar{\epsilon} \right]. \quad (\text{S57})$$

Now an application of the chain rule to the left hand side of (S57) yields

$$\begin{aligned} \mathbb{E}_{Z_1^t} \left[ \frac{\partial}{\partial Z_1^t} \Psi(h_{\epsilon}(Z_1^t, \bar{\epsilon}), t_{\epsilon}(Z_1^t, G_t)) \Big| G_t, \bar{\epsilon} \right] &= \mathbb{E}_{Z_1^t} \left[ \frac{\partial}{\partial Z} \Psi(h_{\epsilon}(Z, \bar{\epsilon}), s) \Big|_{\substack{Z=Z_1^t, \\ s=t_{\epsilon}(Z_1^t, G_t)}} \Big| G_t, \bar{\epsilon} \right] \\ &\quad + {}_{\epsilon}\mu_{t-1} \mathbb{E}_{Z_1^t} \left[ \frac{\partial}{\partial s} \Psi(h_{\epsilon}(Z, \bar{\epsilon}), s) \Big|_{\substack{Z=Z_1^t, \\ s=t_{\epsilon}(Z_1^t, G_t)}} \Big| G_t, \bar{\epsilon} \right] \end{aligned} \quad (\text{S58})$$

Combining (S57) and (S58) gives

$$\begin{aligned} \mathbb{E}_{Z_1^t} \left[ \frac{\partial}{\partial Z} \Psi(h_{\epsilon}(Z, \bar{\epsilon}), s) \Big|_{\substack{Z=Z_1^t, \\ s=t_{\epsilon}(Z_1^t, G_t)}} \Big| G_t, \bar{\epsilon} \right] &= \frac{1}{\gamma^2} \mathbb{E}_{Z_1^t} \left[ Z_1^t \Psi(h_{\epsilon}(Z_1^t, \bar{\epsilon}), t_{\epsilon}(Z_1^t, G_t)) \Big| G_t, \bar{\epsilon} \right] \\ &\quad - {}_{\epsilon}\mu_{t-1} \mathbb{E}_{Z_1^t} \left[ \frac{\partial}{\partial s} \Psi(h_{\epsilon}(Z, \bar{\epsilon}), s) \Big|_{\substack{Z=Z_1^t, \\ s=t_{\epsilon}(Z_1^t, G_t)}} \Big| G_t, \bar{\epsilon} \right] \end{aligned}$$

Substituting back onto (S56) in conjunction with (S55) gives that almost surely,

$$\lim_{N \rightarrow \infty} {}_{\epsilon}a_t = \frac{1}{\kappa \gamma^2} \mathbb{E} \left[ Z_1^t \Psi(h_{\epsilon}(Z_1^t, \bar{\epsilon}), {}_{\epsilon}Z_2^t) \right] - \frac{{}_{\epsilon}\mu_{t-1}}{\kappa} \mathbb{E} \left[ \frac{\partial}{\partial s} \Psi(h_{\epsilon}(Z, \bar{\epsilon}), s) \Big|_{\substack{Z=Z_1^t, \\ s={}_{\epsilon}Z_2^t}} \right].$$

Now using (S36) and (S90), it follows that

$$\begin{aligned} -\frac{1}{\kappa} \mathbb{E} \left[ \frac{\partial}{\partial s} \Psi(h_{\epsilon}(Z, \bar{\epsilon}), s) \Big|_{\substack{Z=Z_1^t, \\ s={}_{\epsilon}Z_2^t}} \right] &= \frac{1}{\kappa} \mathbb{E} \left[ \frac{b\zeta''(\text{prox}_{b\zeta}(bh_{\epsilon}(Z, \bar{\epsilon}) + {}_{\epsilon}Z_2^t))}{1 + b\zeta''(\text{prox}_{b\zeta}(bh_{\epsilon}(Z, \bar{\epsilon}) + {}_{\epsilon}Z_2^t))} \right] \\ &= \frac{1}{\kappa} \mathbb{E} \left[ 1 - \frac{1}{1 + b\zeta''(\text{prox}_{b\zeta}(bh_{\epsilon}(Z, \bar{\epsilon}) + {}_{\epsilon}Z_2^t))} \right] \\ &= 1. \end{aligned}$$

Hence, the state evolution of  ${}_{\epsilon}\mu_t$  as specified in (S37) gives that almost surely

$$\begin{aligned}\lim_{N \rightarrow \infty} {}_{\epsilon}a_t &= \frac{1}{\kappa\gamma^2} \mathbb{E} [Z_1^t \Psi(h_{\epsilon}(Z_1^t, \bar{\epsilon}), {}_{\epsilon}Z_2^t)] - \frac{{}_{\epsilon}\mu_{t-1}}{\kappa} \mathbb{E} \left[ \frac{\partial}{\partial s} \Psi(h_{\epsilon}(Z, \bar{\epsilon}), s) \Big|_{\substack{Z=Z_1^t, \\ s={}_{\epsilon}Z_2^t}} \right] \\ &= \frac{1}{\kappa\gamma^2} \mathbb{E} [Z_1^t \Psi(h_{\epsilon}(Z_1^t, \bar{\epsilon}), {}_{\epsilon}Z_2^t)] + {}_{\epsilon}\mu_{t-1} \\ &= {}_{\epsilon}\mu_t.\end{aligned}\tag{S59}$$

Hence, for any  $l \in \mathbb{N}_0$ ,  $\lim_{N \rightarrow \infty} |{}_{\epsilon}a_t - {}_{\epsilon}\mu_t| = 0$  almost surely. By almost sure boundedness of  $\mathbf{X}$  and since  $\|\beta_0\|_2^2/n \rightarrow \gamma^2$  as  $n \rightarrow \infty$ , it follows that almost surely

$$\lim_{N \rightarrow \infty} \frac{1}{\sqrt{p}} \sum_{l=0}^{t-1} |{}_{\epsilon}a_t - {}_{\epsilon}\mu_t| \|\beta_0\|_2 = 0.\tag{S60}$$

In conjunction with (S52) and (S54) and (S60), this yields that almost surely,

$$\|{}_{\epsilon}\boldsymbol{\nu}^t - {}_{\epsilon}\boldsymbol{\theta}^t\|_2 = 0.\tag{S61}$$

Almost sure convergence of  $\|{}_{\epsilon}\mathbf{R}^t - {}_{\epsilon}\mathbf{S}^t\|_2$  then follows by an induction argument on  $t$ , (S51), (S61) and since  ${}_{\epsilon}\mathbf{S}^0 = {}_{\epsilon}\mathbf{R}^0$ . This concludes the proof.  $\square$

#### B.4.6 Asymptotic equivalence of AMP and MDYPL

**Theorem B.3.** *In the setting of Lemma B.4 and assuming that there exists a stationary solution  $({}_{\epsilon}\mu_*, {}_{\epsilon}b_*, {}_{\epsilon}\sigma_*)$  to the state evolution (S37)-(S38). Then, if  $\|\hat{\beta}^{\text{DY}}\|_2/\sqrt{n} = \mathcal{O}(1)$  almost surely,*

$$\lim_{\epsilon \rightarrow 0} \lim_{t \rightarrow \infty} \lim_{N \rightarrow \infty} \frac{1}{p} \left\| {}_{\epsilon}\hat{\beta}^t - \hat{\beta}^{\text{DY}} \right\|_2^2 = 0$$

*almost surely.*

*Proof.* First, a second order Taylor approximation of  $\ell(\hat{\beta}^{\text{DY}})$  around  ${}_{\epsilon}\hat{\beta}^t$  gives

$$\ell(\hat{\beta}^{\text{DY}}) = \ell({}_{\epsilon}\hat{\beta}^t) + \nabla \ell({}_{\epsilon}\hat{\beta}^t)^\top (\hat{\beta}^{\text{DY}} - {}_{\epsilon}\hat{\beta}^t) + \frac{1}{2} \mathbf{r},\tag{S62}$$

where the remainder term  $\mathbf{r}$  is, equal to

$$\mathbf{r} = (\hat{\beta}^{\text{DY}} - {}_{\epsilon}\hat{\beta}^t)^\top \nabla \nabla^\top \ell(\hat{\beta}^{\text{DY}} - c({}_{\epsilon}\hat{\beta}^t - \hat{\beta}^{\text{DY}})) (\hat{\beta}^{\text{DY}} - {}_{\epsilon}\hat{\beta}^t),$$

for some constant  $c \in [0, 1]$ . Now by Sur 2019, Lemma 7, with probability at least  $1 - c_1 \exp\{-c_2 n\}$  for absolute constants  $c_1, c_2 > 0$ , it holds that for all  $\beta \in \mathbb{R}^p$

$$\nabla \nabla^\top \ell(\beta) \succ \omega \left( \frac{\|\beta\|_2}{\sqrt{n}} \right) \mathbf{I}_p,$$

where  $\mathbf{A} \succ \mathbf{B}$  means that  $\mathbf{A} - \mathbf{B}$  is positive definite. Here,  $\omega(\cdot) \in (0, 1)$  is a nonincreasing function independent of  $n$ . Clearly,

$$\left\| \hat{\beta}^{\text{DY}} - c(\hat{\beta}^{\text{DY}} - {}_{\epsilon}\hat{\beta}^t) \right\|_2 \leq \max \left\{ \left\| \hat{\beta}^{\text{DY}} \right\|_2, \left\| {}_{\epsilon}\hat{\beta}^t \right\|_2 \right\},$$

so that with probability at least  $1 - c_1 \exp\{-c_2 n\}$

$$\begin{aligned} \mathbf{r} &\geq \left\| \hat{\boldsymbol{\beta}}^{\text{DY}} - \epsilon \hat{\boldsymbol{\beta}}^t \right\|_2^2 \omega \left( \frac{\left\| \hat{\boldsymbol{\beta}}^{\text{DY}} - c(\hat{\boldsymbol{\beta}}^{\text{DY}} - \epsilon \hat{\boldsymbol{\beta}}^t) \right\|_2}{\sqrt{n}} \right) \\ &\geq \left\| \hat{\boldsymbol{\beta}}^{\text{DY}} - \epsilon \hat{\boldsymbol{\beta}}^t \right\|_2^2 \omega \left( \max \left\{ \frac{\left\| \hat{\boldsymbol{\beta}}^{\text{DY}} \right\|_2}{\sqrt{n}}, \frac{\left\| \epsilon \hat{\boldsymbol{\beta}}^t \right\|_2}{\sqrt{n}} \right\} \right). \end{aligned} \quad (\text{S63})$$

Using (S63) and the Cauchy-Schwarz inequality, (S62) can be rearranged as

$$\left\| \hat{\boldsymbol{\beta}}^{\text{DY}} - \epsilon \hat{\boldsymbol{\beta}}^t \right\|_2 \leq \frac{2}{\omega \left( \max \left\{ \frac{\left\| \hat{\boldsymbol{\beta}}^{\text{DY}} \right\|_2}{\sqrt{n}}, \frac{\left\| \epsilon \hat{\boldsymbol{\beta}}^t \right\|_2}{\sqrt{n}} \right\} \right)} \left\| \nabla \ell(\epsilon \hat{\boldsymbol{\beta}}^t) \right\|_2,$$

so that it remains to control  $\left\| \hat{\boldsymbol{\beta}}^{\text{DY}} \right\|_2$ ,  $\left\| \epsilon \hat{\boldsymbol{\beta}}^t \right\|_2$  and  $\left\| \nabla \ell(\epsilon \hat{\boldsymbol{\beta}}^t) \right\|_2$ . Towards bounding  $\left\| \nabla \ell(\epsilon \hat{\boldsymbol{\beta}}^t) \right\|_2$ , recall that by (S34) and (S35), any by the definition of the function  $\Psi^t(\cdot, \cdot)$ , and the identity  $z - \zeta'(\text{prox}_{b\zeta}(z)) = \text{prox}_{b\zeta}(z)$ ,

$$-\text{prox}_{\epsilon b_t \zeta}(\epsilon b_t \epsilon \mathbf{y}^* + \epsilon \mathbf{S}^{t-1}) = \epsilon \mathbf{S}^t - \epsilon \mathbf{S}^{t-1} + \mathbf{X}_\epsilon \hat{\boldsymbol{\beta}}^t,$$

and thus

$$\epsilon \hat{\boldsymbol{\beta}}^t - \epsilon \hat{\boldsymbol{\beta}}^{t-1} = \frac{\epsilon b_t}{\kappa} \mathbf{X}^\top \left\{ \epsilon \mathbf{y}^* - \zeta'(\epsilon \mathbf{S}^t - \epsilon \mathbf{S}^{t-1} + \mathbf{X}_\epsilon \hat{\boldsymbol{\beta}}^t) \right\}.$$

Therefore,

$$\begin{aligned} \nabla \ell(\epsilon \hat{\boldsymbol{\beta}}^t) &= \mathbf{X}^\top \left\{ \mathbf{y} - \zeta'(\mathbf{X}_\epsilon \hat{\boldsymbol{\beta}}^t) \right\} \\ &= \mathbf{X}^\top \left\{ \mathbf{y} - \epsilon \mathbf{y} \right\} \\ &\quad + \mathbf{X}^\top \left\{ \epsilon \mathbf{y} - \zeta'(\epsilon \mathbf{S}^t - \epsilon \mathbf{S}^{t-1} - \mathbf{X}_\epsilon \hat{\boldsymbol{\beta}}^t) \right\} \\ &\quad + \mathbf{X}^\top \left\{ \zeta'(\epsilon \mathbf{S}^t - \epsilon \mathbf{S}^{t-1} - \mathbf{X}_\epsilon \hat{\boldsymbol{\beta}}^t) - \zeta'(\mathbf{X}_\epsilon \hat{\boldsymbol{\beta}}^t) \right\}. \end{aligned}$$

almost surely. Further, using that  $\zeta'(x)$  is Lipschitz with Lipschitz constant  $1/4$ ,

$$\begin{aligned} \left\| \mathbf{X}^\top \left\{ \zeta'(\epsilon \mathbf{S}^t - \epsilon \mathbf{S}^{t-1} - \mathbf{X}_\epsilon \hat{\boldsymbol{\beta}}^t) - \zeta'(\mathbf{X}_\epsilon \hat{\boldsymbol{\beta}}^t) \right\} \right\|_2 &\leq \left\| \mathbf{X} \right\|_2 \left\| \zeta'(\epsilon \mathbf{S}^t - \epsilon \mathbf{S}^{t-1} - \mathbf{X}_\epsilon \hat{\boldsymbol{\beta}}^t) - \zeta'(\mathbf{X}_\epsilon \hat{\boldsymbol{\beta}}^t) \right\|_2 \\ &\leq \frac{1}{4} \left\| \mathbf{X} \right\|_2 \left\| \epsilon \mathbf{S}^t - \epsilon \mathbf{S}^{t-1} + \mathbf{X}_\epsilon \hat{\boldsymbol{\beta}}^t - \mathbf{X}_\epsilon \hat{\boldsymbol{\beta}}^t \right\|_2 \\ &= \frac{1}{4} \left\| \mathbf{X} \right\|_2 \left\| \epsilon \mathbf{S}^t - \epsilon \mathbf{S}^{t-1} \right\|_2 \end{aligned}$$

Using (S34), it immediately follows that

$$\left\| \mathbf{X}^\top \left\{ \epsilon \mathbf{y} - \zeta'(\epsilon \mathbf{S}^t - \epsilon \mathbf{S}^{t-1} - \mathbf{X}_\epsilon \hat{\boldsymbol{\beta}}^t) \right\} \right\|_2 = \frac{\kappa}{\epsilon b_t} \left\| \epsilon \hat{\boldsymbol{\beta}}^t - \epsilon \hat{\boldsymbol{\beta}}^{t-1} \right\|_2.$$

Therefore, with probability at least  $1 - c_1 \exp\{-c_2 n\}$ ,

$$\left\| \hat{\boldsymbol{\beta}}^{\text{DY}} - \epsilon \hat{\boldsymbol{\beta}}^t \right\|_2 \leq \frac{2}{\omega \left( \max \left\{ \frac{\left\| \hat{\boldsymbol{\beta}}^{\text{DY}} \right\|_2}{\sqrt{n}}, \frac{\left\| \epsilon \hat{\boldsymbol{\beta}}^t \right\|_2}{\sqrt{n}} \right\} \right)} \left\{ \frac{\kappa}{\epsilon b_t} \left\| \epsilon \hat{\boldsymbol{\beta}}^t - \epsilon \hat{\boldsymbol{\beta}}^{t-1} \right\|_2 + \frac{1}{4} \left\| \mathbf{X} \right\|_2 \left\| \epsilon \mathbf{S}^t - \epsilon \mathbf{S}^{t-1} \right\|_2 + \left\| \mathbf{X} \right\|_2 \left\| \mathbf{y} - \epsilon \mathbf{y} \right\|_2 \right\}.$$

To finish the proof initialise the AMP recursion at the stationary solution, i.e.  $(\epsilon \mu_0, \epsilon b_0, \epsilon \sigma_0) = (\epsilon \mu_*, \epsilon b_*, \epsilon \sigma_*)$ . Then it follows immediately from (S48) with  $\psi(x, y) = x^2$ , in conjunction with

Lemma B.4 and the stationarity condition that almost surely

$$\lim_{N \rightarrow \infty} \frac{\|\epsilon \hat{\beta}^t\|_2}{\sqrt{p}} \leq \lim_{N \rightarrow \infty} \frac{\|\epsilon \hat{\beta}^t - \epsilon \mu_* \beta_0\|_2}{\sqrt{p}} + \lim_{n \rightarrow \infty} \frac{\|\epsilon \mu_* \beta_0\|_2}{\sqrt{p}} = \epsilon \sigma_* + \frac{\gamma}{\epsilon \mu_* \kappa}. \quad (\text{S64})$$

Further,  $\|\hat{\beta}^{\text{DY}}\|_2/\sqrt{n} = \mathcal{O}(1)$  almost surely by assumption. Hence, by the Cauchy property of  $\epsilon \nu^t, \epsilon \mathbf{R}^t$ , as shown in Lemma G.8 along with the equivalence of recursions of Lemma B.4, (S64) and Lemma G.4 and Lemma G.5, it follows that with probability at least  $1 - c_1 \exp\{-c_n\}$

$$\lim_{\epsilon \rightarrow 0} \lim_{t \rightarrow \infty} \lim_{N \rightarrow \infty} \frac{1}{\sqrt{p}} \|\epsilon \hat{\beta}^t - \hat{\beta}^{\text{DY}}\|_2 = 0.$$

The almost sure claim comes from the first Borel-Cantelli Lemma (e.g. Shiryaev 2016, p. 308).  $\square$

It is now possible to finish the proof of Theorem 3.1. First of all, note that by Lemma G.6, there exists a unique stationary solution  $(\epsilon \mu_*, \epsilon b_*, \epsilon \sigma_*)$  to the state evolution (S37)-(S38) that is continuous in  $\epsilon$  such that  $\lim_{\epsilon \rightarrow 0} (\epsilon \mu_*, \epsilon b_*, \epsilon \sigma_*) = (\mu_*, b_*, \sigma_*)$ , where  $(\mu_*, b_*, \sigma_*)$  are a stationary solution to (S16), (S17), (S18).

Now, let  $\psi$  be a pseudo Lipschitz function of order 2. Then

$$\begin{aligned} & \left| \frac{1}{p} \sum_{j=1}^p \psi \left( \hat{\beta}_j^{\text{DY}} - \mu_* \beta_{0,j}, \beta_{0,j} \right) - \frac{1}{p} \sum_{j=1}^p \psi \left( \epsilon \nu^t, \beta_{0,j} \right) \right| \\ & \leq \left| \frac{1}{p} \sum_{j=1}^p \psi \left( \hat{\beta}_j^{\text{DY}} - \epsilon \mu_* \beta_{0,j}, \beta_{0,j} \right) - \frac{1}{p} \sum_{j=1}^p \psi \left( \epsilon \hat{\beta}^t - \epsilon \mu_* \beta_{0,j}, \beta_{0,j} \right) \right| \\ & \quad + \left| \frac{1}{p} \sum_{j=1}^p \psi \left( \epsilon \hat{\beta}^t - \epsilon \mu_* \beta_{0,j}, \beta_{0,j} \right) - \frac{1}{p} \sum_{j=1}^p \psi \left( \epsilon \nu^t, \beta_{0,j} \right) \right|. \quad (\text{S65}) \end{aligned}$$

Now

$$\begin{aligned} & \sum_{j=1}^p \left| \psi \left( \hat{\beta}_j^{\text{DY}} - \epsilon \mu_* \beta_{0,j}, \beta_{0,j} \right) - \psi \left( \epsilon \hat{\beta}^t - \epsilon \mu_* \beta_{0,j}, \beta_{0,j} \right) \right| \\ & \leq \sum_{j=1}^p \left| \psi \left( \hat{\beta}_j^{\text{DY}} - \epsilon \mu_* \beta_{0,j}, \beta_{0,j} \right) - \psi \left( \epsilon \hat{\beta}^t - \epsilon \mu_* \beta_{0,j}, \beta_{0,j} \right) \right| \\ & \leq C \sum_{j=1}^p \left( 1 + \left\| \begin{bmatrix} \hat{\beta}_j^{\text{DY}} - \epsilon \mu_* \beta_{0,j} \\ \beta_{0,j} \end{bmatrix} \right\|_2 + \left\| \begin{bmatrix} \epsilon \hat{\beta}^t - \epsilon \mu_* \beta_{0,j} \\ \beta_{0,j} \end{bmatrix} \right\|_2 \right) \left\| \hat{\beta}_j^{\text{DY}} - \epsilon \hat{\beta}^t \right\|_2 \\ & \leq C \sqrt{\sum_{j=1}^p \left( 1 + \left\| \begin{bmatrix} \hat{\beta}_j^{\text{DY}} - \epsilon \mu_* \beta_{0,j} \\ \beta_{0,j} \end{bmatrix} \right\|_2 + \left\| \begin{bmatrix} \epsilon \hat{\beta}^t - \epsilon \mu_* \beta_{0,j} \\ \beta_{0,j} \end{bmatrix} \right\|_2 \right)^2} \left\| \hat{\beta}^{\text{DY}} - \epsilon \hat{\beta}^t \right\|_2, \quad (\text{S66}) \end{aligned}$$

where the first inequality follows from the triangle inequality, the second by virtue of  $\psi$  being pseudo Lipschitz of order 2 and the last by the Cauchy-Schwarz inequality.

Further, letting  $\mathbf{a}_j = [a_{j1}, a_{j2}]^\top = [\hat{\beta}_j^{\text{DY}} - \epsilon \mu_* \beta_{0,j}, \beta_{0,j}]^\top$  and  $\mathbf{b}_j = [b_{j1}, a_{j2}]^\top = [\hat{\beta}_j^t - \epsilon \mu_* \beta_{0,j}, \beta_{0,j}]^\top$ ,

simple manipulations yield

$$\begin{aligned}
\sum_{j=1}^p (1 + \|\mathbf{a}_j\|_2 + \|\mathbf{b}_j\|_2)^2 &= \sum_{j=1}^p 1 + 2(\|\mathbf{a}_j\|_2 + \|\mathbf{b}_j\|_2) + (\|\mathbf{a}_j\|_2 + \|\mathbf{b}_j\|_2)^2 \\
&= p + 2 \sum_{j=1}^p \|\mathbf{a}_j\|_2 + 2 \sum_{j=1}^p \|\mathbf{b}_j\|_2 + \sum_{j=1}^p \|\mathbf{a}_j\|_2^2 + \sum_{j=1}^p \|\mathbf{b}_j\|_2^2 + 2 \sum_{j=1}^p \|\mathbf{a}_j\|_2 \|\mathbf{b}_j\|_2 \\
&= p + \|\mathbf{a}_{\bullet 1}\|_2^2 + \|\mathbf{b}_{\bullet 1}\|_2^2 + 2\|\mathbf{a}_{\bullet 2}\|_2^2 + 2 \sum_{j=1}^p \|\mathbf{a}_j\|_2 + 2 \sum_{j=1}^p \|\mathbf{b}_j\|_2 + 2 \sum_{j=1}^p \|\mathbf{a}_j\|_2 \|\mathbf{b}_j\|_2 \\
&\leq p + \|\mathbf{a}_{\bullet 1}\|_2^2 + \|\mathbf{b}_{\bullet 1}\|_2^2 + 2\|\mathbf{a}_{\bullet 2}\|_2^2 + 2 \sum_{j=1}^p |a_{j1}| + 2 \sum_{j=1}^p |b_{j1}| + 4 \sum_{j=1}^p |a_{j2}| + 2 \sum_{j=1}^p \|\mathbf{a}_j\|_2 \|\mathbf{b}_j\|_2 \\
&= p + \|\mathbf{a}_{\bullet 1}\|_2^2 + \|\mathbf{b}_{\bullet 1}\|_2^2 + 2\|\mathbf{a}_{\bullet 2}\|_2^2 + 2\|\mathbf{a}_{\bullet 1}\|_1 + 2\|\mathbf{b}_{\bullet 1}\|_1 + 4\|\mathbf{a}_{\bullet 2}\|_1 + 2 \sum_{j=1}^p \|\mathbf{a}_j\|_2 \|\mathbf{b}_j\|_2 \\
&\leq p + \|\mathbf{a}_{\bullet 1}\|_2^2 + \|\mathbf{b}_{\bullet 1}\|_2^2 + 2\|\mathbf{a}_{\bullet 2}\|_2^2 + 2\sqrt{p}\|\mathbf{a}_{\bullet 1}\|_2 + 2\sqrt{p}\|\mathbf{b}_{\bullet 1}\|_2 + 4\sqrt{p}\|\mathbf{a}_{\bullet 2}\|_2 + 2 \sum_{j=1}^p \|\mathbf{a}_j\|_2 \|\mathbf{b}_j\|_2 \\
&\leq p + \|\mathbf{a}_{\bullet 1}\|_2^2 + \|\mathbf{b}_{\bullet 1}\|_2^2 + 2\|\mathbf{a}_{\bullet 2}\|_2^2 + 2\sqrt{p}\|\mathbf{a}_{\bullet 1}\|_2 + 2\sqrt{p}\|\mathbf{b}_{\bullet 1}\|_2 + 4\sqrt{p}\|\mathbf{a}_{\bullet 2}\|_2 \\
&\quad + 2\sqrt{\sum_{j=1}^p a_{j1}^2 + a_{j2}^2} \sqrt{\sum_{j=1}^p b_{j1}^2 + a_{j2}^2} \\
&\leq p + \|\mathbf{a}_{\bullet 1}\|_2^2 + \|\mathbf{b}_{\bullet 1}\|_2^2 + 2\|\mathbf{a}_{\bullet 2}\|_2^2 + 2\sqrt{p}\|\mathbf{a}_{\bullet 1}\|_2 + 2\sqrt{p}\|\mathbf{b}_{\bullet 1}\|_2 + 4\sqrt{p}\|\mathbf{a}_{\bullet 2}\|_2 \\
&\quad + 2(\|\mathbf{a}_{\bullet 1}\|_2 + \|\mathbf{a}_{\bullet 2}\|_2)(\|\mathbf{b}_{\bullet 1}\|_2 + \|\mathbf{a}_{\bullet 2}\|_2), \tag{S67}
\end{aligned}$$

where  $\mathbf{a}_{\bullet i} = (a_{1i}, \dots, a_{pi})$ , ( $i = 1, 2$ ) and a similar convention applies to  $\mathbf{b}_{\bullet 1}$ . The fourth line follows since  $\sqrt{x^2 + y^2} \leq \sqrt{x^2} + \sqrt{y^2} = |x| + |y|$ , the sixth by the Cauchy-Schwarz inequality and since  $\|\mathbf{v}\|_1 = |\langle \mathbf{1}, \mathbf{v} \rangle|$ , where  $\mathbf{1}$  is a  $p$ -vector of ones and the absolute value acts elementwise on  $\mathbf{v}$ . The seventh line follows again by Cauchy-Schwarz, and the last again since  $\sqrt{x+y} \leq \sqrt{x} + \sqrt{y}$ . Now, since  $\epsilon\mu_* < \infty$ , and by assumption on  $\hat{\beta}^{\text{DY}}, \beta_0$ , almost surely,

$$\begin{aligned}
\lim_{N \rightarrow \infty} \frac{1}{\sqrt{p}} \|\mathbf{a}_{\bullet 1}\|_2 &= \lim_{N \rightarrow \infty} \frac{1}{\sqrt{p}} \|\hat{\beta}^{\text{DY}} - \epsilon\mu_*\beta_0\|_2 \leq \lim_{N \rightarrow \infty} \frac{1}{\sqrt{p}} \|\hat{\beta}^{\text{DY}}\| + \epsilon\mu_* \frac{1}{\sqrt{p}} \|\beta_0\|_2 < C + \epsilon\mu_*\gamma \\
\lim_{N \rightarrow \infty} \frac{1}{\sqrt{p}} \|\mathbf{a}_{\bullet 2}\|_2 &= \lim_{N \rightarrow \infty} \frac{1}{\sqrt{p}} \|\beta_0\|_2 = \gamma,
\end{aligned}$$

for some constant  $C > 0$ , which is independent of  $t, \epsilon$ . Further, by (S64), almost surely

$$\lim_{N \rightarrow \infty} \frac{1}{\sqrt{p}} \|\mathbf{b}_{\bullet 1}\|_2 = \lim_{N \rightarrow \infty} \frac{1}{\sqrt{p}} \|\hat{\beta}^t - \epsilon\mu_*\beta_0\|_2 = \epsilon\sigma_*^2.$$

Therefore, (S67) gives that almost surely

$$\lim_{N \rightarrow \infty} \frac{1}{p} \sum_{j=1}^p (1 + \|\mathbf{a}_j\|_2 + \|\mathbf{b}_j\|_2)^2 \leq 1 + (C + \epsilon\mu_*\gamma) \{2 + C + \epsilon\mu_*\} + \epsilon\sigma_*^2 \{2 + \epsilon\sigma_*^2\} + 4\gamma + 2\{C + \epsilon\mu_*\gamma + \gamma\} \{\epsilon\sigma_*^2 + \gamma\}. \tag{S68}$$

And thus

$$\lim_{\epsilon \rightarrow 0} \lim_{t \rightarrow \infty} \lim_{N \rightarrow \infty} \frac{1}{p} \sum_{j=1}^p (1 + \|\mathbf{a}_j\|_2 + \|\mathbf{b}_j\|_2)^2 \leq 1 + (C + \mu_*\gamma) \{2 + C + \mu_*\} + \sigma_*^2 \{2 + \sigma_*^2\} + 4\gamma + 2\{C + \mu_*\gamma + \gamma\} \{\sigma_*^2 + \gamma\},$$

where  $\lim_{\epsilon \rightarrow 0} (\epsilon \mu_*, \epsilon \sigma_*) = (\mu_*, \sigma_*)$  follows from Lemma G.6. In conjunction with Theorem B.3 and (S66), this yields that almost surely

$$\lim_{\epsilon \rightarrow 0} \lim_{t \rightarrow \infty} \lim_{N \rightarrow \infty} \frac{1}{p} \sum_{j=1}^p \left| \psi \left( \hat{\beta}_j^{\text{DY}} - \epsilon \mu_* \beta_{0,j}, \beta_{0,j} \right) - \psi \left( \epsilon \hat{\beta}^t - \epsilon \mu_* \beta_{0,j}, \beta_{0,j} \right) \right| = 0.$$

Similarly,

$$\begin{aligned} & \left| \frac{1}{p} \sum_{j=1}^p \psi \left( \epsilon \hat{\beta}^t - \epsilon \mu_* \beta_{0,j}, \beta_{0,j} \right) - \psi \left( \epsilon \nu^t, \beta_{0,j} \right) \right| \\ & \leq C \frac{1}{p} \sqrt{\sum_{j=1}^p \left( 1 + \left\| \begin{bmatrix} \epsilon \hat{\beta}^t - \epsilon \mu_* \beta_{0,j} \\ \beta_{0,j} \end{bmatrix} \right\|_2 + \left\| \begin{bmatrix} \epsilon \nu^t \\ \beta_{0,j} \end{bmatrix} \right\|_2 \right)^2} \left\| \epsilon \hat{\beta}^t - \epsilon \mu_* \beta_0 - \epsilon \nu^t \right\|_2, \end{aligned}$$

the right hand side of which is zero almost surely as  $N \rightarrow \infty$  for all  $t, \epsilon > 0$ , by Lemma B.4 and (S68). and thus almost surely

$$\lim_{\epsilon \rightarrow 0} \lim_{t \rightarrow \infty} \lim_{N \rightarrow \infty} \left| \frac{1}{p} \sum_{j=1}^p \psi \left( \hat{\beta}_j^{\text{DY}} - \mu_* \beta_{0,j}, \beta_{0,j} \right) - \psi \left( \epsilon \hat{\beta}_j^{\text{DY}} - \epsilon \mu_* \beta_{0,j}, \beta_{0,j} \right) \right| = 0.$$

Now recall that from Corollary B.2.1, and by the stationarity assumption of the phase transition parameters,  $(\epsilon \mu_*, \epsilon b_*, \epsilon \sigma_*)$ , almost surely

$$\lim_{t \rightarrow \infty} \lim_{N \rightarrow \infty} \frac{1}{p} \sum_{j=1}^p \psi(\epsilon \nu_j^t, \beta_{0,j}) = \lim_{N \rightarrow \infty} \frac{1}{p} \sum_{j=1}^p \psi(\epsilon \nu_j^t, \beta_{0,j}) = \mathbb{E} [\psi(\epsilon \sigma_* G, \bar{\beta})],$$

where  $G \sim N(0, 1) \perp \bar{\beta}$ . Since  $\psi$  is pseudo-Lipschitz of order two,

$$\begin{aligned} & |\mathbb{E} [\psi(\epsilon \sigma_* G, \bar{\beta})] - \mathbb{E} [\psi(\sigma_* G, \bar{\beta})]| \leq \mathbb{E} [|\psi(\epsilon \sigma_* G, \bar{\beta}) - \psi(\sigma_* G, \bar{\beta})|] \\ & \leq C |\epsilon \sigma_* - \sigma_*| \mathbb{E} [(1 + \|\epsilon \sigma_* G, \bar{\beta}\|_2 + \|\sigma_* G, \bar{\beta}\|_2) |G|], \end{aligned}$$

and thus it follows that

$$\lim_{\epsilon \rightarrow 0} \lim_{t \rightarrow \infty} \lim_{N \rightarrow \infty} \frac{1}{p} \sum_{j=1}^p \psi(\epsilon \nu_j^t, \beta_{0,j}) = \mathbb{E} [\psi(\sigma_* G, \bar{\beta})].$$

In conjunction with (S65), this establishes (S6). Finally, equivalence of stationary solutions (S3)-(S5) with the stationary solutions to (S16)-(S18) is shown in Lemma G.9. This concludes the proof of the Theorem.

## C Proof of Theorem 3.2

**Theorem 3.2.** *In the setting of Theorem 3.1, and if  $(\kappa, \gamma)$  are such that the ML estimate exists with probability approaching one, then almost surely*

$$\lim_{n \rightarrow \infty} \frac{\left\| \hat{\beta}^{\text{DY}}(\alpha) \right\|_2}{\sqrt{n}} = \mathcal{O}(1), \quad (\text{S69})$$

*for any  $\alpha \in (0, 1)$ . Furthermore, for any  $(\kappa, \gamma)$ , there exists an  $\alpha_0 \in (0, 1)$  such that (S69) holds almost surely for all  $0 < \alpha < \alpha_0$ .*

Both parts of Theorem 3.2 are proven in turn.

**Theorem C.1.** *Under the modelling assumption of Section A, and if  $\gamma < g_{MLE}(\kappa)$ , where  $g_{MLE}$  is the phase transition of Candès and Sur (2020), then almost surely*

$$\lim_{n \rightarrow \infty} \left\| \hat{\beta}^{DY} \right\|_2 = \mathcal{O}(\sqrt{n}).$$

*Proof.* The proof relies on the arguments in the proof of Theorem 4 in the supplementary material of Sur and Candès (2019). All that needs to be done is to show that the DY-prior penalty provides some slackness in the string of inequalities that guarantee boundedness of the estimator.

Write the negative log-likelihood with pseudo-responses  $\mathbf{y}^*$  as

$$-\log \ell(\beta; \mathbf{y}^*, \mathbf{X}) = \alpha \sum_{i=1}^n \zeta(-\tilde{y}_i \mathbf{x}_i^\top \beta) + (1 - \alpha) \left[ \sum_{i=1}^n -\frac{1}{2} \mathbf{x}_i^\top \beta + \zeta(\mathbf{x}_i^\top \beta) \right],$$

where  $\tilde{y}_i = 2y_i - 1$  and  $\zeta(x) = \log(1 + e^x)$ . Assume that

- i) Given a constant  $c > 0$ , for  $\mathcal{B} = \bigcap_{n > N_0} \{s_{\min}(\mathbf{X}) > c\}$  be the event that there exists a  $N_0$  such that for all  $n > N_0$ ,  $s_{\min}(\mathbf{X}) > c$
- ii)  $-\ell(\beta; \mathbf{y}^*, \mathbf{X}) \leq -\ell(\mathbf{0}_p; \mathbf{y}^*, \mathbf{X}) = n \log(2)$ ,
- iii)  $\frac{\|\beta\|_2}{\sqrt{n}} > \frac{\log(2)}{c\epsilon^2}$

Let  $J = \{j \in \{1, \dots, n\} : \tilde{y}_j \mathbf{x}_j^\top \beta < 0\}$ . Then note that ii) implies that

$$\sum_{j=1}^n \max \{-\tilde{y}_j \mathbf{x}_j^\top \beta, 0\} \leq n \log(2). \quad (\text{S70})$$

Indeed, consider

$$\begin{aligned} \alpha \sum_{j=1}^n \max \{-\tilde{y}_j \mathbf{x}_j^\top \beta, 0\} + (1 - \alpha) \left[ \sum_{j=1}^n -\frac{1}{2} \mathbf{x}_j^\top \beta + \zeta(\mathbf{x}_j^\top \beta) \right] &= \alpha \sum_{j \in J} -\tilde{y}_j \mathbf{x}_j^\top \beta + (1 - \alpha) \left[ \sum_{j=1}^n -\frac{1}{2} \mathbf{x}_j^\top \beta + \zeta(\mathbf{x}_j^\top \beta) \right] \\ &\leq \alpha \sum_{j \in J} \zeta(-\tilde{y}_j \mathbf{x}_j^\top \beta) + (1 - \alpha) \left[ \sum_{j=1}^n -\frac{1}{2} \mathbf{x}_j^\top \beta + \zeta(\mathbf{x}_j^\top \beta) \right] \\ &\leq \alpha \sum_{j \in J} \zeta(-\tilde{y}_j \mathbf{x}_j^\top \beta) + (1 - \alpha) \left[ \sum_{j=1}^n -\frac{1}{2} \mathbf{x}_j^\top \beta + \zeta(\mathbf{x}_j^\top \beta) \right] \\ &= -\ell(\beta; \mathbf{y}^*, \mathbf{X}), \end{aligned}$$

where it was used that  $x < \zeta(x)$  for  $x \in \mathbb{R}$ . Now assume that  $\beta$  is such that  $-\ell(\beta; \mathbf{y}^*, \mathbf{X}) \leq n \log(2) = -\ell(\mathbf{0}_p; \mathbf{y}^*, \mathbf{X})$ . Then for such  $\beta$ ,

$$\alpha \sum_{j \in J} \zeta(-\tilde{y}_j \mathbf{x}_j^\top \beta) \leq n \log(2) - (1 - \alpha) \left[ \sum_{i=1}^n -\frac{1}{2} \mathbf{x}_i^\top \beta + \zeta(\mathbf{x}_i^\top \beta) \right]. \quad (\text{S71})$$

Now note that  $(1 - \alpha) \left[ \sum_{i=1}^n -\frac{1}{2} \mathbf{x}_i^\top \beta + \zeta(\mathbf{x}_i^\top \beta) \right]$  is always greater than zero as  $\zeta(x) > x$  for  $x \in \mathbb{R}$

and that this expression is minimised for  $\beta = \mathbf{0}_p$ . Hence, (S71) can be upper bounded as

$$\begin{aligned}
\alpha \sum_{j \in J} \zeta(-\tilde{y}_j \mathbf{x}_j^\top \beta) &\leq n \log(2) - (1 - \alpha) \left[ \sum_{i=1}^n -\frac{1}{2} \mathbf{x}_i^\top \beta + \zeta(\mathbf{x}_i^\top \beta) \right] \\
&\leq n \log(2) - (1 - \alpha) \left[ \sum_{i=1}^n -\frac{1}{2} \mathbf{x}_i^\top \mathbf{0}_p + \zeta(\mathbf{0}_p^\top \beta) \right] \\
&= n \log(2) - (1 - \alpha) n \log(2) \\
&= \alpha n \log(2),
\end{aligned}$$

which establishes (S70) since then by definition of  $J$  and as  $\zeta(x) > x$ ,

$$\sum_{j=1}^n \max\{-\tilde{y}_j \mathbf{x}_j^\top \beta, 0\} = \sum_{j \in J} -\tilde{y}_j \mathbf{x}_j^\top \beta \leq \sum_{j \in J} \zeta(-\tilde{y}_j \mathbf{x}_j^\top \beta) \leq n \log(2).$$

Next, note that conditional on event  $\mathcal{B}$  from assumptions i) & iii) it follows that

$$n \log(2) \leq \frac{n \log(2)}{c} s_{\min}(\mathbf{X}) \leq \frac{n \log(2)}{c} \frac{\|\mathbf{X}\beta\|_2}{\|\beta\|_2} = \frac{n \log(2)}{c} \frac{\|\tilde{\mathbf{y}} \circ \mathbf{X}\beta\|_2}{\|\beta\|_2} \leq \epsilon^2 \sqrt{n} \|\tilde{\mathbf{y}} \circ \mathbf{X}\beta\|_2,$$

where the first inequality holds by event  $\mathcal{B}$ , the second by the Courant-Fischer characterisation of eigenvalues (e.g. Magnus and Neudecker 2019, Section 1.8, Theorem 7), the next equality since  $\tilde{\mathbf{y}} \in \{-1, 1\}$  and the definition of the Hadamard product  $\circ$  and the  $\ell_2$ -norm, and the last inequality follows by iii).

Note that by definition of  $\hat{\beta}^{\text{DY}}$ , it must hold that  $-\ell(\hat{\beta}^{\text{DY}}; \mathbf{y}^*, \mathbf{X}) \leq n \log(2)$ . Hence, conditional on event  $\mathcal{B}$ ,  $\|\hat{\beta}^{\text{DY}}\|_2 / \sqrt{n} > \log(2) / (c\epsilon^2)$  implies that  $\tilde{\mathbf{y}} \circ \mathbf{X}\hat{\beta}^{\text{DY}}$  must fall in the cone

$$\mathcal{A} = \left\{ \mathbf{u} \in \mathbb{R}^n : \sum_{j=1}^n \max\{-u_j, 0\} \leq \epsilon^2 \sqrt{n} \|\mathbf{u}\|_2 \right\}.$$

Therefore

$$\Pr \left( \frac{\|\hat{\beta}^{\text{DY}}\|_2}{\sqrt{n}} > \frac{\log(2)}{c\epsilon^2} \middle| \mathcal{B} \right) \leq \Pr \left( \tilde{\mathbf{y}} \circ \mathbf{X}\hat{\beta}^{\text{DY}} \in \mathcal{A} \middle| \mathcal{B} \right).$$

Next, note that by a straightforward application of Theorem 2.6 in Rudelson and Vershynin (2010), it follows that for any  $\kappa$ , there exist constants  $c_1, c_2 > 0$  such that

$$\Pr(s_{\min}(\mathbf{X}) > c_1) \geq 1 - 2 \exp\{-c_2 n\}.$$

Therefore, letting  $\mathcal{C}_n$  be the event that  $s_{\min}(\mathbf{X}) < c_1$  for  $\mathbf{X} \in \mathbb{R}^{n \times p}$ , the first Borel-Cantelli Lemma gives that the event  $\Pr(\mathcal{C}_n \text{ infinitely often}) = 0$ . Hence, there must exist a  $N_0$  such that  $\Pr(\bigcap_{n > N_0} s_{\min}(\mathbf{X}) > c_1) = 1$ . Thus, letting  $\mathcal{B} = \bigcap_{n > N_0} s_{\min}(\mathbf{X}) > c_1$ , it follows that for  $n > N_0$ ,

$\epsilon > 0$ ,

$$\begin{aligned}
\Pr\left(\frac{\|\hat{\beta}^{\text{DY}}\|_2}{\sqrt{n}} > \frac{\log(2)c_1}{\epsilon^2}\right) &= \Pr\left(\frac{\|\hat{\beta}^{\text{DY}}\|_2}{\sqrt{n}} > \frac{\log(2)c_1}{\epsilon^2} \middle| \mathcal{B}\right) \Pr(\mathcal{B}) \\
&\quad + \Pr\left(\frac{\|\hat{\beta}^{\text{DY}}\|_2}{\sqrt{n}} > \frac{\log(2)c_1}{\epsilon^2} \middle| \neg\mathcal{B}\right) (1 - \Pr(\mathcal{B})) \\
&= \Pr\left(\frac{\|\hat{\beta}^{\text{DY}}\|_2}{\sqrt{n}} > \frac{\log(2)c_1}{\epsilon^2} \middle| \mathcal{B}\right) \cdot 1 + 0 \\
&= \Pr\left(\frac{\|\hat{\beta}^{\text{DY}}\|_2}{\sqrt{n}} > \frac{\log(2)c_1}{\epsilon^2} \middle| \mathcal{B}\right)
\end{aligned}$$

A similar argument shows that  $\Pr(\tilde{\mathbf{y}} \circ \mathbf{X}\hat{\beta}^{\text{DY}} \in \mathcal{A} | \mathcal{B}) = \Pr(\tilde{\mathbf{y}} \circ \mathbf{X}\hat{\beta}^{\text{DY}} \in \mathcal{A})$ . Thus, for  $n > N_0$ ,

$$\begin{aligned}
\Pr\left(\frac{\|\hat{\beta}^{\text{DY}}\|_2}{\sqrt{n}} > \frac{\log(2)c_1}{\epsilon^2}\right) &\leq \Pr(\tilde{\mathbf{y}} \circ \mathbf{X}\hat{\beta}^{\text{DY}} \in \mathcal{A}) \\
&\leq \Pr(\{\tilde{\mathbf{y}} \circ \mathbf{X}\mathbf{b} : \mathbf{b} \in \mathbb{R}^p\} \cap \mathcal{A} \neq \{\mathbf{0}_n\})
\end{aligned}$$

This event is shown to have probability at most  $Cn^{-\delta}$  for some constants  $C > 0, \delta > 1$  in the proof of Theorem 4 in the supplementary material of Sur and Candès (2019) (see also Sur *et al.* 2019, Theorem 7 for more details).

The almost sure part of the claim follows again by the first Borel-Cantelli Lemma. This concludes the proof.  $\square$

**Theorem C.2.** *In the setting of Section A, for any pair  $(\kappa, \gamma)$ , there exists an  $\alpha_0 \in (0, 1)$  such that for all  $0 < \alpha < \alpha_0$ ,*

$$\|\hat{\beta}^{\text{DY}}(\alpha)\|_2 = \mathcal{O}(\sqrt{n})$$

*almost surely for the corresponding MDYPL estimator,  $\hat{\beta}^{\text{DY}}(\alpha)$ , with shrinkage parameter  $\alpha$ .*

*Proof.* It shall be argued that for any  $\kappa, \gamma$ , there exists a radius  $r_0 = c\sqrt{n}$  for some constant  $c > 0$  and a cutoff  $\alpha_0 \in (0, 1)$  such that for all  $\alpha < \alpha_0$ , the maximiser of  $\ell(\beta; \mathbf{y}^*, \mathbf{X})$  as defined in (S2) lies in the set  $S = \{\beta \in \mathbb{R}^p : \|\beta\|_2 \leq r_0\}$  eventually almost surely. Towards this end, let  $p(\beta) = \frac{1-\alpha}{\alpha} \sum_{i=1}^n \frac{1}{2} \mathbf{x}_i^\top \beta - \zeta(\mathbf{x}_i^\top \beta)$  be the log of the prior (S1) with  $\beta_P = \mathbf{0}_p$  bar the normalizing constant and fix any  $\kappa \in (0, 1)$ ,  $\gamma > 0$ . By Lemma C.1, there exist  $c > 0$ ,  $\alpha_0 \in (0, 1)$  such that for all  $0 < \alpha < \alpha_0$ , such that

$$\sup_{\substack{\beta \in \mathbb{R}^p: \\ \|\beta\|_2 > c\sqrt{n}}} p(\beta) < -\frac{1}{\alpha} n \log(2), \quad (\text{S72})$$

with probability at least  $1 - c_1 \exp\{-c_2 n\}$  for some universal constants  $c_1, c_2$  and  $n > n_0$ . Since the log-likelihood  $\ell(\beta; \mathbf{y}, \mathbf{X})$  from a logistic regression model is always bounded from above by zero, it follows that, upon the event of (S72),  $\ell(\beta; \mathbf{y}^*, \mathbf{X}) = \ell(\beta; \mathbf{y}, \mathbf{X}) + p(\beta) < -n \log(2)/\alpha = \ell(\mathbf{0}_p; \mathbf{y}^*, \mathbf{X})$ . On the other hand,  $\ell(\beta; \mathbf{y}^*, \mathbf{X})$  obtains a maximum over  $S$  since it is continuous and  $S$  is compact (e.g. Rudin (1976, Theorem 4.16)). Further, since for any  $\beta \notin S$ ,  $\ell(\beta; \mathbf{y}, \mathbf{X}) < \ell(\mathbf{0}_p; \mathbf{y}, \mathbf{X})$  and  $\mathbf{0}_p \in S$ , the maximiser over  $S$  is the global maximiser of  $\ell(\beta; \mathbf{y}, \mathbf{X})$ , which thus must be bounded by  $c\sqrt{n}$  with probability at least  $1 - c_1 \exp\{-c_2 n\}$ . The almost sure part of the statement follows by

the Borel-Cantelli Lemma. This concludes the proof.  $\square$

**Lemma C.1.** Let  $p(\beta) = \frac{1-\alpha}{\alpha} \sum_{i=1}^n \frac{1}{2} \mathbf{x}_i^\top \beta - \zeta(\mathbf{x}_i^\top \beta)$  be the log of the prior (S1) with  $\beta_P = \mathbf{0}_p$  bar the normalizing constant. Then for any  $\kappa \in (0, 1)$ ,  $\gamma > 0$ , there exist  $c > 0$ ,  $\alpha_0 \in (0, 1)$ ,  $n_0$ , such that for all  $0 < \alpha < \alpha_0$ ,  $n > n_0$

$$\sup_{\substack{\beta \in \mathbb{R}^p: \\ \|\beta\|_2 > c\sqrt{n}}} p(\beta) < -\frac{1}{\alpha} n \log(2),$$

with probability at least  $1 - c_1 \exp\{-c_2 n\}$  for some universal constants  $c_1, c_2$ .

*Proof.* First write  $p(\beta) = p(r\mathbf{u})$  for  $r = \|\beta\|_2$ ,  $\mathbf{u} \in S^{p-1}$  and note that  $p(r\mathbf{u})$  is monotonically decreasing in  $r$ . Indeed,

$$\frac{\partial}{\partial r} p(r\mathbf{u}) = \sum_{i=1}^n \mathbf{x}_i^\top \mathbf{u} \left( \frac{1}{2} - \zeta'(r\mathbf{x}_i^\top \mathbf{u}) \right),$$

and the statement is trivial for  $r = 0$ . Hence assume  $r > 0$ . If  $\mathbf{x}_i^\top \mathbf{u} > 0$ , then by elementary properties of  $\zeta(\cdot)$ ,  $\zeta'(r\mathbf{x}_i^\top \mathbf{u}) > 1/2$ . On the other hand if  $\mathbf{x}_i^\top \mathbf{u} < 0$ ,  $\zeta'(r\mathbf{x}_i^\top \mathbf{u}) < 1/2$  and if  $\mathbf{x}_i^\top \mathbf{u} = 0$ ,  $\zeta'(r\mathbf{x}_i^\top \mathbf{u}) = 1/2$ . Thus, for  $r > 0$ ,  $\frac{\partial}{\partial r} p(r\mathbf{u}) < 0$  except on a set of measure zero, on which it is  $\leq 0$ . Hence it is sufficient to establish that there exists a constant  $c > 0$ , such that for  $r = c\sqrt{n}$

$$\sup_{\mathbf{u} \in S^{p-1}} p(r\mathbf{u}) < -\frac{1}{\alpha} n \log(2), \quad (\text{S73})$$

with sufficiently high probability. A second order Taylor expansion of  $\zeta(r\mathbf{x}_i^\top \mathbf{u})$  around 0 gives

$$\begin{aligned} \zeta(r\mathbf{x}_i^\top \mathbf{u}) &= \zeta(0) + \zeta'(0)r\mathbf{x}_i^\top \mathbf{u} + \frac{1}{2}\zeta''(\gamma_i)(r\mathbf{x}_i^\top \mathbf{u})^2 \\ &= \log(2) + \frac{1}{2}r\mathbf{x}_i^\top \mathbf{u} + \frac{1}{2}\zeta''(\gamma_i)(r\mathbf{x}_i^\top \mathbf{u})^2, \end{aligned}$$

where  $\gamma_i$  lies between 0 and  $r\mathbf{x}_i^\top \mathbf{u}$ . Hence,

$$\begin{aligned} p(r\mathbf{u}) &= \frac{1-\alpha}{\alpha} \sum_{i=1}^n \frac{1}{2} r\mathbf{x}_i^\top \mathbf{u} - \zeta(r\mathbf{x}_i^\top \mathbf{u}) \\ &= \frac{1-\alpha}{\alpha} \sum_{i=1}^n \left\{ \frac{1}{2} r\mathbf{x}_i^\top \mathbf{u} - \log(2) - \frac{1}{2} r\mathbf{x}_i^\top \mathbf{u} - \frac{1}{2} \zeta''(\gamma_i)(r\mathbf{x}_i^\top \mathbf{u})^2 \right\} \\ &= -\frac{1-\alpha}{\alpha} n \log(2) - \frac{1-\alpha}{2\alpha} \sum_{i=1}^n \zeta''(\gamma_i)(r\mathbf{x}_i^\top \mathbf{u})^2 \\ &\leq -\frac{1-\alpha}{\alpha} n \log(2) - \frac{1-\alpha}{2\alpha} \sum_{i=1}^n \zeta''(r\mathbf{x}_i^\top \mathbf{u})(r\mathbf{x}_i^\top \mathbf{u})^2 \\ &= -\frac{1-\alpha}{\alpha} n \log(2) - \frac{1-\alpha}{2\alpha} (r\mathbf{u})^\top \mathbf{X}^\top \mathbf{W}\{r\mathbf{u}\} \mathbf{X}(r\mathbf{u}), \end{aligned}$$

where  $\mathbf{W}\{r\mathbf{u}\}$  is a diagonal matrix with  $[\mathbf{W}\{r\mathbf{u}\}]_{ii} = \zeta''(r\mathbf{x}_i^\top \mathbf{u})$ . The inequality follows since  $\zeta''(\cdot)$  is positive, symmetric around zero  $\zeta''(x) = \zeta''(-x)$ , and strictly decreasing away from zero so that  $|x| > |y|$  implies  $\zeta''(y) > \zeta''(x)$ . Since  $\gamma_i$  lies between 0 and  $r\mathbf{x}_i^\top \mathbf{u}$ ,  $|\gamma_i| \leq |r\mathbf{x}_i^\top \mathbf{u}|$  and

$\zeta''(\gamma_i) > \zeta''(r\mathbf{x}_i^\top \mathbf{u})$  as required. Hence,

$$\begin{aligned}
\sup_{\mathbf{u} \in S^{p-1}} p(r\mathbf{u}) &\leq -\frac{1-\alpha}{\alpha} n \log(2) + \frac{1-\alpha}{2\alpha} \sup_{\mathbf{u} \in S^{p-1}} - (r\mathbf{u})^\top \mathbf{X}^\top \mathbf{W} \{r\mathbf{u}\} \mathbf{X} (r\mathbf{u}) \\
&= -\frac{1-\alpha}{\alpha} n \log(2) - \frac{1-\alpha}{2\alpha} \inf_{\mathbf{u} \in S^{p-1}} (r\mathbf{u})^\top \mathbf{X}^\top \mathbf{W} \{r\mathbf{u}\} \mathbf{X} (r\mathbf{u}) \\
&\leq -\frac{1-\alpha}{\alpha} n \log(2) - \frac{1-\alpha}{2\alpha} \inf_{\mathbf{v} \in S^{p-1}} \inf_{\mathbf{u} \in S^{p-1}} (r\mathbf{u})^\top \mathbf{X}^\top \mathbf{W} \{r\mathbf{v}\} \mathbf{X} (r\mathbf{u}) \\
&= -\frac{1-\alpha}{\alpha} n \log(2) - \frac{1-\alpha}{2\alpha} r^2 \inf_{\mathbf{v} \in S^{p-1}} \lambda_{\min}(\mathbf{X}^\top \mathbf{W} \{r\mathbf{v}\} \mathbf{X}),
\end{aligned}$$

and thus, to establish (S73) it is sufficient that

$$\frac{1-\alpha}{2\alpha} r^2 \inf_{\mathbf{v} \in S^{p-1}} \lambda_{\min}(\mathbf{X}^\top \mathbf{W} \{r\mathbf{v}\} \mathbf{X}) > n \log(2).$$

By Lemma 7 of Sur *et al.* (2019), there exists a  $\epsilon_0 > 0$  such that for all  $0 < \epsilon \leq \epsilon_0$ ,

$$\inf_{\mathbf{v} \in S^{p-1}} \lambda_{\min}(\mathbf{X}^\top \mathbf{W} \{r\mathbf{v}\} \mathbf{X}) \geq \zeta'' \left( \frac{3r}{\sqrt{\epsilon n}} \right) \left( \sqrt{1-\epsilon} - \sqrt{\frac{p}{n}} - 2\sqrt{\frac{H(\epsilon)}{1-\epsilon}} \right)^2,$$

with probability at least  $1 - 2 \exp\{-nH(\epsilon)\} - 2 \exp\{-n/\epsilon\}$ , where  $H(\epsilon) = -\epsilon \log(\epsilon) - (1-\epsilon) \log(1-\epsilon)$ . Hence, since  $r = c\sqrt{n}$ , for  $0 < \epsilon \leq \epsilon_0$ , we can find constants  $c_1(\epsilon, \kappa), c_2(\epsilon, \kappa), C(\epsilon, \kappa) > 0$ , and  $n_0(\kappa, \epsilon)$  such that for all  $n > n_0(\kappa, \epsilon)$ ,

$$\inf_{\mathbf{v} \in S^{p-1}} \lambda_{\min}(\mathbf{X}^\top \mathbf{W} \{r\mathbf{v}\} \mathbf{X}) \geq \zeta'' \left( \frac{3c}{\sqrt{\epsilon}} \right) C(\epsilon, \kappa),$$

with probability at least  $1 - c_1(\epsilon, \kappa) \exp\{-c_2(\epsilon, \kappa)n\}$ . On that event, for  $\alpha$  small enough

$$\frac{1-\alpha}{2\alpha} r^2 \inf_{\mathbf{v} \in S^{p-1}} \lambda_{\min}(\mathbf{X}^\top \mathbf{W} \{r\mathbf{v}\} \mathbf{X}) \geq \frac{1-\alpha}{2\alpha} c^2 n \zeta'' \left( \frac{3c}{\sqrt{\epsilon}} \right) C(\kappa, \epsilon) > n \log(2).$$

This concludes the proof.  $\square$

**Remark 1.** Note that the proof of Lemma C.1 does not depend on the specification of  $\gamma$ . Hence, the threshold value  $\alpha_0$ , which guarantees boundedness of  $\hat{\beta}^{\text{DY}}$  in  $\ell_2$ -norm also depends solely on  $\kappa$ . A more refined analysis might be able to produce a concrete upper bound of the cutoff value  $\alpha_0(\kappa)$ .

## D Proof of Theorem 3.3

Recall that the setup of Theorems 3.3-3.5 is the moderately high-dimensional setting with i.i.d. Gaussian covariates with arbitrary covariance structure. In particular,  $\mathbf{x}_i \sim \mathcal{N}(\mathbf{0}_p, \mathbf{\Sigma})$  for some positive definite matrix  $\mathbf{\Sigma}$  and signal  $\beta_0 \in \mathbb{R}^p$  such that  $\lim_{n \rightarrow \infty} \text{var}(\mathbf{x}_i^\top \beta_0) = \beta_0^\top \mathbf{\Sigma} \beta_0 = \gamma^2$  for  $\gamma \in \mathbb{R}_{>0}^p$  and where  $\lim_{n \rightarrow \infty} p/n \rightarrow \kappa \in (0, 1)$ .

**Theorem 3.3.** Assume that  $(\alpha, \kappa, \gamma)$  are such that the conditions of Theorem 3.1 are met. Let  $\hat{\beta}^{\text{DY}}$  be the MDYPL estimator for a logistic regression model with i.i.d.  $\mathcal{N}(\mathbf{0}_p, \mathbf{\Sigma})$  covariates, with  $\limsup_{n \rightarrow \infty} \lambda_{\max}(\mathbf{\Sigma})/\lambda_{\min}(\mathbf{\Sigma}) < \infty$ , and signal  $\beta_0$ . Then for any  $t \in \mathbb{R}$ ,

$$\frac{1}{p} \sum_{j=1}^p \mathbb{1} \left\{ \sqrt{n} \tau_j \frac{\hat{\beta}_j^{DY} - \mu_* \beta_{0,j}}{\sigma_*} \leq t \right\} \xrightarrow{p} \Phi(t),$$

where  $\Phi(\cdot)$  is the CDF of a standard normal random variable,  $\mathbb{1}(\cdot)$  is the indicator function and  $\tau_j^2 = \text{var}(\mathbf{x}_{ij} | \mathbf{x}_{i-j})$  is the conditional variance of the  $j$ th predictor given all others. Further, if

$$\frac{1}{p} \sum_{j=1}^p \delta_{\sqrt{n} \tau_j \beta_{0,j}} \xrightarrow{d} \pi_{\bar{\beta}} \quad \text{and} \quad \frac{1}{p} \sum_{j=1}^p n \tau_j^2 \beta_{0,j}^2 \xrightarrow{p} E(\bar{\beta}^2),$$

for some distribution  $\pi_{\bar{\beta}}$  with finite second moment and  $\bar{\beta} \sim \pi_{\bar{\beta}}$ , where  $\delta_{(\cdot)}$  is the Dirac delta function, then for any pseudo-Lipschitz function  $\psi : \mathbb{R}^2 \rightarrow \mathbb{R}$  of order 2,

$$\frac{1}{p} \sum_{j=1}^p \psi \left( \sqrt{n} \tau_j \left( \hat{\beta}_j^{DY} - \mu_* \beta_{0,j} \right), \sqrt{n} \tau_j \beta_{0,j} \right) \xrightarrow{p} E[\psi(\sigma_* G, \bar{\beta})], \quad \text{as } n \rightarrow \infty,$$

for  $G \sim N(0, 1)$  independent of  $\bar{\beta}$ .

The proof of Theorem 3.3 is a replication of the arguments in the proof of Theorem 3.2 in Zhao *et al.* (2022) with the substitutions that are outlined in F. No claim of originality is made.

The following Lemma, which is a generalization of Lemma E.2 to arbitrary covariance structures, is the starting point of the analysis. Let  $\langle \mathbf{u}, \mathbf{v} \rangle_{\Sigma} = \mathbf{u}^\top \Sigma \mathbf{v}$ , and  $\|\mathbf{u}\|_{\Sigma}^2 = \langle \mathbf{u}, \mathbf{u} \rangle_{\Sigma}$ . Then write  $\gamma_n^2 = \|\beta_0\|_{\Sigma}^2 = \text{var}(\mathbf{x}_i^\top \beta_0)$  for  $\mathbf{x}_i \sim \mathcal{N}(\mathbf{0}_p, \Sigma)$ .

**Lemma D.1.** Let  $\hat{\beta}^{DY}$  be the MDYPL estimator from  $\mathcal{N}(\mathbf{0}_p, \Sigma)$  covariates and signal  $\beta_0$ . Define

$$\boldsymbol{\xi} = \mathbf{Z} - \left\langle \mathbf{Z}, \frac{\beta_0}{\gamma_n} \right\rangle_{\Sigma} \frac{\beta_0}{\gamma_n},$$

for  $\mathbf{Z} \sim \mathcal{N}(\mathbf{0}_p, \Sigma^{-1})$  independent of everything else. Further, let

$$\tilde{\mu}_n = \frac{\langle \hat{\beta}^{DY}, \beta_0 \rangle_{\Sigma}}{\|\beta_0\|_{\Sigma}^2}, \quad \tilde{\sigma}_n^2 = \left\| \hat{\beta}^{DY} \right\|_{\Sigma}^2 - \frac{\langle \hat{\beta}^{DY}, \beta_0 \rangle_{\Sigma}^2}{\|\beta_0\|_{\Sigma}^2}.$$

Then

$$\frac{\hat{\beta}^{DY} - \tilde{\mu}_n \beta_0}{\tilde{\sigma}_n} \stackrel{d}{=} \frac{\boldsymbol{\xi}}{\|\boldsymbol{\xi}\|_{\Sigma}}.$$

*Proof.* The proof is similar to the proof of Proposition B.1 in the proof of Theorem 3.2 of Zhao *et al.* (2022) and thus omitted.  $\square$

Lemma D.1 immediately yields the equivalence (S74) below. Define  $\mathbf{T}^{\text{approx}}$  as the  $p$ -vector with elements

$$\mathbf{T}_j^{\text{approx}} = \tau_j \sqrt{n} \frac{\hat{\beta}_j^{DY} - \tilde{\mu}_n \beta_{0,j}}{\tilde{\sigma}_n / \sqrt{\kappa}},$$

which ought to approximate

$$\mathbf{T}_j = \tau_j \sqrt{n} \frac{\hat{\beta}_j^{DY} - \mu_* \beta_{0,j}}{\sigma_*}.$$

Further, let  $\mathbf{Z}_j^{\text{scaled}} = \tau_j \mathbf{Z}_j$ , so that

$$\mathbf{Z}^{\text{scaled}} \sim \mathcal{N}(\mathbf{0}_p, \mathbf{R}), \quad \mathbf{R}_{ij} = \tau_i \tau_j [\Sigma^{-1}]_{ij},$$

and finally let  $\tilde{\mathbf{Z}}^{\text{scaled}}$  be the  $p$ -vector with entries

$$\tilde{\mathbf{Z}}_j^{\text{scaled}} = \left( \mathbf{Z}_j^{\text{scaled}} - \left\langle \mathbf{Z}, \frac{\boldsymbol{\beta}_0}{\gamma_n} \right\rangle_{\boldsymbol{\Sigma}} \frac{\tau_j \boldsymbol{\beta}_{0,j}}{\gamma_n} \right) \frac{\sqrt{p}}{\|\boldsymbol{\xi}\|_{\boldsymbol{\Sigma}}}.$$

Then

$$\mathbf{T}^{\text{approx}} \stackrel{d}{=} \tilde{\mathbf{Z}}^{\text{scaled}}. \quad (\text{S74})$$

The remainder of the proof is concerned with showing that  $\mathbf{T} \approx \mathbf{T}^{\text{approx}}$ ,  $\tilde{\mathbf{Z}}^{\text{scaled}} \approx \mathbf{Z}^{\text{scaled}}$  in an adequate sense and that the empirical CDF of  $\mathbf{Z}^{\text{scaled}}$  converges to that of a standard normal.

**Lemma D.2.** *If  $\limsup_{n \rightarrow \infty} \lambda_{\max}(\boldsymbol{\Sigma})/\lambda_{\min}(\boldsymbol{\Sigma}) < \infty$ , then for any univariate Lipschitz function  $\psi$ ,*

$$\frac{1}{p} \sum_{j=1}^p \left\{ \psi(\tilde{\mathbf{Z}}_j^{\text{scaled}}) - \psi(\mathbf{Z}_j^{\text{scaled}}) \right\} \xrightarrow{p} 0, \quad \frac{1}{p} \sum_{j=1}^p \left\{ \psi(\mathbf{T}_j^{\text{approx}}) - \psi(\mathbf{T}_j) \right\} \xrightarrow{p} 0.$$

*Proof.* First consider the pair  $\tilde{\mathbf{Z}}^{\text{scaled}}, \mathbf{Z}^{\text{scaled}}$  and let  $L$  be the Lipschitz constant of  $\psi$ . By the triangle inequality and the definition of  $\tilde{\mathbf{Z}}^{\text{scaled}}, \mathbf{Z}^{\text{scaled}}$ ,

$$\begin{aligned} \left| \frac{1}{p} \sum_{j=1}^p \left\{ \psi(\tilde{\mathbf{Z}}_j^{\text{scaled}}) - \psi(\mathbf{Z}_j^{\text{scaled}}) \right\} \right| &\leq \frac{1}{p} \sum_{j=1}^p \left| \psi(\tilde{\mathbf{Z}}_j^{\text{scaled}}) - \psi(\mathbf{Z}_j^{\text{scaled}}) \right| \\ &\leq L \frac{1}{p} \sum_{j=1}^p \left| \mathbf{Z}_j^{\text{scaled}} \left( 1 - \frac{\sqrt{p}}{\|\boldsymbol{\xi}\|_{\boldsymbol{\Sigma}}} \right) + \left\langle \mathbf{Z}, \frac{\boldsymbol{\beta}_0}{\gamma_n} \right\rangle_{\boldsymbol{\Sigma}} \frac{\tau_j \boldsymbol{\beta}_{0,j}}{\gamma_n} \frac{\sqrt{p}}{\|\boldsymbol{\xi}\|_{\boldsymbol{\Sigma}}} \right| \\ &\leq L \left| 1 - \frac{\sqrt{p}}{\|\boldsymbol{\xi}\|_{\boldsymbol{\Sigma}}} \right| \frac{1}{p} \sum_{j=1}^p |\mathbf{Z}_j^{\text{scaled}}| + \left| \frac{1}{\gamma_n} \left\langle \mathbf{Z}, \frac{\boldsymbol{\beta}_0}{\gamma_n} \right\rangle_{\boldsymbol{\Sigma}} \right| \frac{L\sqrt{p}}{\|\boldsymbol{\xi}\|_{\boldsymbol{\Sigma}}} \frac{1}{p} \sum_{j=1}^p |\tau_j \boldsymbol{\beta}_{0,j}|. \end{aligned} \quad (\text{S75})$$

Arguments similar to Lemma G.10 establish that  $\sqrt{p}/\|\boldsymbol{\xi}\|_{\boldsymbol{\Sigma}} \rightarrow 1$  almost surely as  $n \rightarrow \infty$ . Further note that  $\langle \mathbf{Z}, \boldsymbol{\beta}_0/\gamma_n \rangle_{\boldsymbol{\Sigma}}/\gamma_n$  is a univariate Gaussian with  $\mathcal{O}(1)$  variance so that it is itself  $\mathcal{O}_p(1)$ . Hence, it is sufficient to show that

$$\frac{1}{p} \sum_{j=1}^p |\mathbf{Z}_j^{\text{scaled}}| = \mathcal{O}_p(1), \quad \frac{1}{p} \sum_{j=1}^p |\tau_j \boldsymbol{\beta}_{0,j}| = o(1). \quad (\text{S76})$$

For the first note that  $\mathbb{E}[|\mathbf{Z}_j^{\text{scaled}}|^2] \leq \mathbb{E}[\mathbf{Z}_j^{\text{scaled}2}] = \tau_j^2 [\boldsymbol{\Sigma}^{-1}]_{jj} \mathbb{E}[\mathbf{Z}_j^2] = 1$  by definition of  $\tau_j$ . Now Markov's inequality (e.g. Vershynin (2018, Proposition 1.2.4)) yields that for  $\epsilon > 0$ ,

$$\Pr \left( \frac{1}{p} \sum_{j=1}^p |\mathbf{Z}_j^{\text{scaled}}| \geq \frac{1}{\epsilon} \right) \leq \epsilon \mathbb{E} \left[ \frac{1}{p} \sum_{j=1}^p |\mathbf{Z}_j^{\text{scaled}}| \right] \leq \epsilon, \quad (\text{S77})$$

so that  $\frac{1}{p} \sum_{j=1}^p |\mathbf{Z}_j^{\text{scaled}}| = \mathcal{O}_p(1)$  indeed. Now, by the Cauchy-Schwarz inequality,

$$\frac{1}{p} \sum_{j=1}^p |\tau_j \boldsymbol{\beta}_{0,j}| = \frac{1}{p} \sum_{j=1}^p |\boldsymbol{\theta}_{0,j}| \leq \frac{1}{\sqrt{p}} \|\boldsymbol{\theta}_0\|_2 = \mathcal{O}(p^{-1/2}), \quad (\text{S78})$$

where  $\boldsymbol{\theta}_0 = \mathbf{L}^\top \boldsymbol{\beta}_0$  for  $\boldsymbol{\Sigma} = \mathbf{L}\mathbf{L}^\top$ , and by assumption  $\|\boldsymbol{\theta}_0\|_2^2 = \text{var}(\mathbf{x}_i^\top \boldsymbol{\beta}_0) \rightarrow \gamma^2$  as  $n \rightarrow \infty$ , for  $\mathbf{x}_i \sim \mathcal{N}(\mathbf{0}_p, \boldsymbol{\Sigma})$ . Hence, (S75) is indeed  $o(1)$ . Next consider  $\mathbf{T}, \mathbf{T}^{\text{approx}}$ .

$$\begin{aligned}
\left| \frac{1}{p} \sum_{j=1}^p \psi(\mathbf{T}_j^{\text{approx}}) - \psi(\mathbf{T}_j) \right| &\leq \frac{1}{p} \sum_{j=1}^p |\psi(\mathbf{T}_j^{\text{approx}}) - \psi(\mathbf{T}_j)| \\
&\leq \frac{L}{\sigma_*} \sqrt{\frac{n}{p}} \frac{1}{\sqrt{p}} \sum_{j=1}^p \left| \tau_j \hat{\beta}_j^{\text{DY}} \left( 1 - \frac{\sqrt{\kappa} \sigma_*}{\tilde{\sigma}_n} \right) + \tau_j \beta_{0,j} \left( \frac{\sqrt{\kappa} \sigma_*}{\tilde{\sigma}_n} \tilde{\mu}_n - \mu_* \right) \right| \\
&\leq \frac{L}{\sigma_*} \sqrt{\frac{n}{p}} \left\{ \left| 1 - \frac{\sqrt{\kappa} \sigma_*}{\tilde{\sigma}_n} \right| \frac{1}{\sqrt{p}} \sum_{j=1}^p |\tau_j \hat{\beta}_j^{\text{DY}}| + \left| \frac{\sqrt{\kappa} \sigma_*}{\tilde{\sigma}_n} \tilde{\mu}_n - \mu_* \right| \frac{1}{\sqrt{p}} \sum_{j=1}^p |\tau_j \beta_{0,j}| \right\}.
\end{aligned} \tag{S79}$$

Now, it follows readily from Lemma E.1 and Lemma E.3 that  $\tilde{\mu}_n \rightarrow \mu_*$  and  $\tilde{\sigma}_n \rightarrow \sigma_*$  almost surely as  $n \rightarrow \infty$ . Indeed, note that by Lemma E.1, one can write

$$\tilde{\mu}_n = \frac{(\hat{\beta}^{\text{DY}})^\top \Sigma \beta_0}{\beta_0^\top \Sigma \beta_0} = \frac{(\mathbf{L}^\top \hat{\beta}^{\text{DY}})^\top (\mathbf{L}^\top \beta_0)}{(\mathbf{L}^\top \beta_0)^\top (\mathbf{L}^\top \beta_0)} = \frac{\langle \hat{\theta}^{\text{DY}}, \theta_0 \rangle}{\|\theta_0\|_2^2},$$

for  $\Sigma = \mathbf{L} \mathbf{L}^\top$  and where  $\hat{\theta}^{\text{DY}}$  is the MDYPL estimator from  $\mathcal{N}(\mathbf{0}_p, \mathbf{I}_p)$  covariates and signal  $\theta_0 = \mathbf{L}^\top \beta_0$ . Hence, immediately by Lemma E.3,  $\tilde{\mu}_n \rightarrow \mu_*$  as  $n \rightarrow \infty$  almost surely and the same applies to  $\tilde{\sigma}_n$ . Secondly, by (S78),  $\frac{1}{\sqrt{p}} \sum_{j=1}^p |\tau_j \beta_{0,j}| = o(1)$ . Finally, recalling that  $\tau_j \hat{\beta}_j^{\text{DY}} = \hat{\theta}_j^{\text{DY}}$ , the Cauchy-Schwarz inequality yields

$$\frac{1}{\sqrt{p}} \sum_{j=1}^p |\tau_j \hat{\beta}_j^{\text{DY}}| = \frac{1}{\sqrt{p}} \sum_{j=1}^p |\hat{\theta}_j^{\text{DY}}| \leq \|\hat{\theta}^{\text{DY}}\|_2, \tag{S80}$$

and by Lemma E.1 and Theorem 3.2,  $\lim_{n \rightarrow \infty} \|\hat{\theta}^{\text{DY}}\|_2 = \mathcal{O}(1)$  almost surely. Thus, (S79) is  $o_p(1)$  as required.  $\square$

Taken together, Lemma D.2 and (S74) imply that

$$\frac{1}{p} \sum_{j=1}^p \psi(\mathbf{T}_j) - \psi(\mathbf{Z}_j^{\text{scaled}}) = o_p(1),$$

so that it remains to characterise the distribution of  $\mathbf{Z}^{\text{scaled}}$ , which is fully characterised by the covariance structure  $\Sigma$ . Zhao *et al.* (2022, Section B.2-B.4) show that if  $\lambda_{\max}(\Sigma)/\lambda_{\min}(\Sigma) = o(\sqrt{p})$ , then the empirical CDF of  $\mathbf{Z}^{\text{scaled}}$  converges pointwise to that of a standard normal random variable in probability, which establishes the first part of the Theorem.

The proof of the second part of the Theorem follows a similar structure as the first part. In particular, for a bivariate pseudo-Lipschitz function  $\psi$  of order two, it is first shown that

$$\frac{1}{p} \sum_{j=1}^p \psi(\sigma_* \mathbf{T}_j, \tau_j \sqrt{n} \beta_{0,j}) - \frac{1}{p} \sum_{j=1}^p \psi(\sigma_* \mathbf{T}_j^{\text{approx}}, \tau_j \sqrt{n} \beta_{0,j}) = o_p(1), \tag{S81}$$

and that

$$\frac{1}{p} \sum_{j=1}^p \psi(\sigma_* \tilde{\mathbf{Z}}_j^{\text{scaled}}, \tau_j \sqrt{n} \beta_{0,j}) - \frac{1}{p} \sum_{j=1}^p \psi(\sigma_* \mathbf{Z}_j^{\text{scaled}}, \tau_j \sqrt{n} \beta_{0,j}) = o_p(1), \tag{S82}$$

which, in conjunction with (S74) yields

$$\frac{1}{p} \sum_{j=1}^p \psi(\sigma_* \mathbf{T}_j, \tau_j \sqrt{n} \beta_{0,j}) - \frac{1}{p} \sum_{j=1}^p \psi(\sigma_* \mathbf{Z}_j^{\text{scaled}}, \tau_j \sqrt{n} \beta_{0,j}) = o_p(1),$$

so that it then remains to analyse

$$\frac{1}{p} \sum_{j=1}^p \psi(\sigma_* \mathbf{Z}_j^{\text{scaled}}, \tau_j \sqrt{n} \beta_{0,j}) . \quad (\text{S83})$$

Towards showing (S81), consider

$$\begin{aligned} & \left| \frac{1}{p} \sum_{j=1}^p \psi(\sigma_* \mathbf{T}_j, \tau_j \sqrt{n} \beta_{0,j}) - \psi(\sigma_* \mathbf{T}_j^{\text{approx}}, \tau_j \sqrt{n} \beta_{0,j}) \right| \\ & \leq \frac{1}{p} \sum_{j=1}^p |\psi(\sigma_* \mathbf{T}_j, \tau_j \sqrt{n} \beta_{0,j}) - \psi(\sigma_* \mathbf{T}_j^{\text{approx}}, \tau_j \sqrt{n} \beta_{0,j})| \\ & \leq \frac{L\sigma_*}{p} \sum_{j=1}^p \left( 1 + \|[\sigma_* \mathbf{T}_j, \tau_j \sqrt{n} \beta_{0,j}]^\top\|_2 + \|[\sigma_* \mathbf{T}_j^{\text{approx}}, \tau_j \sqrt{n} \beta_{0,j}]^\top\|_2 \right) \|\mathbf{T}_j - \mathbf{T}_j^{\text{approx}}\|_2 \\ & \leq \frac{L\sigma_*}{p} \left\{ \sum_{j=1}^p (1 + \sigma_* |\mathbf{T}_j| + \sigma_* |\mathbf{T}_j^{\text{approx}}| + 2\sqrt{n} |\tau_j \beta_{0,j}|)^2 \right\}^{1/2} \left\{ \sum_{j=1}^p (\mathbf{T}_j - \mathbf{T}_j^{\text{approx}})^2 \right\}^{1/2}, \end{aligned}$$

where the last line follows by the Cauchy-Schwarz inequality and the monotonicity of  $\ell_p$  norms. Now by construction of  $\mathbf{T}_j, \mathbf{T}_j^{\text{approx}}$  and since  $(a+b)^2 \leq 2a^2 + 2b^2$ ,

$$\begin{aligned} \sum_{j=1}^p (\mathbf{T}_j - \mathbf{T}_j^{\text{approx}})^2 &= \frac{n}{\sigma_*^2} \sum_{j=1}^p \left( \tau_j \hat{\beta}_j^{\text{DY}} \left( 1 - \frac{\sqrt{\kappa} \sigma_*}{\tilde{\sigma}_n} \right) + \tau_j \beta_{0,j} \left( \frac{\sqrt{\kappa} \sigma_*}{\tilde{\sigma}_n} \tilde{\mu}_n - \mu_* \right) \right)^2 \\ &\leq \frac{2n}{\sigma_*^2} \left\{ \left( 1 - \frac{\sqrt{\kappa} \sigma_*}{\tilde{\sigma}_n} \right)^2 \sum_{j=1}^p (\tau_j \hat{\beta}_j^{\text{DY}})^2 + \left( \frac{\sqrt{\kappa} \sigma_*}{\tilde{\sigma}_n} \tilde{\mu}_n - \mu_* \right)^2 \sum_{j=1}^p (\tau_j \beta_{0,j})^2 \right\} \\ &= \frac{2n}{\sigma_*^2} \left\{ \left( 1 - \frac{\sqrt{\kappa} \sigma_*}{\tilde{\sigma}_n} \right)^2 \|\hat{\boldsymbol{\theta}}^{\text{DY}}\|_2^2 + \left( \frac{\sqrt{\kappa} \sigma_*}{\tilde{\sigma}_n} \tilde{\mu}_n - \mu_* \right)^2 \|\boldsymbol{\theta}_0\|_2^2 \right\} \\ &= o(n), \end{aligned}$$

by considerations similar to those in (S78)-(S80). Similarly, one can bound

$$\begin{aligned} \sum_{j=1}^p (1 + \sigma_* |\mathbf{T}_j| + \sigma_* |\mathbf{T}_j^{\text{approx}}| + 2\sqrt{n} |\tau_j \beta_{0,j}|)^2 &\leq 4 \sum_{j=1}^p 1 + \sigma_*^2 \mathbf{T}_j^2 + \sigma_*^2 \mathbf{T}_j^{\text{approx}2} + 4n \tau_j^2 \beta_{0,j}^2 \\ &= 4n + 4\sigma_*^2 \|\mathbf{T}\|_2^2 + 4\sigma_*^2 \|\mathbf{T}^{\text{approx}}\|_2^2 + 16n \|\boldsymbol{\theta}_0\|_2^2. \end{aligned}$$

Now  $\mathbf{T}_j = \sqrt{n}(\hat{\boldsymbol{\theta}}_j^{\text{DY}} - \mu_* \boldsymbol{\theta}_{0,j})/\sigma_*$  and by considerations analogous to Lemma E.3 and Theorem 3.1, choosing  $\psi(t, u) = t^2$ , yields that  $\|\mathbf{T}\|_2^2 = \mathcal{O}_p(n)$ . Similarly, by Lemma E.3 and the expansion of (S87), also  $\|\mathbf{T}^{\text{approx}}\|_2^2 = \mathcal{O}_p(n)$ . Therefore (S81) is indeed  $o_p(1)$ .

Next, consider the difference (S82). Similarly to above,

$$\begin{aligned} & \left| \frac{1}{p} \sum_{j=1}^p \psi(\sigma_* \tilde{\mathbf{Z}}_j^{\text{scaled}}, \tau_j \sqrt{n} \beta_{0,j}) - \psi(\sigma_* \mathbf{Z}_j^{\text{scaled}}, \tau_j \sqrt{n} \beta_{0,j}) \right| \\ & \leq \frac{L\sigma_*}{p} \left\{ \sum_{j=1}^p (1 + |\mathbf{Z}_j^{\text{scaled}}| + |\tilde{\mathbf{Z}}_j^{\text{scaled}}| + 2\sqrt{n} |\tau_j \beta_{0,j}|)^2 \right\}^{1/2} \left\{ \sum_{j=1}^p (\mathbf{Z}_j^{\text{scaled}} - \tilde{\mathbf{Z}}_j^{\text{scaled}})^2 \right\}^{1/2}. \end{aligned}$$

The term

$$\sum_{j=1}^p (1 + |\mathbf{Z}_j^{\text{scaled}}| + |\tilde{\mathbf{Z}}_j^{\text{scaled}}| + 2\sqrt{n} |\tau_j \beta_{0,j}|)^2 = \mathcal{O}_p(n),$$

since  $\mathbf{T}^{\text{approx}} \stackrel{d}{=} \tilde{\mathbf{Z}}^{\text{scaled}}$ , which was shown to be bounded in the above paragraph and  $\mathbf{Z}^{\text{scaled}}$  was appropriately bounded in (S76)-(S77). On the other hand,

$$\begin{aligned} \sum_{j=1}^p \left( \mathbf{Z}_j^{\text{scaled}} - \tilde{\mathbf{Z}}_j^{\text{scaled}} \right)^2 &= \sum_{j=1}^p \left( \mathbf{Z}_j^{\text{scaled}} \left( 1 - \frac{\sqrt{p}}{\|\boldsymbol{\xi}\|_{\boldsymbol{\Sigma}}} \right) + \frac{\langle \mathbf{Z}, \boldsymbol{\beta}_0 / \gamma_n \rangle_{\boldsymbol{\Sigma}}}{\gamma_n} \tau_j \boldsymbol{\beta}_{0,j} \right)^2 \\ &\leq 2 \left( 1 - \frac{\sqrt{p}}{\|\boldsymbol{\xi}\|_{\boldsymbol{\Sigma}}} \right)^2 \|\mathbf{Z}^{\text{scaled}}\|_2^2 + \left( \frac{\langle \mathbf{Z}, \boldsymbol{\beta}_0 / \gamma_n \rangle_{\boldsymbol{\Sigma}}}{\gamma_n} \right)^2 \left( \frac{\sqrt{p}}{\|\boldsymbol{\xi}\|_{\boldsymbol{\Sigma}}} \right)^2 \|\boldsymbol{\theta}_0\|_2^2 \\ &= o_p(n), \end{aligned}$$

since arguments similar to Lemma G.10 show that  $\lim_{n \rightarrow \infty} \sqrt{p} / \|\boldsymbol{\xi}\|_{\boldsymbol{\Sigma}} = 1$  almost surely,  $\mathbb{E}[\mathbf{Z}_j^{\text{scaled}2}] = 1$  and thus a Markov bound similar to (S76)-(S77) establishes that  $\|\mathbf{Z}^{\text{scaled}}\|_2^2 = \mathcal{O}_p(p)$ . The second term is bounded since additionally  $\lim_{n \rightarrow \infty} \gamma_n^2 = \lim_{n \rightarrow \infty} \|\boldsymbol{\theta}_0\|_2^2 = \gamma^2$ , and  $\langle \mathbf{Z}, \boldsymbol{\beta}_0 / \gamma_n \rangle_{\boldsymbol{\Sigma}}$  is a normal random variable with  $\mathcal{O}(1)$  variance.

Hence, it remains to analyse the behaviour of (S83) which is done in Zhao *et al.* (2022, Lemma C.1). As  $\mathbf{Z}^{\text{scaled}}$  solely depends on  $\boldsymbol{\Sigma}$ , this result directly applies to this setting. The conditions of said Lemma are satisfied in the current setting. Zhao *et al.* (2022, Lemma C.1) establishes that

$$\frac{1}{p} \sum_{j=1}^p \psi(\sigma_* \mathbf{Z}_j^{\text{scaled}}, \tau_j \sqrt{n} \boldsymbol{\beta}_{0,j}) \xrightarrow{p} \mathbb{E}[\psi(\sigma_* G, \bar{\beta})],$$

for  $G \sim \mathcal{N}(0, 1) \perp \bar{\beta}$ . This concludes the proof of the Theorem.

## E Proof of Theorem 3.4

**Theorem 3.4.** Assume that  $(\alpha, \kappa, \gamma)$  are such that the conditions of Theorem 3.1 are met. Let  $\hat{\boldsymbol{\beta}}^{\text{DY}}$  be the MDYPL estimator for a logistic regression model with i.i.d.  $\mathcal{N}(\mathbf{0}_p, \boldsymbol{\Sigma})$  covariates and signal  $\boldsymbol{\beta}_0$ . Then for any regression coefficient such that  $\sqrt{n} \tau_j \boldsymbol{\beta}_{0,j} = \mathcal{O}(1)$ ,

$$\sqrt{n} \tau_j \frac{\hat{\boldsymbol{\beta}}_j^{\text{DY}} - \mu_* \boldsymbol{\beta}_{0,j}}{\sigma_*} \xrightarrow{d} \mathcal{N}(0, 1),$$

where  $\tau_j^2 = \text{var}(\mathbf{x}_{ij} | \mathbf{x}_{i-j})$ .

The proof of Theorem 3.4 is a replication of the arguments in the proof of Theorem 3.1 in Zhao *et al.* (2022) with the substitutions that are outlined in F and follows the general outline given in Section 3.2 of the main paper of this text. No claim of originality is made.

**Lemma E.1.** For any matrix  $\mathbf{L} \in \mathbb{R}^{p \times p}$  and  $\boldsymbol{\Sigma} = \mathbf{L} \mathbf{L}^\top$ , let  $\hat{\boldsymbol{\beta}}^{\text{DY}}$  be the MDYPL estimator from a logistic regression model with i.i.d.  $\mathcal{N}(\mathbf{0}_p, \boldsymbol{\Sigma})$  covariates and signal  $\boldsymbol{\beta}_0$ . Then

$$\hat{\boldsymbol{\theta}}^{\text{DY}} = \mathbf{L}^\top \hat{\boldsymbol{\beta}}^{\text{DY}}$$

is the MDYPL estimator from a logistic regression with  $\mathcal{N}(\mathbf{0}_p, \mathbf{I}_p)$  covariates and signal  $\boldsymbol{\theta}_0 = \mathbf{L}^\top \boldsymbol{\beta}_0$ .

*Proof.* This result follows from the invariance of the MDYPL estimator under linear transformations of the covariates (see for example Zehna (1966)) and the rotational invariance of the normal distribution. Details can be found in Zhao *et al.* 2022, Proposition 2.1.  $\square$

**Lemma E.2.** Let  $\hat{\boldsymbol{\theta}}^{\text{DY}}$  be the MDYPL estimator from a logistic regression model with i.i.d.  $\mathcal{N}(\mathbf{0}_p, \mathbf{I}_p)$  covariates and signal  $\boldsymbol{\theta}_0$ . Define the random variables

$$\mu_n = \frac{\langle \hat{\boldsymbol{\theta}}^{\text{DY}}, \boldsymbol{\theta}_0 \rangle}{\|\boldsymbol{\theta}_0\|_2^2}, \quad \sigma_n = \left\| \mathbf{P}_{\boldsymbol{\theta}_0^\perp} \hat{\boldsymbol{\theta}}^{\text{DY}} \right\|_2, \quad (\text{S84})$$

where  $\mathbf{P}_{\boldsymbol{\theta}_0^\perp}$  is the projection onto  $\boldsymbol{\theta}_0^\perp$ , the orthogonal complement of  $\boldsymbol{\theta}_0$ . Then

$$\frac{\hat{\boldsymbol{\theta}}^{\text{DY}} - \mu_n \boldsymbol{\theta}_0}{\sigma_n}$$

is uniformly distributed on the unit sphere lying in  $\boldsymbol{\theta}_0^\perp$ .

*Proof.* The proof is similar to Zhao *et al.* (2022, Lemma 2.1) and therefore omitted.  $\square$

**Lemma E.3** (Zhao *et al.* (2022), Lemma 3.1). Let  $\hat{\boldsymbol{\beta}}^{\text{DY}}$  be the MDYPL estimator with i.i.d. covariates  $\mathbf{x}_i \sim \mathcal{N}(\mathbf{0}_p, n^{-1} \mathbf{I}_p)$  and assume that the conditions of Theorem 3.1 are met. Then for  $\mu_n, \sigma_n$  as in (S84),

$$\mu_n \xrightarrow{\text{a.s.}} \mu_*, \quad \sigma_n \xrightarrow{\text{a.s.}} \sqrt{\kappa} \sigma_*,$$

where  $(\mu_*, \sigma_*)$  are the solutions corresponding to the system of equations (S3) - (S5).

*Proof.* The proof is similar to the proof of Lemma 3.1 in Zhao *et al.* (2022) and relies on Lemma E.1 and Theorem 3.1.

Given  $\boldsymbol{\theta}_0$  such that  $\lim_{n \rightarrow \infty} \|\boldsymbol{\theta}_0\|_2 = \gamma$ , let  $\hat{\boldsymbol{\beta}}^{\text{DY}}$  be the MDYPL estimator from  $\mathcal{N}(\mathbf{0}_p, n^{-1} \mathbf{I}_p)$  covariates and signal  $\boldsymbol{\beta}_0 = \sqrt{n} \mathbf{U} \boldsymbol{\theta}_0$  where  $\mathbf{U}$  is an orthogonal matrix such that  $\mathbf{U} \boldsymbol{\theta}_0 = (\|\boldsymbol{\theta}_0\|_2, \dots, \|\boldsymbol{\theta}_0\|_2)^\top / \sqrt{p}$ , which can for example be constructed using a Householder transformation. Then by Lemma E.1,  $\hat{\boldsymbol{\beta}}^{\text{DY}} = \sqrt{n} \mathbf{U} \hat{\boldsymbol{\theta}}^{\text{DY}}$  where  $\hat{\boldsymbol{\theta}}^{\text{DY}}$  is the MDYPL estimator with  $\mathcal{N}(\mathbf{0}_p, \mathbf{I}_p)$  covariates and signal  $\boldsymbol{\theta}_0$ . Note that by construction, the empirical distribution of  $\boldsymbol{\beta}_0$  converges to a point mass at  $\gamma/\sqrt{k}$  and that  $\lim_{n \rightarrow \infty} \frac{1}{p} \sum_{j=1}^n \beta_{0,j}^2 = \gamma^2/\kappa$  as required. Hence, Theorem 3.1 gives that for any pseudo-Lipschitz function  $\psi$  of order two,

$$\frac{1}{p} \sum_{j=1}^p \psi(\sqrt{n}([ \mathbf{U} \hat{\boldsymbol{\theta}}^{\text{DY}} ]_j - \mu_* [ \mathbf{U} \boldsymbol{\theta}_0 ]_j), \sqrt{n} [ \mathbf{U} \boldsymbol{\theta}_0 ]_j) \xrightarrow{\text{a.s.}} \mathbb{E}[\psi(\sigma_* G, \bar{\beta})],$$

where  $G \sim \mathcal{N}(0, 1)$ , independent of  $\bar{\beta} \sim \delta_{\gamma/\sqrt{\kappa}}$  and  $\mu_*, \sigma_*$  solve (S3)-(S5). Then choosing  $\psi(x, y) = xy$ , gives that

$$\frac{1}{\kappa} \langle \mathbf{U} \hat{\boldsymbol{\theta}}^{\text{DY}} - \mu_* \mathbf{U} \boldsymbol{\theta}_0, \mathbf{U} \boldsymbol{\theta}_0 \rangle = \frac{1}{\kappa} \langle \hat{\boldsymbol{\theta}}^{\text{DY}} - \mu_* \boldsymbol{\theta}_0, \boldsymbol{\theta}_0 \rangle \xrightarrow{\text{a.s.}} 0,$$

from which it follows that

$$\mu_n = \frac{\langle \hat{\boldsymbol{\theta}}^{\text{DY}}, \boldsymbol{\theta}_0 \rangle}{\|\boldsymbol{\theta}_0\|_2} \xrightarrow{\text{a.s.}} \mu_*. \quad (\text{S85})$$

Similarly, choosing  $\psi(x, y) = x^2$ , gives

$$\frac{1}{\kappa} \langle \mathbf{U} \hat{\boldsymbol{\theta}}^{\text{DY}} - \mu_* \mathbf{U} \boldsymbol{\theta}_0, \mathbf{U} \hat{\boldsymbol{\theta}}^{\text{DY}} - \mu_* \mathbf{U} \boldsymbol{\theta}_0 \rangle = \frac{1}{\kappa} \langle \hat{\boldsymbol{\theta}}^{\text{DY}} - \mu_* \boldsymbol{\theta}_0, \hat{\boldsymbol{\theta}}^{\text{DY}} - \mu_* \boldsymbol{\theta}_0 \rangle = \left\| \hat{\boldsymbol{\theta}}^{\text{DY}} - \mu_* \boldsymbol{\theta}_0 \right\|_2^2 \xrightarrow{\text{a.s.}} \sigma_*^2,$$

which in conjunction with (S85) yields

$$\sigma_n^2 = \left\| \hat{\boldsymbol{\theta}}^{\text{DY}} - \mu_n \boldsymbol{\theta}_0 \right\|_2^2 \xrightarrow{a.s.} \kappa \sigma_*^2$$

as required.  $\square$

Towards proving Theorem 3.4, note that Lemma E.1 implies that for any fixed coordinate  $j$ ,

$$\sqrt{n} \tau_j \frac{\hat{\beta}_j^{\text{DY}} - \mu_* \beta_{0,j}}{\sigma_*} = \sqrt{n} \frac{\hat{\boldsymbol{\theta}}_j^{\text{DY}} - \mu_* \boldsymbol{\theta}_{0,j}}{\sigma_*}, \quad (\text{S86})$$

where  $\hat{\boldsymbol{\theta}}^{\text{DY}} = \mathbf{L}^\top \hat{\boldsymbol{\beta}}^{\text{DY}}$ , is the MDYPL estimator from  $\mathcal{N}(\mathbf{0}_p, \mathbf{I}_p)$  covariates with signal  $\boldsymbol{\theta}_0 = \mathbf{L}^\top \boldsymbol{\beta}_0$  for  $\mathbf{L}$  being the Cholesky factorization of  $\boldsymbol{\Sigma} = \mathbf{L}\mathbf{L}^\top$  and where  $\tau_j^2 = \text{var}(\mathbf{x}_{ij} | \mathbf{x}_{i,-j})$  is the conditional variance of the  $j$ th covariate given all other covariates under  $\boldsymbol{\Sigma}$  (see Zhao *et al.* (2022, Section 2.1)).

A simple expansion of the RHS of (S86) gives

$$\sqrt{n} \frac{\hat{\boldsymbol{\theta}}_j^{\text{DY}} - \mu_* \boldsymbol{\theta}_{0,j}}{\sigma_*} = \sqrt{n} \frac{\hat{\boldsymbol{\theta}}_j^{\text{DY}} - \mu_n \boldsymbol{\theta}_{0,j}}{\sigma_n} \frac{\sigma_n}{\sigma_*} + \sqrt{n} \frac{(\mu_n - \mu_*) \boldsymbol{\theta}_{0,j}}{\sigma_*}. \quad (\text{S87})$$

Now by the assumption of the Theorem,  $\sqrt{n} \boldsymbol{\theta}_{0,j} = \sqrt{n} \tau_j \boldsymbol{\beta}_{0,j} = \mathcal{O}(1)$ . Hence, by Lemma E.3, the second term on the RHS of (S87) is  $o(1)$  almost surely. Now by Lemma E.2,  $(\hat{\boldsymbol{\theta}}_j^{\text{DY}} - \mu_n \boldsymbol{\theta}_{0,j})/\sigma_n = \mathbf{P}_{\boldsymbol{\theta}_0^\perp} \hat{\boldsymbol{\theta}}^{\text{DY}} / \|\mathbf{P}_{\boldsymbol{\theta}_0^\perp} \hat{\boldsymbol{\theta}}^{\text{DY}}\|_2$  is distributed uniformly on the unit sphere lying in  $\boldsymbol{\theta}_0^\perp$ , where  $\mathbf{P}_{\boldsymbol{\theta}_0^\perp}$  is the projection matrix into the orthogonal complement  $\boldsymbol{\theta}_0^\perp$  of  $\boldsymbol{\theta}_0$ . It is a well known property of the Gaussian distribution that for  $\mathbf{Z} \sim \mathcal{N}(\mathbf{0}_p, \mathbf{I}_p)$ , the projection onto the unit sphere is uniformly distributed (see for example Vershynin (2018), Section 3.3.3), and thus by Lemma E.2,

$$\frac{\mathbf{P}_{\boldsymbol{\theta}_0^\perp} \hat{\boldsymbol{\theta}}^{\text{DY}}}{\|\mathbf{P}_{\boldsymbol{\theta}_0^\perp} \hat{\boldsymbol{\theta}}^{\text{DY}}\|_2} \stackrel{d}{=} \frac{\mathbf{P}_{\boldsymbol{\theta}_0^\perp} \mathbf{Z}}{\|\mathbf{P}_{\boldsymbol{\theta}_0^\perp} \mathbf{Z}\|_2},$$

for  $\mathbf{Z} \sim \mathcal{N}(\mathbf{0}_p, \mathbf{I}_p)$ . Expanding  $\mathbf{P}_{\boldsymbol{\theta}_0^\perp} \mathbf{Z}$  as

$$\mathbf{P}_{\boldsymbol{\theta}_0^\perp} \mathbf{Z} = \mathbf{Z} - \left\langle \mathbf{Z}, \frac{\boldsymbol{\theta}_0}{\|\boldsymbol{\theta}_0\|_2} \right\rangle \frac{\boldsymbol{\theta}_0}{\|\boldsymbol{\theta}_0\|_2},$$

whose  $j$ th component is thus given by

$$Z_j \left( 1 - \frac{\boldsymbol{\theta}_{0,j}^2}{\|\boldsymbol{\theta}_0\|_2^2} \right) + \xi,$$

where  $Z_j$  is the  $j$ th component of  $\mathbf{Z}$  and  $\xi$  is a normal random variable independent of  $Z_j$  with mean zero and variance

$$\text{var}(\xi) = \frac{\|\boldsymbol{\theta}_{0,-j}\|_2^2}{\|\boldsymbol{\theta}_0\|_2^2} \frac{\boldsymbol{\theta}_{0,j}^2}{\|\boldsymbol{\theta}_0\|_2^2} = \mathcal{O}(n^{-1}),$$

since  $\sqrt{n} \boldsymbol{\theta}_j = \mathcal{O}(1)$ . Consequently  $\xi = \mathcal{O}_p(n^{-1/2})$ . Further, by Lemma G.10,  $\|\mathbf{P}_{\boldsymbol{\theta}_0^\perp} \mathbf{Z}\|_2 / \sqrt{p} \rightarrow 1$  almost

surely. Hence, taken together, one gets that

$$\begin{aligned}
\sqrt{n} \frac{\hat{\boldsymbol{\theta}}_j^{\text{DY}} - \mu_* \boldsymbol{\theta}_{0,j}}{\sigma_*} &= \sqrt{n} \frac{\hat{\boldsymbol{\theta}}_j^{\text{DY}} - \mu_n \boldsymbol{\theta}_{0,j}}{\sigma_n} \frac{\sigma_n}{\sigma_*} + \sqrt{n} \frac{(\mu_n - \mu_*) \boldsymbol{\theta}_{0,j}}{\sigma_*} \\
&= \sqrt{n} \frac{\hat{\boldsymbol{\theta}}_j^{\text{DY}} - \mu_n \boldsymbol{\theta}_{0,j}}{\sigma_n} \frac{\sigma_n}{\sigma_*} + o_p(1) \\
&= \sqrt{n} \frac{\hat{\boldsymbol{\theta}}_j^{\text{DY}} - \mu_n \boldsymbol{\theta}_{0,j}}{\sigma_n} + o_p(1) \\
&\stackrel{d}{=} \sqrt{\frac{n}{p}} \frac{\|\mathbf{P}_{\boldsymbol{\theta}_0^\perp} \mathbf{Z}\|_2}{\sqrt{p}} \left\{ Z_j \left( 1 - \frac{\boldsymbol{\theta}_{0,j}^2}{\|\boldsymbol{\theta}_0\|_2^2} \right) + \xi \right\} + o_p(1) \\
&= \frac{1}{\sqrt{\kappa}} \left\{ Z_j \left( 1 - \frac{\boldsymbol{\theta}_{0,j}^2}{\|\boldsymbol{\theta}_0\|_2^2} \right) + \xi \right\} + o_p(1) \\
&= \frac{1}{\sqrt{\kappa}} Z_j \sigma_j + o_p(1) \\
&= \frac{1}{\sqrt{\kappa}} Z_j + o_p(1)
\end{aligned}$$

for  $\sigma_j = 1 - \boldsymbol{\theta}_{0,j}^2 / \|\boldsymbol{\theta}_0\|_2^2$  which converges to one since  $\boldsymbol{\theta}_{0,j} = \mathcal{O}(n^{-1/2})$ . By (S86) and (S87),

$$\sqrt{n} \frac{\hat{\boldsymbol{\theta}}_j^{\text{DY}} - \mu_* \boldsymbol{\theta}_{0,j}}{\sigma_*} \stackrel{d}{=} \frac{1}{\sqrt{\kappa}} Z_j + o_p(1), \quad (\text{S88})$$

and the first part of the Theorem follows. The general result follows from (S88) and the rotational invariance of the Gaussian distribution in conjunction with Lemma E.1. The argument is completely similar to the one provided in the proof of Theorem 3.1 in Zhao *et al.* (2022) starting below (A.6) and is thus omitted.

## F Proof of Theorem 3.5

**Theorem 3.5.** Let  $\hat{\boldsymbol{\beta}}^{\text{DY}}$  be the MDYPL estimator for a logistic regression model with i.i.d.  $\mathcal{N}(\mathbf{0}_p, \boldsymbol{\Sigma})$  covariates and signal  $\boldsymbol{\beta}_0$ . Assume that  $(\alpha, \kappa, \gamma)$  are such that  $\|\hat{\boldsymbol{\beta}}^{\text{DY}}\|_2 = \mathcal{O}(n^{1/2})$  almost surely and that (S3)-(S5) admit a solution  $(\mu_*, b_*, \sigma_*)$  such that  $\mathbf{J}(\mu_*, b_*, \sigma_*)$  is nonsingular. Consider a fixed subset of indices  $I = \{i_1, \dots, i_k\}$ , and the DY prior penalized likelihood ratio test statistic

$$\Lambda_I = \max_{\boldsymbol{\beta} \in \mathbb{R}^p} \ell(\boldsymbol{\beta}; \mathbf{y}^*, \mathbf{X}) - \max_{\substack{\boldsymbol{\beta} \in \mathbb{R}^p: \\ \beta_j = 0, j \in I}} \ell(\boldsymbol{\beta}; \mathbf{y}^*, \mathbf{X}).$$

Then, under the null that  $\beta_{0,i_1} = \dots = \beta_{0,i_k} = 0$ ,  $\Lambda_I$  is asymptotically distributed as

$$2\Lambda_I \xrightarrow{d} \frac{\kappa \sigma_*^2}{b_*} \chi_k^2,$$

where  $\chi_k^2$  is a Chi-squared random variable with  $k$  degrees of freedom.

This follows immediately from Theorem F.1 and Lemma E.1 as in the discussion of Zhao *et al.* (2022, Section 4).

**Theorem F.1.** Let  $\hat{\boldsymbol{\beta}}^{\text{DY}}$  be the MDYPL estimator for a logistic regression model with i.i.d.  $\mathcal{N}(\mathbf{0}_p, n^{-1} \mathbf{I}_p)$  covariates and signal  $\boldsymbol{\beta}_0$ . Assume that  $(\alpha, \kappa, \gamma)$  are such that  $\|\hat{\boldsymbol{\beta}}^{\text{DY}}\|_2 = \mathcal{O}(n^{1/2})$  almost surely and that (S3)-(S5) admit a solution  $(\mu_*, b_*, \sigma_*)$  such that  $\mathbf{J}(\mu_*, b_*, \sigma_*)$  is nonsingular. Consider a fixed subset of

indices  $I = \{i_1, \dots, i_k\}$ , and the DY prior penalized likelihood ratio test statistic

$$\Lambda_I = \max_{\beta \in \mathbb{R}^p} \ell(\beta; \mathbf{y}^*, \mathbf{X}) - \max_{\substack{\beta \in \mathbb{R}^p: \\ \beta_j = 0, j \in I}} \ell(\beta; \mathbf{y}^*, \mathbf{X}).$$

Then, under the null that  $\beta_{0,i_1} = \dots = \beta_{0,i_k} = 0$ ,  $\Lambda_I$  is asymptotically distributed as

$$2\Lambda_I \xrightarrow{d} \frac{\kappa \sigma_*^2}{b_*} \chi_k^2,$$

where  $\chi_k^2$  is a Chi-squared random variable with  $k$  degrees of freedom.

The proof of Theorem F.1 is analogous the proof of Theorem 3 in Sur and Candès (2019) where the MLE is replaced with the MDYPL estimator, the state evolutions in (5) are replaced by (S3)-(S5) and the standard logistic regression log-likelihood  $\ell(\beta; \mathbf{y}, \mathbf{X})$  is replaced by the log-likelihood with pseudo responses  $\mathbf{y}^*$ , i.e.  $\ell(\beta; \mathbf{y}^*, \mathbf{X})$  and their Theorem 2 is replaced by Theorem 3.1. A line by line analysis reveals that the arguments in the proof of Sur and Candès (2019) go through with minuscule adjustments. As the proof is lengthy and technical, and there are no noteworthy contributions in the adaptation to the MDYPL estimator, it is omitted.

## G Auxiliary Lemmas

**Lemma G.1.** *Given  $\epsilon > 0$ ,  $\alpha \in [0, 1]$ , consider the approximation  $h_\epsilon(Z, \bar{\epsilon}) = \frac{\alpha}{2} \left\{ 1 - \frac{\bar{\epsilon} - \zeta'(Z)}{|\bar{\epsilon} - \zeta'(Z)| + \epsilon} \right\} + \frac{1-\alpha}{2}$  to  $h(Z, \bar{\epsilon}) = \frac{\alpha}{2} \{1 - \text{sign}(\bar{\epsilon} - \zeta'(Z))\} + \frac{1-\alpha}{2}$ . Then*

i)  $\lim_{\epsilon \rightarrow 0} h_\epsilon(Z, \bar{\epsilon}) = h(Z, \bar{\epsilon})$  for all  $Z, \bar{\epsilon}$

ii)  $h_\epsilon(Z, \bar{\epsilon})$  is Lipschitz in  $[Z, \bar{\epsilon}]^\top$

iii)  $\frac{\partial}{\partial Z} h_\epsilon(Z, \bar{\epsilon})$  exists for all  $Z, \bar{\epsilon} \in \mathbb{R}$ ,  $\epsilon > 0$  and is Lipschitz in  $[Z, \bar{\epsilon}]^\top$ .

*Proof.* i) If  $\bar{\epsilon} - \zeta'(Z) = 0$ , then  $h_\epsilon(Z, \bar{\epsilon}) = 0$  for all  $\epsilon > 0$ . If  $\bar{\epsilon} - \zeta'(Z) \neq 0$ , then  $\lim_{\epsilon \rightarrow 0} h_\epsilon(Z, \bar{\epsilon}) = (\bar{\epsilon} - \zeta'(Z))/|\bar{\epsilon} - \zeta'(Z)| = \text{sign}(\bar{\epsilon} - \zeta'(Z))$ . The claim follows.

ii) First it is shown that  $f(x) = x/(|x| + \epsilon)$  is Lipschitz for any  $\epsilon > 0$  with Lipschitz constant  $\epsilon^{-1}$ . To that end, note that  $\frac{\partial}{\partial x} f(x) = \epsilon/(|x| + \epsilon)^2 \leq \epsilon^{-1}$  and by the mean value theorem (e.g. Rudin 1976, Theorem 5.10),

$$|f(x) - f(y)| \leq \sup_{z \in \mathbb{R}} \left| \frac{\partial}{\partial z} f(z) \right| |x - y| \leq \frac{1}{\epsilon} |x - y|.$$

Further, note that  $\zeta''(x)$  is positive and bounded from above by  $1/4$ . Hence,

$$\begin{aligned}
|h_\epsilon(Z, \bar{\epsilon}) - h_\epsilon(Z', \bar{\epsilon}')| &= \frac{\alpha}{2} |f(\bar{\epsilon} - \zeta'(Z)) - f(\bar{\epsilon}' - \zeta'(Z'))| \\
&\leq \frac{\alpha}{2\epsilon} |\bar{\epsilon} - \zeta'(Z) - (\bar{\epsilon}' - \zeta'(Z'))| \\
&\leq \frac{\alpha}{2\epsilon} \{|\bar{\epsilon} - \bar{\epsilon}'| + |\zeta'(Z) - \zeta'(Z')|\} \\
&\leq \frac{\alpha}{2\epsilon} \left\{ |\bar{\epsilon} - \bar{\epsilon}'| + \frac{1}{4} |Z - Z'| \right\} \\
&\leq \frac{\alpha}{8\epsilon} \{|\bar{\epsilon} - \bar{\epsilon}'| + |Z - Z'|\} \\
&\leq \frac{\alpha\sqrt{2}}{8\epsilon} \left\| \begin{bmatrix} Z \\ \bar{\epsilon} \end{bmatrix} - \begin{bmatrix} Z' \\ \bar{\epsilon}' \end{bmatrix} \right\|_2,
\end{aligned}$$

where the first inequality follows by Lipschitzianity of  $f(\cdot)$ , the second by the triangle inequality, the third by the Mean Value Theorem and since  $\sup_{x \in \mathcal{R}} |\zeta''(x)| \leq 1/4$ , and the last since  $(|a| + |b|)^2 \leq 2(|a|^2 + |b|^2)$ .

iii) Existence follows by differentiability of  $f(x)$  and the chain rule,

$$\frac{\partial}{\partial Z} h_\epsilon(Z, \bar{\epsilon}) = \frac{\alpha}{2} \frac{\epsilon}{(|\bar{\epsilon} - \zeta'(Z)| + \epsilon)^2} \zeta''(Z). \quad (\text{S89})$$

Next, it is shown that  $f'(x) = \frac{\partial}{\partial x} x/(|x| + \epsilon) = \epsilon/(|x| + \epsilon)^2$  is Lipschitz in  $x$ .

Case 1:  $x, y > 0$ : For  $x > 0$ , the function simplifies to

$$f'(x) = \frac{\epsilon}{(x + \epsilon)^2}.$$

Differentiating with respect to  $x$  yields

$$f''(x) = \frac{-2\epsilon}{(x + \epsilon)^3},$$

which exists for all  $x > 0$ , and it is continuous and monotonically increasing in  $x$ . Furthermore, as  $x$  approaches infinity,  $f''(x)$  approaches 0, and as  $x$  approaches 0 from the right,  $f'(x)$  approaches  $-2/\epsilon^2$ . Thus,  $|f''(x)|$  is bounded by  $\frac{2}{\epsilon^2}$  for all  $x > 0$ .

By the Mean Value Theorem it follows that

$$|f'(x) - f'(y)| \leq \frac{2}{\epsilon^2} |x - y|.$$

Case 2:  $x > 0, y < 0$ : Note that

$$|f'(x) - f'(y)| = \left| \frac{\epsilon}{(x + \epsilon)^2} - \frac{\epsilon}{(-y + \epsilon)^2} \right| = \left| \frac{\epsilon}{(x + \epsilon)^2} - \frac{\epsilon}{(z + \epsilon)^2} \right| = |f'(x) - f'(z)|,$$

for  $z = -y > 0$ . Thus analogous to Case 1,

$$|f'(x) - f'(z)| \leq \frac{2}{\epsilon^2} |x - z| < \frac{2}{\epsilon^2} |x + z| = \frac{2}{\epsilon^2} |x - y|,$$

since  $z = -y > 0, x > 0$ .

Case 3:  $x > 0, y = 0$   
The difference  $|f'(x) - \epsilon^{-1}|$  simplifies to

$$\frac{x^2 + 2\epsilon x}{x^2 + 2\epsilon x + \epsilon^2}.$$

This expression is less than  $Cx$  if and only if

$$x^2 + 2\epsilon x \leq Cx^3 + 2C\epsilon x^2 + C\epsilon^2 x.$$

A sufficient condition for this inequality is  $C > 2/\epsilon$ .

Case 4:  $x, y < 0$

By symmetry, the function behaves the same way for  $x, y < 0$  as it does for  $x, y > 0$ . Thus, the Lipschitz constant derived for  $x, y > 0$  also applies here.

This establishes that  $f'(x)$  is indeed Lipschitz in  $x$  for all  $x \in \mathbb{R}$ . Claim (iii) follows since  $\zeta''(x)$  is Lipschitz in  $x$  and  $\bar{\epsilon} - \zeta'(Z)$  is Lipschitz in both  $Z, \bar{\epsilon}$  and by (S89).  $\square$

**Lemma G.2.** *The following facts hold for the proximal operator  $\text{prox}_{b\zeta}(x)$  and the function  $\Psi(y, s) = b(y - \text{prox}_{b\zeta}(by + s))$ :*

i) *The proximal operator  $\text{prox}_{b\zeta}(x)$  is nonexpansive, i.e. for  $x, x' \in \mathbb{R}$ :*

$$|\text{prox}_{b\zeta}(x) - \text{prox}_{b\zeta}(x')| \leq |x - x'|.$$

ii)  *$\Psi(h_\epsilon(Z, \bar{\epsilon}), s) = b(h_\epsilon(Z, \bar{\epsilon}) - \zeta'(\text{prox}_{b\zeta}(bh_\epsilon(Z, \bar{\epsilon}) + s)))$  is Lipschitz continuous in  $[Z, s, \bar{\epsilon}]^\top$ .*

iii)  *$\Psi(y, s) = b(y - \zeta'(\text{prox}_{b\zeta}(by + s)))$  is Lipschitz continuous in  $s$  with Lipschitz constant at most 1.*

iv)  *$\frac{\partial}{\partial Z}\Psi(h_\epsilon(Z, \bar{\epsilon}), s)$  exists for all  $Z, \bar{\epsilon}, s \in \mathbb{R}$ ,  $\epsilon > 0$  and is Lipschitz*

*Proof.* i) Note that  $\zeta(x)$  is proper, closed and convex (see e.g. Beck 2017, Chapter 2, for the definition). Indeed, properness of  $\zeta(x) : \mathbb{R} \rightarrow [\infty, \infty]$  follows since it is monotonically increasing in  $x$ ,  $\lim_{x \rightarrow \infty} \zeta(x) = 0$  and  $f(0) = 1$ . Closedness follows since lower semicontinuity is equivalent to closedness (e.g. Beck 2017, Theorem 2.6) and  $\zeta(x)$  is clearly continuous and therefore closed. Hence the claim follows by nonexpansivity of the proximal operator for proper, closed and convex functions (see for example Beck 2017, Theorem 6.4.2b)), for  $x, x' \in \mathbb{R}$ ,

$$|\text{prox}_{b\zeta}(x) - \text{prox}_{b\zeta}(x')| \leq |x - x'|.$$

ii) It is shown in Lemma G.1 ii) that the approximation  $h_\epsilon$  is Lipschitz.

By nonexpansivity of the proximal operator, which is shown in Lemma G.2 i),

$$|\text{prox}_{b\zeta}(x) - \text{prox}_{b\zeta}(x')| \leq |x - x'|.$$

Now letting  $x = bh_\epsilon(Z, \bar{\epsilon}) + s$ ,  $x' = bh_\epsilon(Z', \bar{\epsilon}') + s'$  then by Lipschitzianity of  $h_\epsilon$ , and the triangle inequality and Jensen's inequality, again

$$\begin{aligned} |\text{prox}_{b\zeta}(bh_\epsilon(Z, \bar{\epsilon}) + s) - \text{prox}_{b\zeta}(bh_\epsilon(Z', \bar{\epsilon}') + s')| &\leq |b(h_\epsilon(Z, \bar{\epsilon}) - h_\epsilon(Z', \bar{\epsilon}')) + (s - s')| \\ &\leq bL\{|\bar{\epsilon} - \bar{\epsilon}'| + |Z - Z'|\} + |s - s'| \\ &\leq \max\{bL, 1\}\{|\bar{\epsilon} - \bar{\epsilon}'| + |Z - Z'| + |s - s'|\} \\ &\leq \sqrt{3} \max\{bL, 1\} \|[Z, \bar{\epsilon}, s]^\top - [Z', \bar{\epsilon}', s']^\top\|_2, \end{aligned}$$

for some constant  $L$ . Hence, again by boundedness of  $\frac{\partial^2}{\partial x^2} \zeta(x)$ , it immediately follows that for any  $t \in [q]$ ,  $\mathbf{x}, \mathbf{x}', \mathbf{y}, \mathbf{y}' \in \mathfrak{R}^q$ , and  $b > 0$ , note that

$$\begin{aligned}
& |\Psi(h_\epsilon(Z, \bar{\epsilon}), s) - \Psi(h_\epsilon(Z', \bar{\epsilon}'), s')| \\
& \leq b |h_\epsilon(Z, \bar{\epsilon}) - h_\epsilon(Z', \bar{\epsilon}')| \\
& + b |\zeta'(\text{prox}_{b\zeta}(bh_\epsilon(Z, \bar{\epsilon}) + s)) - \zeta'(\text{prox}_{b\zeta}(bh_\epsilon(Z', \bar{\epsilon}') + s'))| \\
& \leq bL \{|\bar{\epsilon} - \bar{\epsilon}'| + |Z - Z'|\} + \\
& \quad \frac{b}{4} \max\{bL, 1\} \{|\bar{\epsilon} - \bar{\epsilon}'| + |Z - Z'| + |s - s'|\} \\
& = \left(bL + \frac{b}{4} \max\{bL, 1\}\right) \{|\bar{\epsilon} - \bar{\epsilon}'| + |Z - Z'|\} + \frac{b}{4} \max\{bL, 1\} |s - s'| \\
& \leq \sqrt{3} \left(bL + \frac{b}{4} \max\{bL, 1\}\right) \|[Z, s, \bar{\epsilon}]^\top - [Z', s', \bar{\epsilon}']^\top\|_2.
\end{aligned}$$

iii) From Donoho and Montanari (2016), Proposition 6.3,

$$\frac{\partial}{\partial s} \Psi(y, s) = -\frac{b\zeta''(\text{prox}_{b\zeta}(by + s))}{1 + b\zeta''(\text{prox}_{b\zeta}(by + s))}, \quad (\text{S90})$$

which is less than one in absolute value and the claim follows by the mean value theorem.

iv) By Proposition 6.3 of Donoho and Montanari (2016), the proximal operator  $\text{prox}_{b\zeta}(x)$  is differentiable for  $b > 0$ ,  $x \in \mathfrak{R}$  with partial derivative

$$\frac{\partial}{\partial x} \text{prox}_{b\zeta}(x) = \frac{1}{1 + b\zeta''(z)} \Big|_{z=\text{prox}_{b\zeta}(x)}.$$

Consequently,

$$\frac{\partial}{\partial x} \zeta'(\text{prox}_{b\zeta}(x)) = \frac{b\zeta''(z)}{1 + b\zeta''(z)} \Big|_{z=\text{prox}_{b\zeta}(x)},$$

and thus using Lemma G.1 iii), and the chain rule,

$$\begin{aligned}
\frac{\partial}{\partial Z} \Psi(h_\epsilon(Z, \bar{\epsilon}), s) &= \frac{\partial}{\partial y} \Psi(y, s) \Big|_{y=h_\epsilon(Z, \bar{\epsilon})} \frac{\partial}{\partial Z} h_\epsilon(Z, \bar{\epsilon}) \\
&= b \left(1 - \frac{b\zeta''(\text{prox}_{b\zeta}(bh_\epsilon(Z, \bar{\epsilon}) + s))}{1 + b\zeta''(\text{prox}_{b\zeta}(bh_\epsilon(Z, \bar{\epsilon}) + s))}\right) \frac{\partial}{\partial Z} h_\epsilon(Z, \bar{\epsilon}) \\
&= \frac{b}{1 + b\zeta''(\text{prox}_{b\zeta}(bh_\epsilon(Z, \bar{\epsilon}) + s))} \frac{\partial}{\partial Z} h_\epsilon(Z, \bar{\epsilon})
\end{aligned}$$

Thus by simple expansion and the triangle inequality,

$$\begin{aligned}
& \left| \frac{\partial}{\partial Z} \Psi(h_\epsilon(Z, \bar{\epsilon}), s) - \frac{\partial}{\partial Z} \Psi(h_\epsilon(Z', \bar{\epsilon}'), s') \right| \\
&= b \left| \left\{ \frac{1}{1 + b\zeta''(\text{prox}_{b\zeta}(bh_\epsilon(Z, \bar{\epsilon}) + s))} - \frac{1}{1 + b\zeta''(\text{prox}_{b\zeta}(bh_\epsilon(Z', \bar{\epsilon}') + s'))} \right\} \frac{\partial}{\partial Z} h_\epsilon(Z, \bar{\epsilon}) \right. \\
&\quad \left. + \frac{1}{1 + b\zeta''(\text{prox}_{b\zeta}(bh_\epsilon(Z', \bar{\epsilon}') + s'))} \left\{ \frac{\partial}{\partial Z} h_\epsilon(Z', \bar{\epsilon}') - \frac{\partial}{\partial Z} h_\epsilon(Z, \bar{\epsilon}) \right\} \right| \\
&\leq b \left| \frac{b}{1 + b\zeta''(\text{prox}_{b\zeta}(bh_\epsilon(Z, \bar{\epsilon}) + s))} - \frac{1}{1 + b\zeta''(\text{prox}_{b\zeta}(bh_\epsilon(Z', \bar{\epsilon}') + s'))} \right| \left| \frac{\partial}{\partial Z} h_\epsilon(Z, \bar{\epsilon}) \right| \\
&\quad + b \left| \frac{1}{1 + b\zeta''(\text{prox}_{b\zeta}(bh_\epsilon(Z', \bar{\epsilon}') + s'))} \right| \left| \frac{\partial}{\partial Z} h_\epsilon(Z', \bar{\epsilon}') - \frac{\partial}{\partial Z} h_\epsilon(Z, \bar{\epsilon}) \right|. \quad (\text{S91})
\end{aligned}$$

Now it is easily seen that the function  $f(x) = 1/(1+x)$  is Lipschitz over the nonnegative real line as it is differentiable and its derivative  $\frac{\partial}{\partial x} f(x) = -1/(1+x)^2$  is bounded from above by 1 in absolute value for  $x \geq 0$ . Further, it is easily seen that  $\frac{\partial}{\partial Z} h_\epsilon(Z, \bar{\epsilon})$  is bounded in absolute value. Hence, using boundedness of  $\zeta'''(x)$ , Lemma G.1 ii) and Lemma G.2 i), it follows immediately that

$$\begin{aligned}
& b \left| \frac{1}{1 + b\zeta''(\text{prox}_{b\zeta}(bh_\epsilon(Z, \bar{\epsilon}) + s))} - \frac{1}{1 + b\zeta''(\text{prox}_{b\zeta}(bh_\epsilon(Z', \bar{\epsilon}') + s'))} \right| \left| \frac{\partial}{\partial Z} h_\epsilon(Z, \bar{\epsilon}) \right| \\
&\leq bC \left| \frac{1}{1 + b\zeta''(\text{prox}_{b\zeta}(bh_\epsilon(Z, \bar{\epsilon}) + s))} - \frac{1}{1 + b\zeta''(\text{prox}_{b\zeta}(bh_\epsilon(Z', \bar{\epsilon}') + s'))} \right| \\
&\leq b^2 C C' |\zeta''(\text{prox}_{b\zeta}(bh_\epsilon(Z, \bar{\epsilon}) + s)) - \zeta''(\text{prox}_{b\zeta}(bh_\epsilon(Z', \bar{\epsilon}') + s'))| \\
&\leq b^2 C C' C'' |\text{prox}_{b\zeta}(bh_\epsilon(Z, \bar{\epsilon}) + s) - \text{prox}_{b\zeta}(bh_\epsilon(Z', \bar{\epsilon}') + s')| \\
&\leq b^2 C C' C'' C''' \|[Z, s, \bar{\epsilon}]^\top - [Z', s', \bar{\epsilon}']^\top\|,
\end{aligned}$$

for some positive constants  $C, C', C'', C'''$ . Similarly, by nonnegativity of  $\zeta''$  and  $b$ , as well as Lemma G.1 iii),

$$\begin{aligned}
& b \left| \frac{1}{1 + b\zeta''(\text{prox}_{b\zeta}(bh_\epsilon(Z', \bar{\epsilon}') + s'))} \right| \left| \frac{\partial}{\partial Z} h_\epsilon(Z', \bar{\epsilon}') - \frac{\partial}{\partial Z} h_\epsilon(Z, \bar{\epsilon}) \right| \\
&\leq bC \left| \frac{\partial}{\partial Z} h_\epsilon(Z', \bar{\epsilon}') - \frac{\partial}{\partial Z} h_\epsilon(Z, \bar{\epsilon}) \right| \\
&\leq bC C' \|[Z, s, \bar{\epsilon}]^\top - [Z', s', \bar{\epsilon}']^\top\|,
\end{aligned}$$

for some positive constants  $C, C'$ . Along with (S91) this concludes the proof.  $\square$

**Lemma G.3.** Let  $\mathbf{X} \in \mathbb{R}^{n \times p}$  have i.i.d. entries  $x_{ij} \sim \mathcal{N}(0, n^{-1})$  and let  $\lim_{n \rightarrow \infty} p/n = \kappa \in (0, 1)$ . Then almost surely,  $\|\mathbf{X}\|_2 < \infty$ .

*Proof.* This follows directly from Rudelson and Vershynin 2010, Theorem 2.1.  $\square$

**Lemma G.4.** For  $i = 1, \dots, n$ , let  $\bar{\epsilon}_i$  be i.i.d.  $U(0, 1)$  random variables and  $\boldsymbol{\eta}_{0,i}$  be i.i.d.  $N(0, \gamma^2)$  such that  $\bar{\epsilon}_i \perp \boldsymbol{\eta}_{0,j}$  for  $i, j = 1, \dots, n$ . Further, let

$$y_i^* = \alpha \mathbb{1} \{ \bar{\varepsilon}_i < \zeta'(\boldsymbol{\eta}_{0,i}) \} + \frac{1-\alpha}{2}, \quad \epsilon y_i^* = \alpha \left\{ 1 - \frac{\bar{\varepsilon}_i - \zeta'(\boldsymbol{\eta}_{0,i})}{|\bar{\varepsilon}_i - \zeta'(\boldsymbol{\eta}_{0,i})| + \epsilon} \right\} + \frac{1-\alpha}{2}.$$

Then for  $\mathbf{y}^* = (y_1^*, \dots, y_n^*)$ ,  $\epsilon \mathbf{y}^* = (\epsilon y_1^*, \dots, \epsilon y_n^*)$ ,

$$i) \lim_{n \rightarrow \infty} \frac{1}{p} \|\mathbf{y}^* - \epsilon \mathbf{y}^*\|_2^2 = E[(y_i^* - \epsilon y_i^*)^2] \text{ almost surely,}$$

$$ii) \lim_{\epsilon \rightarrow 0} E[(y_i^* - \epsilon y_i^*)^2] = 0$$

*Proof.* (i) By definition  $\frac{1}{p} \|\mathbf{y}^* - \epsilon \mathbf{y}^*\|_2^2 = \frac{1}{p} \sum_{i=1}^n (y_i^* - \epsilon y_i^*)^2$ . By boundedness of  $y_i^*, \epsilon y_i^*$ ,  $E[(y_i^* - \epsilon y_i^*)^2]$  exists and thus, by the strong law of large numbers (e.g. Vershynin 2018, Theorem 1.3.1), claim (i) follows. (ii) Note that since  $\bar{\varepsilon}_i, \boldsymbol{\eta}_{0,i}$  are continuous independent random variables. Hence the event  $\{\exists i : \bar{\varepsilon}_i = \zeta'(\boldsymbol{\eta}_{0,i})\}$  has measure zero. Hence,  $E[(y_i^* - \epsilon y_i^*)^2] = E[(h(\bar{\varepsilon}_i, \boldsymbol{\eta}_{0,i}) - \epsilon h(\bar{\varepsilon}_i, \boldsymbol{\eta}_{0,i}))^2]$ . The claim now follows from boundedness of  $E[(y_i^* - \epsilon y_i^*)^2]$ , the dominated convergence theorem and Lemma G.1 i).  $\square$

**Lemma G.5.** The map  $f(\boldsymbol{\beta}) = \omega(\|\boldsymbol{\beta}\|_2/\sqrt{n})$  of Lemma 7 in Sur (2019) is such that if  $\lim_{\epsilon \rightarrow 0} \|\boldsymbol{\beta}(\epsilon)\|_2 = r$ , for some sequence  $\boldsymbol{\beta}(\epsilon) \in \mathbb{R}^p$  indexed by  $\epsilon$ , then  $\lim_{\epsilon \rightarrow 0} f(\boldsymbol{\beta}(\epsilon)) = \omega(r/\sqrt{n})$ .

*Proof.* It is readily checked that the function  $\omega(\|\boldsymbol{\beta}\|_2/\sqrt{n})$  is of the form  $c_1 \inf_{z: |z| \leq c_2 \frac{\|\boldsymbol{\beta}\|_2}{\sqrt{n}}} \zeta''(z)$  for some constants  $c_1, c_2 > 0$  that do not depend on  $\boldsymbol{\beta}$ . Now  $\zeta''(z)$  is symmetric and strictly decreasing in  $|z|$  so that  $\inf_{z: |z| \leq c_2 \frac{\|\boldsymbol{\beta}\|_2}{\sqrt{n}}} \zeta''(z) = \zeta''(c_2 \|\boldsymbol{\beta}\|_2/\sqrt{n})$ . The claim follows by taking limits and the continuity of the function  $\zeta''$ .  $\square$

**Lemma G.6.** Consider the system of equations  $F(\mu, b, \sigma, \epsilon) = 0$  given by

$$E \left[ \frac{1}{1 + b \zeta''(\text{prox}_{b\zeta}(b_\epsilon Y^* + Z_*))} \right] - 1 + \kappa = 0 \quad (\text{S92})$$

$$\frac{b}{\kappa \gamma^2} E[Z \{ \epsilon Y^* - \zeta'(\text{prox}_{b\zeta}(b_\epsilon Y^* + Z_*)) \}] = 0 \quad (\text{S93})$$

$$\frac{b^2}{\kappa^2} E[\{ \epsilon Y^* - \zeta'(\text{prox}_{b\zeta}(b_\epsilon Y^* + Z_*)) \}^2] - \sigma^2 = 0, \quad (\text{S94})$$

where  $Z \sim N(0, \gamma^2)$ ,  $G \sim N(0, 1)$ , and  $\bar{\varepsilon} \sim U(0, 1)$ , all independent of each other, and  $\epsilon Y^* = h_\epsilon(Z, \bar{\varepsilon})$ ,  $Z_* = \mu Z + \kappa^{1/2} \sigma G$ .

Assume there exists a solution  $F(\mu_*, b_*, \sigma_*, 0) = 0$  such that the Jacobian with respect to  $(\mu_*, b_*, \sigma_*)$  of  $F(\mu_*, b_*, \sigma_*, 0)$  is nonsingular.

Then, in a neighbourhood around  $(\mu_*, b_*, \sigma_*)$ ,  $\epsilon = 0$ , there exist unique functions  $\epsilon \mu_*, \epsilon b_*, \epsilon \sigma_*$  that are continuous in  $\epsilon$  such that  $F(\epsilon \mu_*, \epsilon b_*, \epsilon \sigma_*, \epsilon) = 0$ .

*Proof.* The claim follows by the Implicit Function Theorem (e.g. Rudin 1976, Theorem 9.28), for which it is required that

- (i) There exists a solution  $F(\mu_*, b_*, \sigma_*, 0)$ ,
- (ii) The Jacobian with respect to  $(\mu_*, b_*, \sigma_*)$  of  $F(\mu_*, b_*, \sigma_*, 0)$  is nonsingular

(iii)  $F(\mu, b, \sigma, \epsilon)$  is continuously differentiable in a neighbourhood around  $(\mu_*, b_*, \sigma_*)$ ,  $\epsilon = 0$

(i) and (ii) are assumed so that it remains to show (iii). Hence, it is sufficient to show that the partial derivatives of (S92)-(S94) exist and are continuous in a neighbourhood around  $(\mu_*, b_*, \sigma_*)$ ,  $\epsilon = 0$ . Begin with (S92) and consider

$$\begin{aligned}
\frac{\partial}{\partial b} \frac{1}{1 + b\zeta''(\text{prox}_{b\zeta}(b_\epsilon Y^* + Z_*))} &= - \frac{1}{[1 + b\zeta''(\text{prox}_{b\zeta}(b_\epsilon Y^* + Z_*))]^2} \frac{\partial}{\partial b} b\zeta''(\text{prox}_{b\zeta}(b_\epsilon Y^* + Z_*)) \\
&= - \frac{1}{[1 + b\zeta''(\text{prox}_{b\zeta}(b_\epsilon Y^* + Z_*))]^2} \left\{ \zeta''(\text{prox}_{b\zeta}(b_\epsilon Y^* + Z_*)) \right. \\
&\quad \left. + b\zeta'''(\text{prox}_{b\zeta}(b_\epsilon Y^* + Z_*)) \left[ \frac{\partial}{\partial u} \text{prox}_{b\zeta}(u) \Big|_{u=b_\epsilon Y^* + Z_*} \frac{\partial}{\partial b} u + \frac{\partial}{\partial b} \text{prox}_{b\zeta}(u) \Big|_{u=b_\epsilon Y^* + Z_*} \right] \right\} \\
&= - \frac{1}{[1 + b\zeta''(\text{prox}_{b\zeta}(b_\epsilon Y^* + Z_*))]^2} \left\{ \zeta''(\text{prox}_{b\zeta}(b_\epsilon Y^* + Z_*)) \right. \\
&\quad \left. + b\zeta'''(\text{prox}_{b\zeta}(b_\epsilon Y^* + Z_*)) \left[ \frac{\epsilon Y^*}{1 + b\zeta''(\text{prox}_{b\zeta}(b_\epsilon Y^* + Z_*))} - \frac{\zeta'(\text{prox}_{b\zeta}(b_\epsilon Y^* + Z_*))}{1 + b\zeta''(\text{prox}_{b\zeta}(b_\epsilon Y^* + Z_*))} \right] \right\} \\
&= - \frac{1}{[1 + b\zeta''(\text{prox}_{b\zeta}(b_\epsilon Y^* + Z_*))]^2} \\
&\quad \cdot \left\{ \zeta''(\text{prox}_{b\zeta}(b_\epsilon Y^* + Z_*)) + \frac{b\zeta'''(\text{prox}_{b\zeta}(b_\epsilon Y^* + Z_*))}{1 + b\zeta''(\text{prox}_{b\zeta}(b_\epsilon Y^* + Z_*))} \left[ \epsilon Y^* - \zeta'(\text{prox}_{b\zeta}(b_\epsilon Y^* + Z_*)) \right] \right\}, \tag{S95}
\end{aligned}$$

where the first and second equality follow by the chain rule and the third uses Proposition A.1 of Donoho and Montanari (2016). Now note that  $\zeta'(x) \in (0, 1)$ ,  $\zeta''(x) \in (0, \frac{1}{4}]$ ,  $\zeta'''(x) \in [-\frac{1}{6\sqrt{3}}, \frac{1}{6\sqrt{3}}]$  and  $\epsilon Y^* \in [\frac{1-\alpha}{2}, \frac{1+\alpha}{2}]$ . Hence (S95) is bounded. Thus, by the Dominated Convergence Theorem and the Mean Value Theorem,

$$\frac{\partial}{\partial b} \mathbb{E} \left[ \frac{1}{1 + b\zeta''(\text{prox}_{b\zeta}(b_\epsilon Y^* + Z_*))} \right] = \mathbb{E} \left[ \frac{\partial}{\partial b} \frac{1}{1 + b\zeta''(\text{prox}_{b\zeta}(b_\epsilon Y^* + Z_*))} \right]. \tag{S96}$$

And again by dominated convergence, (S96) is continuous if (S95) is. By Lemma G.7,  $\text{prox}_{b\zeta}(b_\epsilon Y^* + Z_*)$  is continuous in  $(b, \epsilon Y^*, Z_*)$ . Since  $\epsilon Y^* = \frac{\alpha}{2} \left\{ 1 - \frac{\bar{\epsilon} - \zeta'(Z)}{|\bar{\epsilon} - \zeta'(Z)| + \epsilon} \right\}$  and  $Z_* = \mu Z + \kappa^{1/2} \sigma G$ ,  $\text{prox}_{b\zeta}(b_\epsilon Y^* + Z_*)$  is continuous in  $(\mu, b\sigma, \epsilon)$ . The claim follows by continuity of  $\zeta'(\cdot), \zeta''(\cdot), \zeta'''(\cdot)$  and since (S95) is the composition of continuous functions. The treatment of the other partial derivatives is similar and thus details are omitted.

Next consider,

$$\frac{\partial}{\partial \mu} \frac{1}{1 + b\zeta''(\text{prox}_{b\zeta}(b_\epsilon Y^* + Z_*))} = - \frac{b\zeta'''(\text{prox}_{b\zeta}(b_\epsilon Y^* + Z_*)) Z}{[1 + b\zeta''(\text{prox}_{b\zeta}(b_\epsilon Y^* + Z_*))]^3}, \tag{S97}$$

which is again dominated by an integrable function and thus  $\frac{\partial}{\partial \mu} \mathbb{E} \left[ \frac{1}{1 + b\zeta''(\text{prox}_{b\zeta}(b_\epsilon Y^* + Z_*))} \right]$  is continuous in  $(\mu, b, \sigma, \epsilon)$ .

Similarly,

$$\frac{\partial}{\partial \sigma} \frac{1}{1 + b\zeta''(\text{prox}_{b\zeta}(b_\epsilon Y^* + Z_*))} = - \frac{b\zeta'''(\text{prox}_{b\zeta}(b_\epsilon Y^* + Z_*)) \kappa^{1/2} G}{[1 + b\zeta''(\text{prox}_{b\zeta}(b_\epsilon Y^* + Z_*))]^3},$$

and the same conclusion as for (S97) holds for  $\frac{\partial}{\partial \sigma} \mathbb{E} \left[ \frac{1}{1+b\zeta''(\text{prox}_{b\zeta}(b_\epsilon Y^* + Z_*))} \right]$ .

Finally,

$$\frac{\partial}{\partial \epsilon} \frac{1}{1+b\zeta''(\text{prox}_{b\zeta}(b_\epsilon Y^* + Z_*))} = -\frac{b\zeta'''(\text{prox}_{b\zeta}(b_\epsilon Y^* + Z_*))}{[1+b\zeta''(\text{prox}_{b\zeta}(b_\epsilon Y^* + Z_*))]^3} \frac{\alpha}{2} \frac{\bar{\epsilon} - \zeta'(Z)}{(|\bar{\epsilon} - \zeta'(Z)| + \epsilon)^2}, \quad (\text{S98})$$

which is bounded and continuous in  $(b, \mu, \sigma, \epsilon)$  for  $\bar{\epsilon} \neq \zeta'(Z)$ . Since the event  $\bar{\epsilon} = \zeta'(Z)$ , has measure zero, as  $\bar{\epsilon} \sim U(0, 1)$  and  $Z \sim \mathcal{N}(0, 1)$   $\bar{\epsilon} \perp Z$ , dominated convergence still applies and the claim holds.

Next, consider (S93), and differentiate the integrand with respect to  $b$ ,

$$\begin{aligned} \frac{\partial}{\partial b} \frac{b}{\kappa\gamma^2} Z \{ \epsilon Y^* - \zeta'(\text{prox}_{b\zeta}(b_\epsilon Y^* + Z_*)) \} &= \frac{1}{\kappa\gamma^2} Z \{ \epsilon Y^* - \zeta'(\text{prox}_{b\zeta}(b_\epsilon Y^* + Z_*)) \} \\ &\quad - Z \frac{\zeta''(\text{prox}_{b\zeta}(b_\epsilon Y^* + Z_*))}{1+b\zeta''(\text{prox}_{b\zeta}(b_\epsilon Y^* + Z_*))} \{ \epsilon Y - \zeta'(\text{prox}_{b\zeta}(b_\epsilon Y^* + Z_*)) \}, \end{aligned}$$

of which both terms on the RHS are dominated by an integrable function and which are continuous in  $(\mu, b, \sigma, \epsilon)$ . Thus  $\frac{\partial}{\partial b} \frac{b}{\kappa\gamma^2} \mathbb{E} [Z \{ \epsilon Y^* - \zeta'(\text{prox}_{b\zeta}(b_\epsilon Y^* + Z_*)) \}]$  exists and is continuous in  $(\mu, b, \sigma, \epsilon)$ .

Next, differentiate with respect to  $\mu$  to get

$$\frac{\partial}{\partial \mu} \frac{b}{\kappa\gamma^2} Z \{ \epsilon Y^* - \zeta'(\text{prox}_{b\zeta}(b_\epsilon Y^* + Z_*)) \} = -\frac{b}{\kappa\gamma^2} \frac{Z^2 \zeta''(\text{prox}_{b\zeta}(b_\epsilon Y^* + Z_*))}{1+b\zeta''(\text{prox}_{b\zeta}(b_\epsilon Y^* + Z_*))},$$

which is again dominated by an integrable function and continuous in  $(\mu, b, \sigma, \epsilon)$ , so that

$$\frac{\partial}{\partial \mu} \frac{b}{\kappa\gamma^2} \mathbb{E} [Z \{ \epsilon Y^* - \zeta'(\text{prox}_{b\zeta}(b_\epsilon Y^* + Z_*)) \}]$$

exists and is continuous in  $(\mu, b, \sigma, \epsilon)$ .

Differentiating with respect to  $\sigma$  yields

$$\frac{\partial}{\partial \mu} \frac{b}{\kappa\gamma^2} Z \{ \epsilon Y^* - \zeta'(\text{prox}_{b\zeta}(b_\epsilon Y^* + Z_*)) \} = -\frac{b}{\kappa\gamma^2} \frac{Z \kappa^{1/2} G \zeta''(\text{prox}_{b\zeta}(b_\epsilon Y^* + Z_*))}{1+b\zeta''(\text{prox}_{b\zeta}(b_\epsilon Y^* + Z_*))},$$

and the same conclusion holds for  $\frac{\partial}{\partial \sigma} \frac{b}{\kappa\gamma^2} \mathbb{E} [Z \{ \epsilon Y^* - \zeta'(\text{prox}_{b\zeta}(b_\epsilon Y^* + Z_*)) \}]$ .

Finally, differentiating with respect to  $\epsilon$ ,

$$\frac{\partial}{\partial \mu} \frac{b}{\kappa\gamma^2} Z \{ \epsilon Y^* - \zeta'(\text{prox}_{b\zeta}(b_\epsilon Y^* + Z_*)) \} = -\frac{b}{\kappa\gamma^2} Z \left\{ 1 - \frac{b\zeta''(\text{prox}_{b\zeta}(b_\epsilon Y^* + Z_*))}{1+b\zeta''(\text{prox}_{b\zeta}(b_\epsilon Y^* + Z_*))} \right\} \frac{\alpha}{2} \frac{\bar{\epsilon} - \zeta'(Z)}{(|\bar{\epsilon} - \zeta'(Z)| + \epsilon)^2},$$

and arguing analogous to (S98) yields that  $\frac{\partial}{\partial \epsilon} \frac{b}{\kappa\gamma^2} \mathbb{E} [Z \{ \epsilon Y^* - \zeta'(\text{prox}_{b\zeta}(b_\epsilon Y^* + Z_*)) \}]$  exists and is continuous in  $(\mu, b, \sigma, \epsilon)$ .

Lastly, the same is repeated for (S94).

$$\begin{aligned} \frac{\partial}{\partial b} \frac{b^2}{\kappa^2} \{ \epsilon Y^* - \zeta'(\text{prox}_{b\zeta}(b_\epsilon Y^* + Z_*)) \}^2 - \sigma^2 &= \frac{2b}{\kappa^2} \{ \epsilon Y^* - \zeta'(\text{prox}_{b\zeta}(b_\epsilon Y^* + Z_*)) \}^2 - 1 \\ &\quad - \frac{2b^2}{\kappa^2} \{ \epsilon Y^* - \zeta'(\text{prox}_{b\zeta}(b_\epsilon Y^* + Z_*)) \} \frac{\zeta''(\text{prox}_{b\zeta}(b_\epsilon Y^* + Z_*))}{1+b\zeta''(\text{prox}_{b\zeta}(b_\epsilon Y^* + Z_*))} \\ &\quad \cdot \{ \epsilon Y^* - \zeta'(\text{prox}_{b\zeta}(b_\epsilon Y^* + Z_*)) \}, \end{aligned}$$

$$\frac{\partial}{\partial \mu} \frac{b^2}{\kappa^2} \{ \epsilon Y^* - \zeta'(\text{prox}_{b\zeta}(b_\epsilon Y^* + Z_*)) \}^2 - \sigma^2 = -\frac{2b^2}{\kappa^2} \{ \epsilon Y^* - \zeta'(\text{prox}_{b\zeta}(b_\epsilon Y^* + Z_*)) \} \frac{Z \zeta''(\text{prox}_{b\zeta}(b_\epsilon Y^* + Z_*))}{1+b\zeta''(\text{prox}_{b\zeta}(b_\epsilon Y^* + Z_*))},$$

$$\frac{\partial}{\partial \sigma} \frac{b^2}{\kappa^2} \left\{ \epsilon Y^* - \zeta'(\text{prox}_{b\zeta}(b_\epsilon Y^* + Z_*)) \right\}^2 - \sigma^2 = -\frac{2b^2}{\kappa^2} \left\{ \epsilon Y^* - \zeta'(\text{prox}_{b\zeta}(b_\epsilon Y^* + Z_*)) \right\} \frac{\kappa^{1/2} G\zeta''(\text{prox}_{b\zeta}(b_\epsilon Y^* + Z_*))}{1 + b\zeta''(\text{prox}_{b\zeta}(b_\epsilon Y^* + Z_*))} - 2\sigma,$$

$$\frac{\partial}{\partial \epsilon} \frac{b^2}{\kappa^2} \left\{ \epsilon Y^* - \zeta'(\text{prox}_{b\zeta}(b_\epsilon Y^* + Z_*)) \right\}^2 - \sigma^2 = -\frac{2b^2}{\kappa^2} \left\{ \epsilon Y^* - \zeta'(\text{prox}_{b\zeta}(b_\epsilon Y^* + Z_*)) \right\} \cdot \frac{1}{1 + b\zeta''(\text{prox}_{b\zeta}(b_\epsilon Y^* + Z_*))} \frac{\alpha}{2} \frac{\bar{\epsilon} - \zeta'(Z)}{(|\bar{\epsilon} - \zeta'(Z)| + \epsilon)^2},$$

all of which are dominated by some integrable function and continuous almost everywhere. Thus, again by dominated convergence, all partial derivatives of  $\frac{b^2}{\kappa^2} \mathbb{E} \left[ \left\{ \epsilon Y^* - \zeta'(\text{prox}_{b\zeta}(b_\epsilon Y^* + Z_*)) \right\}^2 \right] - \sigma^2$  exist and are continuous. Thus,  $F(\mu, b, \sigma, \epsilon)$  is continuously differentiable in a neighbourhood around  $(\mu_*, b_*, \sigma, 0)$  and the Implicit Function Theorem establishes the claim of the Lemma.  $\square$

**Lemma G.7.** *The proximal operator  $\text{prox}_{b\zeta}(by + z)$  is continuous in  $(b, y, z)$  for  $b > 0$ ,  $x, y \in \mathbb{R}$  where  $\zeta(x) = \log(1 + e^x)$ .*

*Proof.* Recall that by definition of the proximal operator,

$$\text{prox}_{b\zeta}(by + z) = \arg \min_{u \in \mathbb{R}} \left\{ b\zeta(u) + \frac{1}{2}(u - [by + z])^2 \right\},$$

and since  $\zeta(\cdot)$  is differentiable and strictly convex, it is uniquely determined as the solution to the first order condition

$$b\zeta'(u) + u - by - z = 0.$$

Now note that  $F(u, b, y, z) = b\zeta'(u) + u - by - z$  is continuously differentiable in  $(u, b, y, z)$  and that  $\frac{\partial}{\partial u} F(u, b, y, z) = b\zeta''(u) + 1 > 0$  for all  $(u, b, y, z)$ . Hence, by the Implicit Function Theorem (e.g. Rudin 1976, Theorem 9.28), there exists a unique function  $u(b', y', z')$  in a neighbourhood around  $(b, y, z)$  that is continuous in its arguments such that  $F(u(b', y', z'), b', y', z') = 0$ . Hence, the proximal operator is continuous in a neighbourhood around  $(b, y, z)$ . Since the choice of  $(b, y, z)$  was arbitrary, it is continuous over its entire domain.  $\square$

**Lemma G.8.** *In the setting of Corollary B.2.1 and assuming that a stationary solution  $(\epsilon\mu_*, \epsilon b_*, \epsilon\sigma_*)$  to the state evolution (S37)-(S38) exists, the AMP iterates of (S39) and (S40) satisfy the Cauchy property*

$$\lim_{t \rightarrow \infty} \lim_{N \rightarrow \infty} \frac{1}{p} \left\| \epsilon \boldsymbol{\nu}^{t+1} - \epsilon \boldsymbol{\nu}^t \right\|_2^2 = 0$$

$$\lim_{t \rightarrow \infty} \lim_{N \rightarrow \infty} \frac{1}{n} \left\| \epsilon \mathbf{R}^{t+1} - \epsilon \mathbf{R}^t \right\|_2^2 = 0$$

*almost surely.*

*Proof.* The proof is a direct translation of the Lemmas 6.8-6.9 of Donoho and Montanari (2016) along the lines suggested by Sur and Candès 2019 in the proof of Theorem 7 of the supplementary material. In particular, isolating iterates  $\epsilon \boldsymbol{\nu}^{t-1}, \epsilon \boldsymbol{\nu}^t$  in Theorem B.2, similar arguments to those in

Corollary B.2.1 yield that, almost surely

$$\lim_{N \rightarrow \infty} \frac{1}{p} \sum_{j=1}^p \psi \left( \begin{bmatrix} \epsilon \boldsymbol{\nu}_j^{t-1} \\ \epsilon \boldsymbol{\nu}_j^t \end{bmatrix}, \begin{bmatrix} 0 \\ 0 \end{bmatrix} \right) = \mathbb{E} \left[ \psi \left( \begin{bmatrix} \mathbf{Z}_t^{2t} \\ \mathbf{Z}_{t-1}^{2t} \end{bmatrix}, \begin{bmatrix} 0 \\ 0 \end{bmatrix} \right) \right], \quad \begin{bmatrix} \mathbf{Z}_{t-1}^{2t} \\ \mathbf{Z}_t^{2t} \end{bmatrix} \sim N \left( \mathbf{0}_2, \begin{bmatrix} \epsilon \tau_{t-1}^2 & \epsilon \rho_{t-1,t} \\ \epsilon \rho_{t-1,t} & \epsilon \tau_t^2 \end{bmatrix} \right)$$

where

$$\begin{aligned} \epsilon \tau_t^2 &= \kappa^{-2} \mathbb{E} [\{\Psi^{t-1}(h_\epsilon(\mathbf{Z}_1^{2t-1}, \bar{\epsilon}), \mathbf{Z}_2^{2t-1})\}^2] \\ \epsilon \rho_{t-1,t} &= \kappa^{-2} \mathbb{E} [\Psi^{t-1}(h_\epsilon(\mathbf{Z}_1^{2t-1}, \bar{\epsilon}), \mathbf{Z}_{t+1}^{2t-1}) \Psi^{t-2}(h_\epsilon(\mathbf{Z}_1^{2t-1}, \bar{\epsilon}), \mathbf{Z}_t^{2t-1})], \end{aligned}$$

which in turn have covariance structure according to the state evolution (S8)-(S9). Now recall that given the covariance structure derived in Corollary B.2.1, it was argued that given initial conditions  $\hat{\beta}^0$ ,

$$\begin{aligned} \epsilon \mu_0 &= \frac{1}{\gamma^2} \lim_{n \rightarrow \infty} \frac{\langle \hat{\beta}^0, \beta_0 \rangle}{n} \\ \epsilon \sigma_0^2 &= \lim_{n \rightarrow \infty} \frac{\|\hat{\beta}^0 - \mu_0 \beta_0\|_2^2}{p}, \end{aligned} \tag{S99}$$

for all  $t$ ,  $\epsilon \tau_t = \epsilon \sigma_t$ . Now, given a stationary solutions  $(\epsilon \mu_*, \epsilon b_{*\epsilon}, \sigma_*)$  to the state evolutions (S36)-(S38), choose the oracle initialiser  $\hat{\beta}^0 = \epsilon \mu_* \beta_0 + \epsilon \sigma_* \boldsymbol{\xi}$ , where  $\boldsymbol{\xi} \sim N(\mathbf{0}_p, \mathbf{I}_p)$  which is independent of  $\beta_0$ . Then the initial conditions of (S99) are

$$\begin{aligned} \epsilon \mu_0 &= \frac{1}{\gamma^2} \lim_{n \rightarrow \infty} \frac{\langle \epsilon \mu_* \beta_0 + \epsilon \sigma_* \boldsymbol{\xi}, \beta_0 \rangle}{n} \stackrel{a.s.}{=} \epsilon \mu_* \\ \epsilon \sigma_0^2 &= \lim_{n \rightarrow \infty} \frac{\|\epsilon \sigma_* \boldsymbol{\xi}\|_2^2}{p} \stackrel{a.s.}{=} \epsilon \sigma_*^2. \end{aligned}$$

Henceforth condition on the event that  $\epsilon \mu_0 = \epsilon \mu_*$ ,  $\epsilon \sigma_0^2 = \epsilon \sigma_*^2$ . Then  $\epsilon \tau_{t-1}^2 = \epsilon \tau_t^2 = \epsilon \sigma_*^2$  and letting  $\psi(\mathbf{u}, \mathbf{v}) = (\mathbf{u}_1 - \mathbf{u}_2)^2$ , for  $\mathbf{u} = [\mathbf{u}_1, \mathbf{u}_2]^\top$ , one gets that almost surely,

$$\lim_{N \rightarrow \infty} \frac{1}{p} \|\epsilon \boldsymbol{\nu}^t - \epsilon \boldsymbol{\nu}^{t-1}\|_2^2 = 2(\epsilon \sigma_*^2 - \epsilon \rho_{t,t-1}).$$

Hence, the goal is to show that  $\lim_{t \rightarrow \infty} \epsilon \rho_{t,t-1} = \epsilon \sigma_*^2$ .

Towards that end, following the proof of Theorem 4.1 of Donoho and Montanari (2016), define the doubly infinite matrix  $\boldsymbol{\Gamma} = \{\Gamma_{s,t}\}_{s,t \in \mathbb{N}_0}$  with entries

$$\Gamma_{s+1,t+1} = \frac{1}{\kappa^2} \mathbb{E} [\Psi^*(h_\epsilon(Z, \bar{\epsilon}), \epsilon Z_s) \Psi^*(h_\epsilon(Z, \bar{\epsilon}), \epsilon Z_t)]$$

where  $\Psi^*(y, s) = \epsilon b_* (y - \zeta'(\text{prox}_{\epsilon b_* \zeta}(\epsilon b_* y + s)))$  and

$$\begin{aligned} \epsilon Z_s &= \epsilon \mu_* Z + \kappa^{1/2} \epsilon \tilde{G}_s, & \begin{bmatrix} \epsilon \tilde{G}_s \\ \epsilon \tilde{G}_t \end{bmatrix} &\sim N \left( \mathbf{0}_2, \begin{bmatrix} \epsilon \sigma_*^2 & \Gamma_{s,t} \\ \Gamma_{s,t} & \epsilon \sigma_*^2 \end{bmatrix} \right), \\ \epsilon Z_t &= \epsilon \mu_* Z + \kappa^{1/2} \epsilon \tilde{G}_t, \end{aligned}$$

where  $Z \sim N(0, \gamma^2)$ ,  $\bar{\epsilon}$ , are all pairwise independent and independent of  $\tilde{G}_s, \tilde{G}_t$ . Further, take the boundary conditions  $\Gamma_{0,0} = \epsilon \sigma_*^2$ ,  $\Gamma_{t,0} = \Gamma_{0,t} = 0$  so that in particular  $\Gamma_{t,t} = \epsilon \sigma_*^2$ .

It is then readily verified that for all  $t, s$ ,  $\Gamma_{t,s} = \epsilon \rho_{t,s}$ . Next, let  $q_t = \Gamma_{t+1,t} / \epsilon \sigma_*^2$ . Then  $q_t$  is governed by the recursion

$$\begin{aligned} q_{t+1} &= H(q_t) \\ H(q) &= \frac{1}{\kappa^2 \epsilon \sigma_*^2} \mathbb{E} [\Psi^*(h_\epsilon(Z, \bar{\epsilon}), \epsilon Z_1) \Psi^*(h_\epsilon(Z, \bar{\epsilon}), \epsilon Z_2)], \end{aligned}$$

with

$$\begin{aligned} \epsilon Z_1 &= \epsilon \mu_* Z + \kappa^{1/2} \epsilon \sigma_* G_1 \\ \epsilon Z_2 &= \epsilon \mu_* Z + \kappa^{1/2} \epsilon \sigma_* G_2 \end{aligned} \quad \begin{bmatrix} G_1 \\ G_2 \end{bmatrix} \sim N \left( \mathbf{0}_2, \begin{bmatrix} 1 & q \\ q & 1 \end{bmatrix} \right) \perp Z \sim N(0, \gamma^2).$$

Next, it is proven that:

- i)  $H(1) = 1$
- ii)  $H(q)$  is increasing for  $q \in [0, 1]$ ,
- iii)  $H(q)$  is strictly convex for  $q \in [0, 1]$

Towards i) note that

$$H(1) = \frac{1}{\kappa^2 \epsilon \sigma_*^2} \mathbb{E} \left[ \Psi^* (h_\epsilon(Z, \bar{\epsilon}), \epsilon Z_1)^2 \right],$$

for  $\epsilon Z_1 = \epsilon \mu_* Z + \kappa^{1/2} \epsilon \sigma_* G$ ,  $G \sim N(0, 1) \perp Z$ . Thus  $H(1) = 1$  since (S38) holds for  $(\epsilon \mu_*, \epsilon b_*, \epsilon \sigma_*)$ .

Next, given  $\bar{\epsilon}, Z$ , let  $g_{Z, \bar{\epsilon}}(G) = \Psi^*(h_\epsilon(Z, \bar{\epsilon}), \epsilon \mu_* Z + \kappa^{1/2} \epsilon \sigma_* G)$  and let

$$\mathcal{H}(q) = \mathbb{E} \left[ g_{Z, \bar{\epsilon}}(G_1) g_{Z, \bar{\epsilon}}(G_2) \middle| \bar{\epsilon}, Z \right], \quad \begin{bmatrix} G_1 \\ G_2 \end{bmatrix} \sim N \left( \mathbf{0}_2, \begin{bmatrix} 1 & q \\ q & 1 \end{bmatrix} \right). \quad (\text{S100})$$

Then, by linearity of expectations and the tower property, it is sufficient to show that  $\mathcal{H}(q)$  satisfies ii) and iii).

Following the argument in Donoho and Montanari 2016, Lemma 6.9, let  $\{X_t\}_{t \geq 0}$  be the stationary Ornstein-Uhlenbeck process with covariance  $\mathbb{E}(X_0 X_t) = e^{-t}$ . Then

$$\mathcal{H}(q) = \mathbb{E} [g_{Z, \bar{\epsilon}}(G_1) g_{Z, \bar{\epsilon}}(G_2)] \Big|_{t=\log(1/q)},$$

where the expectation is taken with respect to the process  $\{X_t\}_{t \geq 0}$ . Then by the spectral representation for  $t = \log(1/q)$ ,

$$\mathcal{H}(q) = \sum_{l=1}^{\infty} c_l^2 e^{-lt} = \sum_{l=1}^{\infty} c_l^2 q_l,$$

and the claim follows since  $c_l \neq 0$  at least once for  $g_{Z, \bar{\epsilon}}$  nonlinear.

Hence, it follows that  $\lim_{t \rightarrow \infty} q_t = 1$  if and only if  $H'(1) \leq 1$ .

Further, it holds that

$$H'(1) = \frac{1}{\kappa} \mathbb{E} \left[ \left\{ \frac{\partial}{\partial s} \Psi^*(h_\epsilon(\bar{\epsilon}, Z), \epsilon Z_1) \right\}^2 \right].$$

Indeed, again condition on  $\bar{\epsilon}, Z$  and consider  $\frac{\partial}{\partial q} \mathcal{H}(q)$  as defined in (S100). For notational convenience, the conditioning in the expectation of  $\mathcal{H}$  is suppressed below and  $g_{Z, \bar{\epsilon}}(G)$  is simply denoted by  $g(G)$ .

Then, since  $G_2$  can be written as  $qG_1 + \sqrt{1-q^2}\tilde{G}$  for  $\tilde{G} \sim N(0, 1)$  is independent of all other

random variables, it holds that

$$\begin{aligned}
\frac{\partial}{\partial q} \mathcal{H}(q) &= \frac{\partial}{\partial q} \mathbb{E}[g(G_1)g(G_2)] \\
&= \mathbb{E} \left[ \frac{\partial}{\partial q} g(G_1)g(G_2) \right] \\
&= \mathbb{E} \left[ \frac{\partial}{\partial q} g(G_1)g(qG_1 + \sqrt{1-q^2}\tilde{G}) \right] \\
&= \mathbb{E} \left[ g(G_1)g'(qG_1 + \sqrt{1-q^2}\tilde{G})\kappa^{1/2}_\epsilon \sigma_* \left\{ G_1 - \frac{q}{\sqrt{1-q^2}}\tilde{G} \right\} \right] \\
&= \mathbb{E} \left[ g(G_1)g'(qG_1 + \sqrt{1-q^2}\tilde{G})\kappa^{1/2}_\epsilon \sigma_* G_1 \right] - \frac{q}{\sqrt{1-q^2}} \mathbb{E} \left[ g(G_1)g'(qG_1 + \sqrt{1-q^2}\tilde{G})\kappa^{1/2}_\epsilon \sigma_* \tilde{G} \right], \tag{S101}
\end{aligned}$$

where the second inequality follows by dominated convergence. Now let  $F(G_1, G_2) = g(G_1)g'(G_2)$ . Then note that  $\frac{\partial}{\partial G_1} F(G_1, G_2) = \kappa^{1/2}_\epsilon \sigma_* g'(G_1)g'(G_2)$  and  $\frac{\partial}{\partial G_2} F(G_1, G_2) = \kappa^{1/2}_\epsilon \sigma_* g(G_1)g''(G_2)$ . Hence, using Gaussian integration by parts, which can be derived as a consequence of Stein's Lemma (Stein, 1981, Lemma 1),

$$\begin{aligned}
\mathbb{E} \left[ g(G_1)g'(qG_1 + \sqrt{1-q^2}\tilde{G})\kappa^{1/2}_\epsilon \sigma_* G_1 \right] &= \mathbb{E} \left[ g(G_1)g'(G_2)\kappa^{1/2}_\epsilon \sigma_* G_1 \right] \\
&= \kappa^{1/2}_\epsilon \sigma_* \mathbb{E} [G_1 F(G_1, G_2)] \\
&= \kappa^{1/2}_\epsilon \sigma_* \left\{ \text{cov}(G_1, G_1) \mathbb{E} \left[ \frac{\partial}{\partial G_1} F(G_1, G_2) \right] \right. \\
&\quad \left. + \text{cov}(G_1, G_2) \mathbb{E} \left[ \frac{\partial}{\partial G_2} F(G_1, G_2) \right] \right\} \\
&= \kappa_\epsilon \sigma_*^2 \left\{ \mathbb{E} \left[ \frac{\partial}{\partial G_1} F(G_1, G_2) \right] + q \mathbb{E} \left[ \frac{\partial}{\partial G_2} F(G_1, G_2) \right] \right\} \\
&= \kappa_\epsilon \sigma_*^2 \left\{ \mathbb{E} [g'(G_1)g'(G_2)] + q \mathbb{E} \left[ \frac{\partial}{\partial G_2} g(G_1)g''(G_2) \right] \right\}.
\end{aligned}$$

Similarly,

$$\begin{aligned}
\mathbb{E} \left[ g(G_1)g'(qG_1 + \sqrt{1-q^2}\tilde{G})\kappa^{1/2}_\epsilon \sigma_* \tilde{G} \right] &= \kappa^{1/2}_\epsilon \sigma_* \mathbb{E} [F(G_1, qG_1 + \sqrt{1-q^2}\tilde{G})\tilde{G}] \\
&= \kappa^{1/2}_\epsilon \sigma_* \left\{ \text{cov}(G_1, \tilde{G}) \mathbb{E} \left[ \frac{\partial}{\partial G_1} F(G_1, qG_1 + \sqrt{1-q^2}\tilde{G}) \right] \right. \\
&\quad \left. + \text{cov}(\tilde{G}, \tilde{G}) \mathbb{E} \left[ \frac{\partial}{\partial \tilde{G}} F(G_1, qG_1 + \sqrt{1-q^2}\tilde{G}) \right] \right\} \\
&= \sqrt{1-q^2} \kappa_\epsilon \sigma_*^2 \mathbb{E} [g(G_1)g''(qG_1 + \sqrt{1-q^2}\tilde{G})] \\
&= \sqrt{1-q^2} \kappa_\epsilon \sigma_*^2 \mathbb{E} [g(G_1)g''(G_2)], \tag{S102}
\end{aligned}$$

where it was used that  $\text{cov}(G_1, \tilde{G}) = 0$ . Thus combining (S101)-(S102), it follows that

$$\frac{\partial}{\partial q} \mathcal{H}(q) = \kappa_\epsilon \sigma_*^2 \mathbb{E} [g'(G_1)g'(G_2)].$$

Marginalizing over  $Z, \bar{\varepsilon}$  then gives

$$\begin{aligned}
\frac{\partial}{\partial q} H(q) &= \frac{1}{\kappa^2 \epsilon \sigma_*^2} \frac{\partial}{\partial q} \mathbb{E}_{Z, \bar{\varepsilon}} \left[ \mathbb{E} \left[ g(G_1) g(G_2) \middle| Z, \bar{\varepsilon} \right] \right] \\
&= \frac{1}{\kappa^2 \epsilon \sigma_*^2} \mathbb{E}_{Z, \bar{\varepsilon}} \left[ \mathbb{E} \left[ \frac{\partial}{\partial q} g(G_1) g(G_2) \middle| Z, \bar{\varepsilon} \right] \right] \\
&= \frac{1}{\kappa} \mathbb{E}_{Z, \bar{\varepsilon}} \left[ \mathbb{E} \left[ g'(G_1) g'(G_2) \middle| Z, \bar{\varepsilon} \right] \right] \\
&= \frac{1}{\kappa} \mathbb{E} [g'(G_1) g'(G_2)] \\
&= \frac{1}{\kappa} \mathbb{E} \left[ g'(G_1) g'(qG_1 + \sqrt{1-q^2} \tilde{G}) \right],
\end{aligned}$$

and it thus follows that  $H'(1) = \frac{1}{\kappa} \mathbb{E} \left[ \left\{ \frac{\partial}{\partial s} \Psi^*(h_\epsilon(\bar{\varepsilon}, Z), \epsilon Z_1) \right\}^2 \right]$  as required.

Now it is easily checked that  $\frac{\partial}{\partial s} \Psi^* \in (0, 1)$  and thus

$$H'(1) = \frac{1}{\kappa} \mathbb{E} \left[ \left\{ \frac{\partial}{\partial s} \Psi^*(h_\epsilon(\bar{\varepsilon}, Z), \epsilon Z_1) \right\}^2 \right] \leq \frac{1}{\kappa} \mathbb{E} \left[ \frac{\partial}{\partial s} \Psi^*(h_\epsilon(\bar{\varepsilon}, Z), \epsilon Z_1) \right] = 1$$

since (S36) holds. Similar arguments show the Cauchy-property for  $\frac{1}{n} \|\epsilon \mathbf{R}^t - \epsilon \mathbf{R}^{t-1}\|_2^2$ .  $\square$

**Lemma G.9.** *The solution to the system of equations (S3)-(S5) is equivalent to the stationary solution of (S16)-(S18)*

*Proof.* Begin by imposing stationarity for equations (S16)-(S18), so that they become

$$\begin{aligned}
1 - \kappa &= \mathbb{E} \left[ \frac{1}{1 + b_* \zeta''(\text{prox}_{b_* \zeta}(b_* Y^* + Z_*))} \right] \\
0 &= \frac{b_*}{\kappa \gamma^2} \mathbb{E} [Z \{Y^* - \zeta'(\text{prox}_{b_* \zeta}(b_* Y^* + Z_*))\}] \\
\sigma_*^2 &= \frac{b_*^2}{\kappa^2} \mathbb{E} [\{Y^* - \zeta'(\text{prox}_{b_* \zeta}(b_* Y^* + Z_*))\}^2],
\end{aligned}$$

for independent  $Z \sim N(0, \gamma^2)$ ,  $G \sim N(0, 1)$ , and  $\bar{\varepsilon} \sim U(0, 1)$ , and  $Y^* = \alpha \mathbf{1}\{\bar{\varepsilon} \leq \zeta'(Z)\} + \frac{1-\alpha}{2}$ ,  $Z_* = \mu_* Z + \kappa^{1/2} \sigma_* G$ . Hence

$$\begin{aligned}
\mathbb{E} \left[ \frac{1}{1 + b_* \zeta''(\text{prox}_{b_* \zeta}(b_* Y^* + Z_*))} \right] &= \mathbb{E} \left[ \frac{\zeta'(Z)}{1 + b_* \zeta''(\text{prox}_{b_* \zeta}(b_* \frac{1+\alpha}{2} + Z_*))} \right] + \mathbb{E} \left[ \frac{\zeta'(-Z)}{1 + b_* \zeta''(\text{prox}_{b_* \zeta}(b_* \frac{1-\alpha}{2} + Z_*))} \right] \\
&= \mathbb{E} \left[ \frac{\zeta'(Z)}{1 + b_* \zeta''(\text{prox}_{b_* \zeta}(b_* \frac{1+\alpha}{2} + Z_*))} \right] + \mathbb{E} \left[ \frac{\zeta'(-Z)}{1 + b_* \zeta''(-\text{prox}_{b_* \zeta}(b_* \frac{1-\alpha}{2} + Z_*))} \right] \\
&= \mathbb{E} \left[ \frac{\zeta'(Z)}{1 + b_* \zeta''(\text{prox}_{b_* \zeta}(b_* \frac{1+\alpha}{2} + Z_*))} \right] + \mathbb{E} \left[ \frac{\zeta'(-Z)}{1 + b_* \zeta''(\text{prox}_{b_* \zeta}(b_* \frac{1+\alpha}{2} - Z_*))} \right] \\
&= 2 \mathbb{E} \left[ \frac{\zeta'(Z)}{1 + b_* \zeta''(\text{prox}_{b_* \zeta}(b_* \frac{1+\alpha}{2} + Z_*))} \right],
\end{aligned}$$

where the first equality follows by conditioning on  $Y^*$ , the second follows since  $\zeta''(x) = \zeta''(-x)$ ,

the fourth since  $-\text{prox}_{b\zeta}(-u) = \text{prox}_{b\zeta}(u+b)$  (cf. p.18 in the supplementary material of Sur and Candès (2019)), which holds since the proximal operator  $x^* = \text{prox}_{b\zeta}(-u)$  is the unique solution to  $b\zeta'(x^*) + x^* + u = 0$  and similarly  $y^* = \text{prox}_{b\zeta}(u+b)$  is the unique solution to  $b\zeta'(y^*) + y^* - u - b = 0$ . Hence, by substitution and using that  $\zeta'(-x) = 1 - \zeta'(x)$ ,  $y^*$  is the unique solution to  $b(\zeta'(y) - \zeta'(-x^*)) + y^* - x = 0$  so that  $y^* = -x^*$ . Therefore, letting  $-u = b_*(1 - \alpha)/2 + Z_*$ ,  $u + b_* = b_*(1 + \alpha)/2 - Z_*$  as required. The last equality follows by a simple change of variable and the symmetry of the normal distribution.

Similarly,

$$\begin{aligned}
\mathbb{E} [Z \{Y^* - \zeta'(\text{prox}_{b_*\zeta}(b_*Y^* + Z_*))\}] &= \mathbb{E} \left[ \zeta'(Z) Z \left\{ \frac{1+\alpha}{2} - \zeta' \left( \text{prox}_{b_*\zeta} \left( b_* \frac{1+\alpha}{2} + Z_* \right) \right) \right\} \right] \\
&+ \mathbb{E} \left[ \zeta'(-Z) Z \left\{ \frac{1-\alpha}{2} - \zeta' \left( \text{prox}_{b_*\zeta} \left( b_* \frac{1-\alpha}{2} + Z_* \right) \right) \right\} \right] \\
&= \mathbb{E} \left[ \zeta'(Z) Z \left\{ \frac{1+\alpha}{2} - \zeta' \left( \text{prox}_{b_*\zeta} \left( b_* \frac{1+\alpha}{2} + Z_* \right) \right) \right\} \right] \\
&+ \mathbb{E} \left[ \zeta'(-Z) Z \left\{ \frac{1-\alpha}{2} - \left( 1 - \zeta' \left( -\text{prox}_{b_*\zeta} \left( b_* \frac{1-\alpha}{2} + Z_* \right) \right) \right) \right\} \right] \\
&= \mathbb{E} \left[ \zeta'(Z) Z \left\{ \frac{1+\alpha}{2} - \zeta' \left( \text{prox}_{b_*\zeta} \left( b_* \frac{1+\alpha}{2} + Z_* \right) \right) \right\} \right] \\
&- \mathbb{E} \left[ \zeta'(-Z) Z \left\{ \frac{1+\alpha}{2} - \zeta' \left( \text{prox}_{b_*\zeta} \left( b_* \frac{1+\alpha}{2} - Z_* \right) \right) \right\} \right] \\
&= 2\mathbb{E} \left[ \zeta'(Z) Z \left\{ \frac{1+\alpha}{2} - \zeta' \left( \text{prox}_{b_*\zeta} \left( b_* \frac{1+\alpha}{2} + Z_* \right) \right) \right\} \right],
\end{aligned}$$

where again, the first equality comes from conditioning on  $Y^*$ , the second, from  $\zeta'(-x) = 1 - \zeta'(x)$ , the third by the symmetry of the proximal operator around  $b$ , i.e.  $-\text{prox}_{b\zeta}(-u) = \text{prox}_{b\zeta}(u+b)$ , and the last by change of variable and symmetry of the normal distribution.

And finally,

$$\begin{aligned}
\mathbb{E} [\{Y^* - \zeta'(\text{prox}_{b_*\zeta}(b_*Y^* + Z_*))\}^2] &= \mathbb{E} \left[ \zeta'(Z) \left\{ \frac{1+\alpha}{2} - \zeta' \left( \text{prox}_{b_*\zeta} \left( b_* \frac{1+\alpha}{2} + Z_* \right) \right) \right\}^2 \right] \\
&+ \mathbb{E} \left[ \zeta'(-Z) \left\{ \frac{1-\alpha}{2} - \zeta' \left( \text{prox}_{b_*\zeta} \left( b_* \frac{1-\alpha}{2} + Z_* \right) \right) \right\}^2 \right] \\
&= \mathbb{E} \left[ \zeta'(Z) \left\{ \frac{1+\alpha}{2} - \zeta' \left( \text{prox}_{b_*\zeta} \left( b_* \frac{1+\alpha}{2} + Z_* \right) \right) \right\}^2 \right] \\
&+ \mathbb{E} \left[ \zeta'(-Z) \left\{ \frac{1+\alpha}{2} - \zeta' \left( -\text{prox}_{b_*\zeta} \left( b_* \frac{1-\alpha}{2} + Z_* \right) \right) \right\}^2 \right] \\
&= \mathbb{E} \left[ \zeta'(Z) \left\{ \frac{1+\alpha}{2} - \zeta' \left( \text{prox}_{b_*\zeta} \left( b_* \frac{1+\alpha}{2} + Z_* \right) \right) \right\}^2 \right] \\
&+ \mathbb{E} \left[ \zeta'(-Z) \left\{ \frac{1+\alpha}{2} - \zeta' \left( \text{prox}_{b_*\zeta} \left( b_* \frac{1+\alpha}{2} - Z_* \right) \right) \right\}^2 \right] \\
&= 2\mathbb{E} \left[ \zeta'(Z) \left\{ \frac{1+\alpha}{2} - \zeta' \left( \text{prox}_{b_*\zeta} \left( b_* \frac{1+\alpha}{2} + Z_* \right) \right) \right\}^2 \right].
\end{aligned}$$

□

**Lemma G.10.** Let  $\mathbf{u} \in \mathbb{R}^p$  be a unit vector and  $\mathbf{P}_{\mathbf{u}^\perp} = \mathbf{I}_p - \mathbf{u}\mathbf{u}^\top$  be the projection into the subspace  $\mathbf{u}^\perp$  that is orthogonal to  $\mathbf{u}$ . Then for  $\mathbf{Z} \sim \mathcal{N}(\mathbf{0}_p, \mathbf{I}_p)$ , almost surely,

$$\lim_{p \rightarrow \infty} \frac{\|\mathbf{P}_{\mathbf{u}^\perp} \mathbf{Z}\|_2}{\sqrt{p}} = 1,$$

as  $p \rightarrow \infty$ .

*Proof.* Consider  $\|\mathbf{P}_{\mathbf{u}^\perp} \mathbf{Z}\|_2^2 = \mathbf{Z}^\top \mathbf{P}_{\mathbf{u}^\perp} \mathbf{Z}$  since  $\mathbf{P}_{\mathbf{u}^\perp}$  is idempotent and note that  $\text{tr}(\mathbf{P}_{\mathbf{u}^\perp}) = p - 1$ . By the Hanson-Wright inequality (e.g. Vershynin (2018, Theorem 6.2.1)), there exists a universal constant  $c > 0$  such that for any  $\epsilon \in (0, 1)$ ,

$$\Pr \left( \left| \frac{\mathbf{Z}^\top \mathbf{P}_{\mathbf{u}^\perp} \mathbf{Z}}{p - 1} - 1 \right| > \epsilon \right) \leq 2 \exp \{ -c\epsilon^2(p - 1) \}.$$

Now since for  $\delta > 0$ ,  $|z - 1| \geq \delta$  implies that  $|z^2 - 1| \geq \max\{\delta, \delta^2\}$  (see Vershynin (2018, Equation 3.2)), one gets that

$$\Pr \left( \left| \frac{\|\mathbf{P}_{\mathbf{u}^\perp} \mathbf{Z}\|_2}{\sqrt{p - 1}} - 1 \right| > \epsilon \right) \leq 2 \exp \{ -c\epsilon^2(p - 1) \}.$$

By the first Borel-Cantelli Lemma, it follows that  $\lim_{p \rightarrow \infty} \|\mathbf{P}_{\mathbf{u}^\perp} \mathbf{Z}\|_2 / (p - 1) = 1$  almost surely and the claim follows.  $\square$

## References

- Beck A (2017). *First-order methods in optimization*. SIAM. ISBN 978-1-61197-498-0. doi:10.1137/1.9781611974997.
- Candès EJ, Sur P (2020). “The phase transition for the existence of the maximum likelihood estimate in high-dimensional logistic regression.” *The Annals of Statistics*, **48**(1), 27–42. doi:10.1214/18-AOS1789.
- Diaconis P, Ylvisaker D (1979). “Conjugate priors for exponential families.” *The Annals of Statistics*, **7**(2), 269–281. doi:10.1214/aos/1176344611.
- Donoho D, Montanari A (2016). “High dimensional robust M-estimation: Asymptotic variance via approximate message passing.” *Probability Theory and Related Fields*, **166**, 935–969. doi:10.1007/s00440-015-0675-z.
- Feng OY, Venkataramanan R, Rush C, Samworth RJ (2022). “A unifying tutorial on approximate message passing.” *Foundations and Trends in Machine Learning*, **15**(4), 335–536. doi:10.1561/22000000092.
- Javanmard A, Montanari A (2013). “State evolution for general approximate message passing algorithms, with applications to spatial coupling.” *Information and Inference: A Journal of the IMA*, **2**(2), 115–144. doi:10.1093/imaiai/iat004.
- Magnus JR, Neudecker H (2019). *Matrix Differential Calculus with Applications in Statistics and Econometrics*. John Wiley & Sons. ISBN 9781119541202. doi:10.1002/9781119541219.
- Rudelson M, Vershynin R (2010). *Non-asymptotic theory of random matrices: Extreme singular values*, pp. 1576–1602. doi:10.1142/9789814324359\_0111.
- Rudin W (1976). *Principles of Mathematical Analysis*. McGraw-hill New York, 3rd edition. ISBN 978-0070542358.
- Shiryaev AN (2016). *Probability-1*, volume 95. Springer. ISBN 978-1-4939-7905-9. doi:10.1007/978-0-387-72206-1.

- Stein CM (1981). “Estimation of the mean of a multivariate normal distribution.” *The Annals of Statistics*, **9**(6), 1135–1151. doi:10.1214/aos/1176345632.
- Sur P (2019). *A Modern Maximum Likelihood Theory for High-dimensional Logistic Regression*. Ph.D. thesis, Stanford University. URL <http://purl.stanford.edu/jw604jq1260>.
- Sur P, Candès EJ (2019). “A modern maximum-likelihood theory for high-dimensional logistic regression.” *Proceedings of the National Academy of Sciences*, **116**(29), 14516–14525. doi:10.1073/pnas.1810420116.
- Sur P, Chen Y, Candès EJ (2019). “The likelihood ratio test in high-dimensional logistic regression is asymptotically a rescaled chi-square.” *Probability theory and related fields*, **175**, 487–558. doi:10.1007/s00440-018-00896-9.
- Vershynin R (2018). *High-dimensional Probability: An Introduction with Applications in Data Science*, volume 47. Cambridge university press.
- Zehna PW (1966). “Invariance of maximum likelihood estimators.” *The Annals of Mathematical Statistics*, **37**(3), 744–744. doi:10.1214/aoms/1177699475.
- Zhao Q, Sur P, Candès EJ (2022). “The asymptotic distribution of the MLE in high-dimensional logistic models: Arbitrary covariance.” *Bernoulli*, **28**(3), 1835–1861. doi:10.3150/21-BEJ1401.
